# Supplementary material for: Repairing Regressors for Fair Binary Classification at Any Decision Threshold
Source: arXiv:2203.07490 source file (2023-12-10)
Supplement: Supplementary file 1 [file junk.tex]

where the last equality in the above line follows from Leibniz Rule. Straightf-orward computation of the derivative of $V_\tau(\cdot)$ shows  
\begin{align*}
    \partialdd{}{\lambda}V_\tau(\pi_{\pa,\lambda})  = V^{'}_{\tau}(\pi_{\pa,\lambda})(T_\pa^* - \id) 
\end{align*}



\begin{align*}
    \partialdd{}{\lambda}V_\tau(\pi_{\protp,\frac{1-\lambda}{p_\pa} + \lambda})
\end{align*}
\begin{align*}
    = \left(\frac{p_\pa-1}{p_\pa}\right)V^{'}_{\tau}(\pi_{\protp,\frac{1-\lambda}{p_\pa} + \lambda})\id - \left(\frac{1-p_\pa }{p_\pa}\right)V^{'}_{\tau}(\pi_{\protp,\frac{1-\lambda}{p_\pa} + \lambda})T_\protp^* , 
\end{align*}
\noindent indicating that the derivative we're after is nothing more than
