# Supplementary material for: Repairing Regressors for Fair Binary Classification at Any Decision Threshold
Source: arXiv:2203.07490 source file (2023-12-10)
Supplement: Supplementary file 2 [file 00_appendix.tex]

\newpage
\appendix
\onecolumn


\input{sections/old_appendix/10_sdp}

\input{sections/old_appendix/20_ot}

\input{sections/old_appendix/30_proofs}

\input{sections/old_appendix/40_algorithm}

\input{sections/old_appendix/50_empirical}
