# Supplementary material for: Repairing Regressors for Fair Binary Classification at Any Decision Threshold
Source: arXiv:2203.07490 source file (2023-12-10)
Supplement: Supplementary file 3 [file 10_sdp.tex]

% \section{Strong Demographic Parity}

% While notably proven~\citet{jiang2020wasserstein}, we provide our own proof of Strong Definition Parity (SDP), which we discuss as the special case of Distributional Parity (Definition \ref{def:distributionalparity}) for which $\gamma=\PR$. First, we formally, we define SDP as follows:

% \begin{definition}
% \label{def:sdp}
% Recall that $\ospace \subseteq \binaryrange$ is a closed subset denoting probabilities. Let $U(\Omega)$ be a uniform distribution over $\ospace$. For positive rate metric $\PR$, \textit{strong demographic parity} for a regressor $f$ is satisfied when
% \begin{align*}
%     \mathcal{S}(f) \triangleq  \Expect_{\tau \sim U(\ospace)}| \PR_{\pa}(\tau) - \PR_{\protp}(\tau) | = 0,
% \end{align*}
% where $\mu_\pa$ and $\mu_\protp$ are measures that group-specific measures that satisfy Assumption~\ref{assumption:wass}. 
% \end{definition}

% Definition~\ref{def:sdp} is equivalent to Equation~\ref{eq:wass_e}, with the added condition that parity occurs when the Wasserstein distance $\Wass_{1}(\mu_\pa,\mu_\protp) = 0$. 
