# Supplementary material for: Repairing Regressors for Fair Binary Classification at Any Decision Threshold
Source: arXiv:2203.07490 source file (2023-12-10)
Supplement: Supplementary file 4 [file 20_ot.tex]

\section{Additional Background on Optimal Transport}
In this section of the Appendix, we provide additional details for topics we could not fit into the main body of the paper. For readers familiar with Optimal Transport, much of the below material will not be new; nevertheless, we encourage all readers to use these sections as reference as they see fit. 

\textbf{Additional Notation}. Let $O = \ospace \times Y \times \Prot$.  We define our probability measures w.r.t. a probability space $(O, \mathcal F, \mathbb P)$ where $\mathcal{F}$ is a $\sigma-$algebra on $O$.  $\mathbb P$ is the measure associated with the full joint distribution, and as defined above, $\mu$ are the measures for the underlying associated marginal distributions. 

The $\id$ function is shorthand for the identity function, i.e, $\id:\ospace \rightarrow \ospace$ and $\id(s) = s$ for $s \in \Omega$.  Additionally we denote the push-forward operator as $f\#\mu$ (see \citet{ComputationalOptimalTransport}, Remark 2.5) where $f$ is a measurable function pushing mass from a measure $\mu$. 

We also include the following remark, as we make use of it in the proof of Theorem 1 (Section \ref{app:proofs:thm1}). 
\begin{remark}
\label{rem:continuous_monotone_T}
If $\mu_\pa, \mu_\protp$ are non-atomic, then $T_\pa^\protp$ is continuous and non-decreasing (see \citet[p.55]{santambrogio2015optimal} where $T\#\mu_{\pa} = \mu_\protp$. 
\end{remark}
\subsection{Barycenters}
\label{sec:barycenters}
In general, and as stated above, Wasserstein-1 barycenters are defined as the solution to the following minimization problem:  
\begin{definition}
For two measures $\mu_\pa,\mu_\protp \in \Pm(\ospace)$, their $\lambda$-weighted \textit{Wasserstein-1 barycenter} is 
\begin{align*}
\mu_{\lambda} \leftarrow \argmin_{\mu' \in \Pm(\ospace)}  (1-\lambda)\Wass_1(\mu_\pa, \mu')  + \lambda\Wass_1(\mu_\protp, \mu');
\end{align*}
\end{definition}
As shown in \citet[Thm 5.28]{santambrogio2015optimal}, when Assumption \ref{assumption:wass} is satisfied, these measures satisfy a relatively simple closed form:
\begin{align}
\label{eq:barycenter_pushfoward}
    \mu_\lambda = ((1-\lambda)\id + \lambda T_a^b) \# \mu_a.
\end{align}
In cases where we explicitly state that some barycenter-like-interpolation begins at a group-specific $\mu$, we will include the group in the subscript, e.g., $\mu_{\pa,\lambda} = ((1-\lambda)\id + \lambda T_a^b) \# \mu_a$.

Additionally, we include the following proposition which reveals a convenient property of barycenters that we make use of in the proof of Theorem $\ref{thm:convex}$ (Appendix~\ref{app:proofs:thm1}):
\begin{proposition}
\label{prop:mcann} (Proposition 1.3 from  \citet{mccanInterpolation})  Let $\mu_\pa, \mu_\protp \in \Pm(\ospace)$ satisfy Assumption \ref{assumption:wass} and let $\mu_\lambda$ be the barycenter of $\mu_a$ and $\mu_b$.  Then $\mu_{\pa,\lambda} = \mu_{\protp,1-\lambda}$ and $\mu_{\protp,\lambda} = \mu_{\pa,1-\lambda}$. 
\end{proposition}


Next, we introduce a result from prior work that show that the set of barycenters $\{\mu_\lambda\}_{\lambda \in \binaryrange}$ admit a linear-like geometric structure in the space of probability measures, much like the linear interpolation performed in Equation (\ref{eq:barycenter_pushfoward}). To clarify this result, we first introduce two new terms: Wasserstein Spaces, and (Wasserstein) Geodesics. First:

\begin{definition}
\label{def:w-space}
The Wasserstein-1 Space is the set of distributions $\Pm(\ospace)$ endowed with the $\Wass_1$ metric.  
\end{definition}

In other words, the Wasserstein-1 Space is exactly a metric space over probability measures with finite first order moments, where the Wasserstein-1 distance is the chosen metric between them.  To this end, it is well-known that the Wasserstein Distance satisfies the properties of a metric \cite{ComputationalOptimalTransport}, e.g, the triangle inequality. 

Second, we introduce geodesics. Informally, in a metric space, a geodesic is the shortest path between two points. Formally:


\begin{definition} 
\label{def:geodesic}
Let $\lambda_1,\lambda_2 \in \binaryrange$. A curve $\eta:\binaryrange \rightarrow \Pm(\ospace)$ is a geodesic\footnote{Most precisely, this is the definition for a constant-speed geodesic, however we ignore this imprecision for clarity.} in $\Wass_{1}(\ospace)$ if 
\begin{align*}
    \Wass_1(\eta(\lambda_1),\eta(\lambda_2)) = |\lambda_2-\lambda_1|\Wass_1(\eta(0), \eta(1))
\end{align*}
\end{definition}

Geodesics are useful for making our informal, intuitive understanding of barycenters more precise. So far, we have described a barycenter as the least-expensive composition of two probability measures. We can alternatively understand this ``least-expensive'' intuition in precise geometric terms --- i.e., as a geodesic.

Using Definitions~\ref{def:w-space} and~\ref{def:geodesic}, we state the following theorem: 

\begin{theorem}
\label{thm:geodesic}
(Theorem 5.27 from \citet{santambrogio2015optimal})  Suppose that $\ospace$ is a convex set. Let $\mu_a,\mu_\protp \in \Pm(\ospace)$ satisfy Assumption \ref{assumption:wass}. If $T_\pa^\protp$ is an optimal transport plan from $\mu_\pa$ to $\mu_\protp$ then the set of barycenters between these distributions is exactly the curve $\mu_\lambda = ((1-\lambda)\id + \lambda T_\pa^\protp)\#\mu_\pa$, which is a geodesic in $\Wass_{1}(\ospace)$. 
\end{theorem}

Informally, this theorem states that interpolation along $\lambda$-barycenters produces a geodesic in $\Wass_1(\ospace)$  

It is important to note that, in general, the Wasserstein-1 space is not convex \citep{wassProjection}; however,  we can exploit the geometry of geodesics to make special-case convexity claims.  

\subsection{Connecting Barycenters and Geometric Repair}
\label{sec:connecting_barycenters}

Recall from the definition of geometric repair that we can define a repaired regressor $f_\lambda$ as 
\begin{align*}
    f_{\lambda}(x,\prot) \triangleq (1-\lambda)f(x,\prot) + \lambda \fsdp(x,\prot),  
\end{align*}
where $\lambda \in \binaryrange$ is the repair parameter and $\fsdp(x,g) = T_\prot^*(f(x,\prot))$. Given that $f(x,\prot)$ is the original score, and $\fsdp(x,\prot)= T_\prot^*(f(x,\prot))$ is the transformed score, we can we equivalently define geometric repair as
\begin{align*}
    f_{\lambda}(x,\prot) = ((1-\lambda)\id + \lambda T_\prot^*) \circ f(x,\prot) 
\end{align*}
If we we use the geometric repair definition to push-forward $\mu_g$, the measure by which the scores for group $\prot$ are distributed, then we obtain the measure(s) which govern $f_\lambda$  
\begin{align}
\label{eq: repair_law}
   ((1-\lambda)\id + \lambda T_\prot^*) \# \mu_\prot = Law(f_\lambda(\Xrv,\prot)),
\end{align}
for which we denote $Law(f_\lambda(\Xrv,\prot))$ as $\mu_{\prot,\lambda}$. From this equality we can draw a connection between wasserstein barycenters and geometric repair -- ultimately showing that as we vary the repair parameter, we are actually interpolating between each group's score distribution and the SDP barycenter distribution $\mu_*$. 

\textbf{Which $\lambda$ is Which?} So far, we've introduced two styles of notation to discuss the interpolation of measures via barycenters, they are $\mu_\lambda$, and $\mu_{\prot,\lambda}$. To disambiguate their difference, consider the following:  
\begin{enumerate}
    \item $\mu_\lambda$  denotes $\lambda$-weighted barycenters in a general context, and is not specific to geometric repair.  Recall the formula for $\mu_\lambda$, which is based on our general-case formula for barycenters (see Section \ref{sec:barycenters} and Equation (\ref{eq:barycenter_pushfoward}))
    \begin{align*}
         \mu_\lambda = ((1-\lambda)\id + \lambda T_a^b) \# \mu_a
    \end{align*}
    In the above, we omit groups from the subscript because we tend to emphasize the transportation is happening \emph{from} $\mu_a$ \emph{to} $\mu_b$.  
    
    \item  $\mu_{\prot,\lambda}$ denotes the interpolation of some group's conditional distribution toward its $p_\pa$-barycenter, denoted $\mu_*$ (recall this is the SDP solution by Equation (\ref{eq:sdp_barycenter})) as a result of geometric repair, i.e., 
    \begin{align}
    \label{eq: mu_group_lambda}
        \mu_{\prot,\lambda} = ((1-\lambda)\id + \lambda T_\prot^*) \# \mu_\prot. 
    \end{align}
    Under geometric repair, \textit{each} group's distribution is moving toward the barycenter, so the difference between group $\pa$'s $\lambda$-repaired distribution, and group $\protp$'s $\lambda$-repaired distribution, is significant -- hence the additional notation. 
 \end{enumerate}

With this in mind, we revisit Proposition $\ref{prop:mcann}$ in the context of geometric, and introduce the following Lemma, which we use in the proof of Theorem $\ref{thm:convex}$.
\begin{lemma}
\label{lemma: subsitution_help}
Let $\mu_\pa, \mu_\protp \in \Pm(\ospace)$ satisfy Assumption \ref{assumption:wass} and let $\mu_{\pa,\lambda}$ be the $\lambda$-barycenter of $\mu_a$ and $\mu_*$, and let $\mu_{\protp,\lambda}$ be the $\lambda$-barycenter of $\mu_\protp$ and $\mu_*$ then 
\begin{align*}
    \mu_{\pa,\lambda} &= \mu_{\protp, \frac{1-p_\pa\lambda}{1-p_\pa}} \\ 
    \mu_{\protp, \lambda} &= \mu_{\pa, \frac{1-\lambda}{p_\pa} + \lambda}
\end{align*}
\begin{proof}
Recall by Equations (\ref{eq: mu_group_lambda}) and (\ref{eq:barycenter_pushfoward})  that $\mu_{\pa,\lambda} = \mu_{\lambda(1-p_\pa)}$.  Similarly, $\mu_{\protp,t} = \mu_{1-t p_\pa}$.  To prove the Lemma, we need some $\lambda$ s.t. $\lambda = t$, such that $\lambda$ becomes geometric repair parameter for both groups. Letting $\lambda(1-p_\pa) = 1-t p_\pa$ and solving for $\lambda$, yields the proposition, i.e., $\lambda = \frac{1- t p_\pa}{1-p_\pa}$ and therefore $\mu_{\pa,\lambda} = \mu_{\protp, \frac{1-p_\pa\lambda}{1-p_\pa}}$. The second equivalence follows symmetrically, by swapping $t$ and $\lambda$. 



% Let $\lambda = t(1-p_\pa)$ for $t \in \binaryrange$. If we recall that $T_\pa^*$ maps group $a$ to the $p_\pa$-weighted barycenter, then it easily follows from Equations \TODO{number them} that
% \begin{align*}
%     \mu_{t(1-p_\pa)} = ((1-t(1-p_\pa))\id +  t(1-p_\pa) T_a^b) \# \mu_a = ((1-\lambda)\id + \lambda T_\pa^*) \# \mu_\pa = \mu_{\pa, \lambda}
% \end{align*}

% By similar reasoning $\mu_{1-p_\pa t} = \mu_{\protp, \lambda} $. Setting $\lambda(1-p_\pa) = 1-p_{\pa}t$, solving for $\lambda$, and simplifying the expression yields the desired statement. 
\end{proof}
\end{lemma}




\subsubsection{Fairness Metrics as Functionals}
\label{sec:fairness_metrics_functionals}
In general, we can view fairness metrics as a functionals over the space of probabilities.  Specifically, the fairness metrics we consider in this work can be written as a ``potential energy'' functional and are defined by the integral of a given function taken over some measure.
\begin{definition}[Potential Energy]
\label{def:potential_energy}
The potential energy of a function $V:\ospace \rightarrow \reals{}$ over some measure $\mu \in \Pm(\ospace)$ is defined 
\begin{align}
\mathcal{V}(\mu) = \int_{\ospace}Vd\mu. 
\end{align}
\end{definition}

To  express fairness metrics as a potential energy functional we need: the indicator function, a threshold, and the some group conditioned score measure.  For example, we can re-write the positive rate for group $\prot$ as 
\begin{align}
     \PR_{\prot}(\tau) = \Expect_{s \sim \Scorerv}[\mathds{1}_{s \geq \tau}|\Protrv=\prot] &= \int_{\ospace}  \mathds{1}_{s \geq \tau} d\mu_\prot.  
\end{align}
where the last equality follows by definition of conditional expectation.  Similarly, we could express $\gamma \in \{\TPR,\FPR\}$
\begin{align}
\label{eq:gamma_functional}
      \gamma_{\prot}(\tau) = \Expect_{s \sim \Scorerv}[\mathds{1}_{s \geq \tau}|\Protrv=\prot, \Yrv] &= \int_{\ospace}  \mathds{1}_{s \geq \tau} d\mu_{\prot|Y}.  
\end{align}

\subsubsection{Displacement Convexity}

Conceptually, displacement convexity describes the phenomena that some functional on probability measures is convex as one interpolates between two distributions, along their barycenters -- recall that these barycenters form a geodesic (Theorem \ref{thm:geodesic}).  Since the interpolation of score distributions via geometric repair produces a Wasserstein geodesic, displacement convexity is a tool well suited to help us characterize the convexity of fairness metrics under geometric repair. 

\begin{definition}
\label{sec: displacement_convex}
(Definition 7.2 from \citet{agueh2011barycenters})A functional $\mathcal{V}: \Pm(\Omega) \rightarrow \binaryrange$ is said to be displacement convex if the mapping $\lambda \mapsto \mathcal{V}(\mu_\lambda)$ is convex where $\mu_\lambda = ((1-\lambda)\id + \lambda T_\pa^\protp)\#\mu$ is a geodesic between any $\mu_\pa,\mu_\protp \in \Pm(\ospace)$ that satisfy Assumption \ref{assumption:wass}. 
\end{definition}


The following theorem provides a necessary and sufficient condition to determine if potential energy functional is displacement convex. Unsurprisingly, the displacement convexity of the functional $\mathcal{V}$ rests entirely on the convexity of the function $V$ that it integrates over.  

\begin{theorem}
\label{thm:v_convexity}
(Proposition 7.25 from \citet{santambrogio2015optimal} and Proposition 7.7 from \citep{agueh2011barycenters}) The functional $\mathcal{V}$ is displacement convex iff $V$ is convex. 
\end{theorem}

In the case of fairness metrics, the function $V$ is the indicator function over a score $s \in \ospace$ at some $\tau$ i.e. $\mathds{1}_{[s \geq 1]}$.  In general, the indicator function is convex, when the set it is indicating is also convex set \cite{fremond2017collisions}.  Clearly, $[\tau, 1]$ is a convex set, making the indicator function a convex function in our setting.  From this, we can easily establish that $\gamma(\cdot)$ by Equation ($\ref{eq:gamma_functional}$). 
