# Supplementary material for: Repairing Regressors for Fair Binary Classification at Any Decision Threshold
Source: arXiv:2203.07490 source file (2023-12-10)
Supplement: Supplementary file 5 [file 30_proofs.tex]

\section{Proofs}

% In this appendix, we provide complete proofs of Propositions~\ref{rem:risk_bounds} and~\ref{prop:rank_preserving}, as well as fill in comprehensive details for our proof sketch of Theorem~\ref{thm:convex} and Corollary~\ref{cor:additive}. These results concern maximizing distributional parity (Definition~\ref{def:distributionalparity}) using geometric repair (Definition~\ref{def:geometricrepair}).

\subsection{Proof of Proposition~\ref{rem:risk_bounds}}

Recall that Proposition~\ref{rem:risk_bounds} claims that geometric repair (Definition~\ref{def:geometricrepair}) is performance-preserving. In Section~\ref{sec:geometric_repair}, we informally define performance preservation to mean that parity is maximized while minimally impacting empirical risk. 

Formally, we suppose that we want to bound the performance of  $f_\lambda$ under a risk minimization framework like~\citet{chzhen2022minimax, legouic2020projection}. If we define risk as $\mathcal{R}_1(f_\lambda) \triangleq \|f-f_\lambda\|_{1} $, then the following  relationship between the risk of $f_\lambda$ and $\fsdp$ holds: 

\textbf{Proposition~\ref{rem:risk_bounds},} For any $f_{\lambda}$,  $\mathcal{R}_1(f_{\lambda}) \leq \mathcal{R}_1(\fsdp$). More specifically, 
% \begin{align*}
    $\mathcal{R}_1(f_{\lambda}) = \lambda\mathcal{R}_1(\fsdp),  \forall \lambda \in \binaryrange$.
% \end{align*}

\begin{proof}
By definition $\mathcal{R}_1(f_{\lambda}) = \|f - f_\lambda \| = \|f - (f + \lambda(\fsdp - f))\| = \lambda\|f-\fsdp \| = \lambda\mathcal{R}_1(\fsdp)$.  The claimed inequality easily follows. 
\end{proof}

We note that this result for the $\ell_1$ norm is directly related to those that appear in \citet{chzhen2022minimax, legouic2020projection} for the $\ell_2$ norm. 

\subsection{Proof of Proposition~\ref{prop:rank_preserving}}

Recall that Proposition~\ref{prop:rank_preserving} claims that geometric repair (Definition~\ref{def:geometricrepair}) is rank-preserving. In Section~\ref{sec:geometric_repair}, we informally define rank preservation to mean that the repaired regressor $f_\lambda$ never changes the percentiles of scores induced by the original, unrepaired $f$. This entails a property called rational ordering, introduced in \citet[p. 6]{lipton2018rationalordering}, which informally means that ``within each group, individuals with higher probability of belonging to the positive class are always assigned to the positive class ahead of those with lower probabilities.'' Formally,

\textbf{Proposition~\ref{prop:rank_preserving}.} 
Any $\f_\lambda$ is rank preserving and therefore satisfies rational ordering. That is, for any $\lambda \in \binaryrange$, $\tau \in \ospace$, and $(x_1,g_1), (x_2,g_2)$ then

\vspace{-.2cm}
\begin{align*}
    \text{if} &\quad  f(x_1,\prot_1) \leq f(x_2, \prot_2),  \\ 
    \text{then} &\quad  f_{\lambda}(x_1,\prot_1) \leq f_{\lambda}(x_2, \prot_2).
\end{align*}
\begin{proof}
As shown in Section \ref{sec:connecting_barycenters} we can write $f_\lambda$ as $ f_{\lambda}(x,\prot) = ((1-\lambda)\id + \lambda T_\prot^*) \circ f(x,\prot)$. However, the sum $(1-\lambda)\id + \lambda T_\prot^*$ is non-decreasing since it is the sum of non-decreasing $T_{\prot}^*$ (Remark \ref{rem:continuous_monotone_T}) and $\id$ (by Definition).  Since $f_\lambda$ is non-decreasing, we can conclude the proof. 
\end{proof}
% \TODO{note about relationship to prior work}

\subsection{Proof of Theorem~\ref{thm:convex}}\label{app:proofs:thm1}

% Our main result in Section~\ref{sec:geometric_repair} is to show that distributional parity (Definition~\ref{def:distributionalparity}) is convex in the set of $\f_\lambda$-repaired regressors, where in this context convexity implies the existence of some optimal $f_{\lambda_*}$. Given that  $f_{\lambda_*}$ exists, we can find the repair parameter $\lambda_*$ that achieves the repaired $f_{\lambda_*}$ that maximizes distributional parity (within the set of $\f_\lambda$-repaired regressors). \TODO{should we say more about this constrained space?}.


\textbf{Theorem~\ref{thm:convex}.} Recall $\UF_{\gamma}$ denotes distributional parity (Definition~\ref{def:distributionalparity}). Fix $\gamma \in \Gamma$, and let $f$ be a regressor and $f_\lambda$ be this regressor under geometric repair (Definition~\ref{def:geometricrepair}) for any $\lambda \in \binaryrange$. The map $\lambda \mapsto \UF_{\gamma}(\f_\lambda)$ is convex in $\lambda$. That is, if $\lambda_*$ satisfies 

\vspace{-.5cm}
\begin{align*}
    \lambda_* \leftarrow \argmin_{\lambda \in \binaryrange} \UF_{\gamma}(\f_\lambda),
\end{align*}
\vspace{-.2cm}

then $f_{\lambda_{*}}$ is the distributional-parity-maximizing regressor in the set of repaired regressors. 

% \textit{Proof Sketch.}
% \begin{step}
% \label{step:1}
% For some $f$ and its group-conditional score distributions $\mu_\pa,\mu_\protp$, we draw an equivalence between geometric repair and the $\lambda$-barycenters of  $\mu_\pa,\mu_\protp$. By varying $\lambda$,  $\mu_\pa$ and $\mu_\protp$ both individually shift towards $\mu_*$, i.e.,  $\mu_{\prot, \lambda} \triangleq Law(f_\lambda(\Xrv, \prot))$. \textbf{See Section \ref{sec:barycenters} and the end of Section \ref{sec:connecting_barycenters}}.
% \end{step}
% \vspace{.25cm}

% \begin{step}
% \label{step:2}
% We examine the output of $f_\lambda$ as the $\lambda$-barycenter of group-conditional score distributions. This allows us to use tools that characterize convexity in the barycenter space to determine the convexity of distributional parity in $f_\lambda$. \textbf{See beginning of Section \ref{sec:connecting_barycenters}}
% \end{step}
% \vspace{.25cm}

% \begin{step}
% \label{step:3}
% We introduce displacement convexity~\citep{mccanInterpolation}, which is used to describe a functional on probability measures $\mc V: \Pm(\ospace) \rightarrow \binaryrange$ that is convex on a set of barycenters. In our case, this set of barycenters is (wlog) $\{\mu_{\pa, \lambda}\}_{\lambda \in \binaryrange}$. \textbf{See Section \ref{sec: displacement_convex} \footnote{Note, we do not specifically make use of displacement convexity in the result below, however we feel that the result is of independent interest and provides helpful intuition for Step \ref{step:5}.}}.
% \end{step}
% \vspace{.25cm}

% \begin{step}
% \label{step:4}
% We prove that all $\gamma$ can be written as displacement convex functionals. \textbf{See Section \ref{sec:fairness_metrics_functionals}.}
% \end{step}
% \vspace{.25cm}

% \begin{step}
% \label{step:5}
% Finally, we prove that $\lambda \mapsto \UF_{\gamma}(\f_\lambda)$ is convex in $\lambda$. \textbf{See Below.}$\qed$ 
% \end{step}
% \vspace{.25cm}

\begin{proof}
Let $\gamma \in \Gamma$. To prove convexity, we show that  $\frac{d^2}{d\lambda^2}\UF_\gamma(f_\lambda)$ is non-negative everywhere. First, we remind readers the definition of $\UF_\gamma(f_\lambda)$ (distributional parity): 
\begin{align*}
     \mathcal{U}_\gamma(f_\lambda) \triangleq \Expect_{\tau \sim U(\ospace)}| \gamma_{\pa}(\tau) - \gamma_{\protp}(\tau) |. 
\end{align*}
where $\gamma_\prot$ is a fairness metric on the score distributions of $f_\lambda$ for group $\prot \in \Prot$.  

To compute this derivative, we will first compute the derivative of $\gamma_{\pa}(\tau) - \gamma_{\protp}(\tau)$, and then use this to compute the derivative of the $\Expect_{\tau \sim U(\ospace)}| \gamma_{\pa}(\tau) - \gamma_{\protp}(\tau)|$. 

First, we analyze the derivative(s) of $\gamma_\pa$ (wlog). As stated in Section \ref{sec:fairness_metrics_functionals}, we can express $\gamma_\pa$ as a potential energy functional (see Definition \ref{def:potential_energy}) of some repaired group-conditional score measure $\mu_{\prot, \lambda}$. Let $V_\tau(s) := \mathds{1}_{s \geq \tau}$ where $s \in \ospace$. Then $\gamma_\pa$ is defined (see Equation \ref{eq:gamma_functional}) 
\begin{align*}
    \gamma_\pa(\tau) = \int_{\ospace} V_\tau d \mu_{a|\Yrv, \lambda} 
\end{align*}
where $\mu_{a|Y, \lambda}$ is $\mu_{a,\lambda}$ further conditioned on $\Yrv$.  As we proceed, we suppress the $\Yrv$ from the notation, instead writing $\mu_{a, \lambda}$; however, the reader should keep in mind that this result is general, and that this suppression is for brevity and will not affect the computations that follow.  

By Theorem \ref{thm:geodesic}, $\{\mu_{\pa,\lambda}\}_{\lambda \in \binaryrange}$ is a geodesic. Therefore, we can rewrite any $\mu_{\pa,\lambda}$ as $\mu_{\pa,\lambda} \coloneqq ((1-\lambda)id + \lambda T_a^*) \# \mu_a$. Recall $T_\pa^*$ is the optimal transport plan from $\mu_\pa$ to the $p_\pa$-weighted barycenter $\mu_*$ As one final notational convenience, we use $\pi_{\prot,\lambda}$ to denote $(1-\lambda)id + \lambda T_\prot^*$.  We'll first utilize this notation for the group $\pa$ case. Using these substitutions, we have (wlog) that $\mu_{\pa,\lambda} \coloneqq (\pi_{\pa,\lambda}) \# \mu_\pa$, so $\gamma_\pa$ can be equivalently written  
\begin{align*}
    \gamma_\pa(\tau) = \int_{\ospace} V_\tau d(\pi_{\pa,\lambda}\#\mu_\pa). 
\end{align*}

Next we'll apply several change of variables in order to write the above integral w.r.t the Lebesgue measure.  The first change of variables follows by definition of the push-forward operator 
\begin{align*}
    \gamma_\pa(\tau) = \int_{\pi_{\pa,\lambda}^{-1}(\ospace)} V_\tau(\pi_{\pa,\lambda}) d\mu_\pa =  \int_{\ospace} V_\tau(\pi_{\pa,\lambda}) d\mu_\pa. 
\end{align*}
We use the following argument to reason why the domain of integration is unchanged after the reader: by Remark, \ref{rem:continuous_monotone_T} that $T$ is continuous and non-decreasing.  Over a closed domain $\id$ is also continuous and non-decreasing.  Thus, their sum, $\pi_\lambda$ must a bijective function (since it is continuous and monotone on a closed domain). Since $\pi_{\prot,\lambda}$ is a bijective mapping from $\ospace \rightarrow \ospace$, it follows that  $\pi_{\prot, \lambda}^{-1}(\ospace) = \ospace$.  

Next, we use absolutely continuity to re-write the above in terms of $\ell$, i.e, by Assumption \ref{assumption:wass} $\mu_a$ is absolutely continuous with respect to $\ell$ meaning that by the Radon Nikodym-Theorem
\begin{align*}
     \gamma_\pa(\tau) =  \int_{\ospace} V_\tau(\pi_{\prot,\lambda}) d\mu_\pa = \int_{\ospace} \rho_{\mu_\pa}V_\tau(\pi_{\prot,\lambda}) d\ell
\end{align*}
where $\rho_{\mu_\pa}$ is the Radon Nikodym Derivative, i.e., the probability density function associated with $\mu_\pa$. 
This wraps up our definition $\gamma_\pa$.  We'll also need to define this $\protp \in \Prot$.  To do this, we invoke Lemma \ref{lemma: subsitution_help}, i.e., $\mu_{\protp,\lambda} = \mu_{\pa, \frac{1-\lambda}{p_\pa} + \lambda}$. With this in mind, we can write the following, which symmetrically follows from the argument above for the $\mu_\pa$ case:
\begin{align*}
    \gamma_\protp(\tau) = \int_{\ospace} \rho_{\mu_\pa}V_\tau(\pi_{\protp, \frac{1-\lambda}{p_\pa} + \lambda}) d\ell 
\end{align*}
Next, let $h_{\pa,\tau}(\lambda)$ be the mapping $\lambda \mapsto \mathcal V_\tau(\mu_{\pa,\lambda})$ and $h_{\protp,\tau}(\lambda)$ be defined similarly as $\lambda \mapsto \mathcal V_\tau(\mu_{\pa, \frac{1-\lambda}{p_\pa} + \lambda})$.  Then, the difference $h_{\pa,\tau}(\lambda) -h_{\protp,\tau}(\lambda)$ is simply $\gamma_\pa(\tau) - \gamma_\protp(\tau)$ for $f_\lambda$.  We take the derivative of this difference, i.e., 
\begin{dmath*}
    \partialdd{}{\lambda} [h_{\pa,\tau}(\lambda) - h_{\protp,\tau}(
    \lambda)] =  \partialdd{}{\lambda} \int_{\ospace} \rho_{\mu_\pa}\cdot [V_\tau(\pi_{\pa,\lambda}) - V_\tau(\pi_{\protp,\frac{1-\lambda}{p_\pa} + \lambda})] d\ell = \int_{\ospace} \rho_{\mu_\pa}\cdot\left[\partialdd{}{\lambda}\left(V_\tau(\pi_{\pa,\lambda}) - V_\tau(\pi_{\protp,\frac{1-\lambda}{p_\pa} + \lambda})\right)\right] d\ell 
\end{dmath*}
where the last equality in the above line follows from Leibniz Rule. Straightf-orward computation of the derivative of $V_\tau(\cdot)$ shows  
\begin{align*}
    \partialdd{}{\lambda}V_\tau(\pi_{\pa,\lambda})  = V^{'}_{\tau}(\pi_{\pa,\lambda})(T_\pa^* - \id) 
\end{align*}

\noindent and

\begin{align*}
    \partialdd{}{\lambda}V_\tau(\pi_{\protp,\frac{1-\lambda}{p_\pa} + \lambda})
\end{align*}
\begin{align*}
    = \left(\frac{p_\pa-1}{p_\pa}\right)V^{'}_{\tau}(\pi_{\protp,\frac{1-\lambda}{p_\pa} + \lambda})\id - \left(\frac{1-p_\pa }{p_\pa}\right)V^{'}_{\tau}(\pi_{\protp,\frac{1-\lambda}{p_\pa} + \lambda})T_\protp^* , 
\end{align*}
\noindent indicating that the derivative we're after is nothing more than
\begin{dmath*}
     \partialdd{}{\lambda} [h_{\pa,\tau}(\lambda) - h_{\protp,\tau}(
    \lambda)]    = \int_{\ospace} \rho_{\mu_\pa} \cdot  \left[T_\pa^*(V^{'}_{\tau}(\pi_{\pa,\lambda})) +  \left(\frac{1-p_\pa }{p_\pa}\right)V^{'}_{\tau}(\pi_{\protp,\frac{1-\lambda}{p_\pa} + \lambda})T_\protp^* - \left(\frac{p_\pa-1}{p_\pa}\right)V^{'}_{\tau}(\pi_{\protp,\frac{1-\lambda}{p_\pa} + \lambda})\id - V^{'}_{\tau}(\pi_{\pa,\lambda})\id)\right]  d\ell.
\end{dmath*}

By its definition, the derivative of $V^{'}_{\tau}(\pi_{\prot,\lambda})$ is exactly the Dirac delta function $\delta(\pi_{\prot,\lambda} - \tau)$.  Making this substitution, the above yields 
\begin{dmath*}
    \partialdd{}{\lambda} [h_{\pa,\tau}(\lambda) - h_{\protp,\tau}( \lambda)]= \\ 
    % \int_{\ospace} \rho_{\mu_\pa} \cdot  \left[T_\pa^\protp(\delta(\pi_\lambda - \tau) + \delta(\pi_{1-\lambda} - \tau)) - \id(\delta(\pi_\lambda - \tau) + \delta(\pi_{1-\lambda} - \tau))\right] d\ell. \\ 
   \int_{\ospace} \rho_{\mu_\pa} \cdot \left[T_\pa^*(\delta(\pi_{\pa,\lambda}-\tau)) +  \left(\frac{1-p_\pa }{p_\pa}\right)\delta(\pi_{\protp,\frac{1-\lambda}{p_\pa} + \lambda}-\tau)T_\protp^* - \left(\frac{p_\pa-1}{p_\pa}\right)\delta(\pi_{\protp,\frac{1-\lambda}{p_\pa} + \lambda}-\tau)\id - \delta(\pi_{\pa,\lambda}-\tau)\id)\right].
\end{dmath*}
Then, by definition of $\delta$, we at last obtain
\begin{dmath*}
     \partialdd{}{\lambda} [h_{\pa,\tau}(\lambda) - h_{\protp,\tau}(
    \lambda)]  = \left[T_\pa^* +  \left(\frac{1-p_\pa }{p_\pa}\right)T_\protp^* - \left(\frac{p_\pa-1}{p_\pa}\right)\id - \id\right] \circ \tau .
    %= \\ 
    % \int_{\ospace} \rho_{\mu_\pa} \cdot  \left[T_\pa^\protp(\delta(\pi_\lambda - \tau) + \delta(\pi_{1-\lambda} - \tau)) - id(\delta(\pi_\lambda - \tau) + \delta(\pi_{1-\lambda }- \tau))\right] d\ell = 
    % \rho_{\mu_\pa}(\tau) \cdot 2(T_\pa^\protp(\tau) - id(\tau)).  
\end{dmath*}

Since the above does not depend on $\lambda$,  taking another derivative simply yields  $\frac{d^2}{d\lambda^2} [h_{\pa,\tau}(\lambda) - h_{\protp,\tau}(\lambda)] = 0$. From this, we take the second derivative of the absolute value of this difference, i.e., 
\begin{dmath}
\label{eq:convexity_inside_derivative}
   \frac{d}{d^2\lambda} |h_{\pa,\tau} - h_{\protp,\tau}| = \\
   \text{sign}(h_{\pa,\tau} - h_{\protp,\tau})\underbrace{\frac{d^2}{d\lambda^2} [h_{\pa,\tau}(\lambda) - h_{\protp,\tau}(\lambda)]}_{=~0} + 2 \underbrace{\delta(h_{\pa,\tau} - h_{\protp,\tau})}_{\simeq ~0~\text{or}~1}\underbrace{(\cdot)^2}_{\geq 0}. 
\end{dmath}
The first term on the r.h.s., we've already shown is zero, and the second term is also non-negative.  Another application of Leibniz' Rule allows that \begin{align*}
      \frac{d}{d^2\lambda}\underbrace{\Expect_{\tau \sim U(\ospace)}|h_{\pa,\tau} - h_{\protp,\tau}|}_{\UF_\gamma(f_\lambda)} = \Expect_{\tau \sim U(\ospace)}\left|\underbrace{\frac{d}{d^2\lambda}[h_{\pa,\tau} - h_{\protp,\tau}]}_{\geq 0 ~ \text{by (\ref{eq:convexity_inside_derivative})}}\right|.
\end{align*}
This indicates that $\UF_\gamma(f_\lambda)$ is convex (i.e., we have shown that the second derivative is non-negative).  The existence of a a solution to $\lambda_* \leftarrow \argmin_{\lambda \in \binaryrange} \UF_{\gamma}(\f_\lambda)$ is guaranteed by this fact, therefore indicating that $f_{\lambda_*}$ maximizes distributional parity in the set of repaired regressors.  
\end{proof}



As noted in Section~\ref{sec:geometric_repair}, the validity of Theorem~\ref{thm:convex} indicates that finding the distributional-parity-maximizing regressor reduces to a univariate optimization problem.  Locating the optimal $\lambda_*$, such that $f_{\lambda^*}$ satisfies the desired fairness metric $\gamma$, with the following caveat:  Our results for \emph{maximizing} distributional parity do not claim that we achieve \emph{perfect} distributional parity; however, we are able to show experimentally that our Algorithm \ref{alg:repair} is remarkably successful in achieving parity in almost all cases (Section~\ref{sec:experiments} and Appendix~\ref{appendix:experiments}).


\textbf{Corollary~\ref{cor:additive}.} Since convex functions are closed under addition, Theorem~\ref{thm:convex} also applies to additive combinations of $\UF_{\gamma_1}(f_\lambda) +\UF_{\gamma_2}(f_\lambda) +  ....  + \UF_{\gamma_m}(f_\lambda)$


\iffalse
\subsection{Impossibility Result?}

\TODO{?}

Before we show our concrete post-processing algorithm and empirical results, we offer one more theoretical insight.
\begin{theorem}
Any $f$ which satisfies distributional parity for $\gamma=\PR$ will not satisfy distributional parity for $\gamma=TPR$ nor $\FPR$ unless group conditional score distributions and labels are conditionally independent, i.e., $\Scorerv|\Protrv \perp \Yrv$. 
\end{theorem}

\fi
