# Supplementary material for: Repairing Regressors for Fair Binary Classification at Any Decision Threshold
Source: arXiv:2203.07490 source file (2023-12-10)
Supplement: Supplementary file 6 [file 50_empirical.tex]

\section{Experimental Configuration and Additional Results}\label{appendix:experiments}

We provide details about our Algorithm, and experimental configurations in Section~\ref{sec:experiments}, as well as additional results on other datasets.

\subsection{Algorithm~\ref{alg:repair} and Differentiation.}~
We show in the proof of Theorem \ref{app:proofs:thm1} that computing the derivative of $\UF_\gamma(f_\lambda)$ requires knowledge of the probability density function of either group's distribution of scores (denoted $\rho_{\mu_\prot}$).  Often, this distribution is not known, therefore preventing us from using more traditional, derivative based optimization techniques. 

\subsection{Experimental configuration details, and reproducibility for main paper results}

Code for all experiments, as well as instructions for reproducing our specific results, can be found in the anonymous repository located \url{https://anonymous.4open.science/r/distributional-fairness-436F/}{here}.

For Figure~\ref{fig:dist-compare} in the main paper, which compares our method for achieving distributional parity against other all-threshold fairness methods, we needed to do extensive hyperparameter tuning to find the best-performing repair parameter for the algorithm in \citet{feldman2015certifying}. In more detail, the algorithm in \citet{feldman2015certifying} includes a \texttt{repairlevel} hyperparameter, which, similar to our $\lambda$ (found through optimization, rather than a chosen hyperparameter), controls the extent to which inputs are adjusted during pre-processing. We performed grid search using $\texttt{repairlevel} \in \{0.05, 0.15, 0.2, ..., 0.95, 1.0\}$. When comparing our method to that in \citet{feldman2015certifying} for a given $\gamma$, we do so using the \texttt{repairlevel} that yielded the best results from grid search for that $\gamma$. %In other words, Figure \ref{fig:dist-parity} shows the over-threshold performance that Feldman could achieve at \textit{any} repairlevel. 
For our implementation, we incorporated the open-source implementation of \citet{feldman2015certifying}, available in the Fairlearn package~\citep{bird2020fairlearn}. 

\subsection{Additional experiments}

\custompar{Additional dataset}
In addition to the two datasets from the main paper, we also show results here for the 
% we use an additional task from \texttt{Adult} \citep{ding2021retiring}, Public Coverage, where the sensitive feature is race and the target variable is whether an individual uses public health insurance; as well as the 
\texttt{Taiwan Credit} dataset \citep{bay2000uci}, where the sensitive
attribution is education level and the target variable is good credit.

\custompar{Additional models}
In addition to Logistic Regression and SVM models, we show results below for scores generated by an underlying Random Forest and 2-layer neural network; again, we use \texttt{scikit-learn} implementations with default hyperparameters.

% \TODO{We should include all the figures we want (I believe we said additional Figures that look like Figure 3?), along with dataset information akin to what we put in the main paper for old and new Adult. With each result, we should include information about HPO, if necessary. If not, e.g., if the HPO in the main paper applies here, then we should just note that the subsection above is sufficient.}

\custompar{Additional Discussion}
In our additional experiments we show that our method works very well across a combination of models and datasets however, there are two main minor limitations we'd like to discuss.  The experiment in which we removed the least disparity, was SVMs on the \texttt{Adult} Income-Sex task, for Equalized Odds, see Figure \ref{fig:app:adult_old_svm}.  We have hypothesized that our method may be ineffective here due an abnormality in the classifier's score distributions.  Specifically, we point out the SVM hardly assigns scores $<.15$, for the Female group, thereby inflating error rates for members of that group, with scores above 0.15. We look forward to investigating ways to improve our performance on this task in future work. Additionally, there are some cases in which we record very little disparity in the unrepaired regressor. For some of these cases, despite increasing parity at almost every threshold, our method \textit{marginally} decreases parity at certain select threshold(s), see for example, in Figure \ref{fig:app:adult_new_svm} at $\tau=0.2$. We believe that this effect is neither pervasive nor significant; in most cases, we do not see any parity decreases. With that said, in the scenarios where parity slightly decreases at a threshold, we note that our algorithm still increases total parity on average, almost achieving parity across all other thresholds. 

% \jessica{
% i think fig 6 is actually super interesting. fig 6a is basically telling us that the svm basically never gives a score greater than 0.15ish for the female group; so we can improve the distribution of scores and achieve SDP. however, we have almost no information about how those scores --- the ones we bumped up from 0.15ish to something between 0.15-1 --- relate to labels. So we can't to that much more to bring down the error for the female group for $\tau > 0.15$. 
% There's probably a more mathematically rigorous to say this, but I think that's what's happening here. does that make sense?  
% }

% \TODO{Say something about results for which we didn't really do much better (but still), but still changed the distribution, and seemed to add more disparity at some thresholds, e.g. Fig 10 Eq. Odds results}

% \jessica{
% Probably something similar (but maybe weaker) is going on here, and increasing disparity slightly at $\tau \approx 0.2$ is the price we pay for minimizing expected disparity over $\tau \in [0.3, 0.8]$.
% }

% %%%%% ADULT OLD
The following figures represent additional results for models trained on:

\begin{itemize}
    \item \texttt{Adult} UCI~\citep{dua2017uci} (Figures~\ref{fig:app:adult_old_lr},~\ref{fig:app:adult_old_svm},~\ref{fig:app:adult_old_rf},~\ref{fig:app:adult_old_mlp})
    \item New \texttt{Adult}~\citep{ding2021retiring} (Figures~\ref{fig:app:adult_new_lr},~\ref{fig:app:adult_new_svm},~\ref{fig:app:adult_new_rf},~\ref{fig:app:adult_new_mlp})
    \item \texttt{Taiwan Credit}\citep{bay2000uci} (Figures~\ref{fig:app:taiwan_lr},~\ref{fig:app:taiwan_svm},~\ref{fig:app:taiwan_rf},~\ref{fig:app:taiwan_mlp})
\end{itemize}

\begin{figure*}[!ht]
    \centering
    \begin{minipage}{.33\textwidth}
        \centering
        \includegraphics[width=0.9\linewidth]{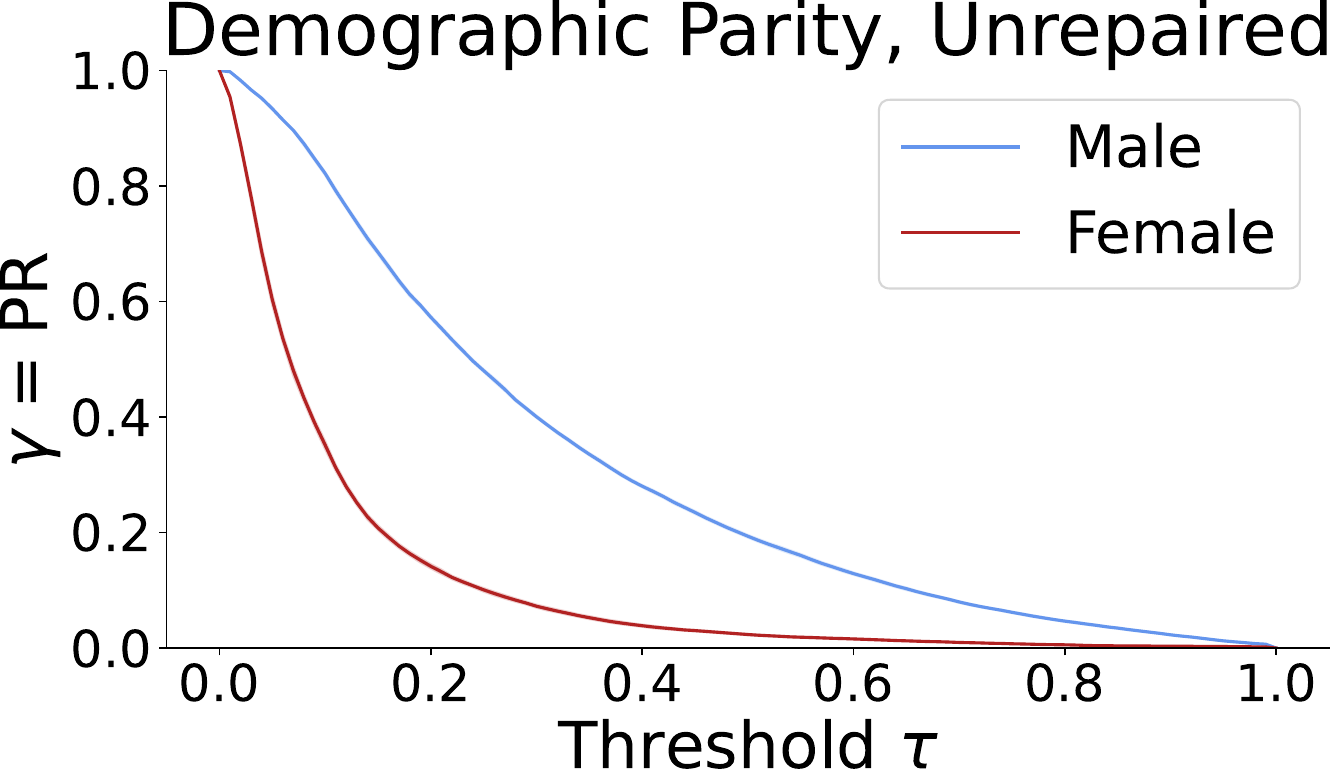}\\
        \includegraphics[width=0.9\linewidth]{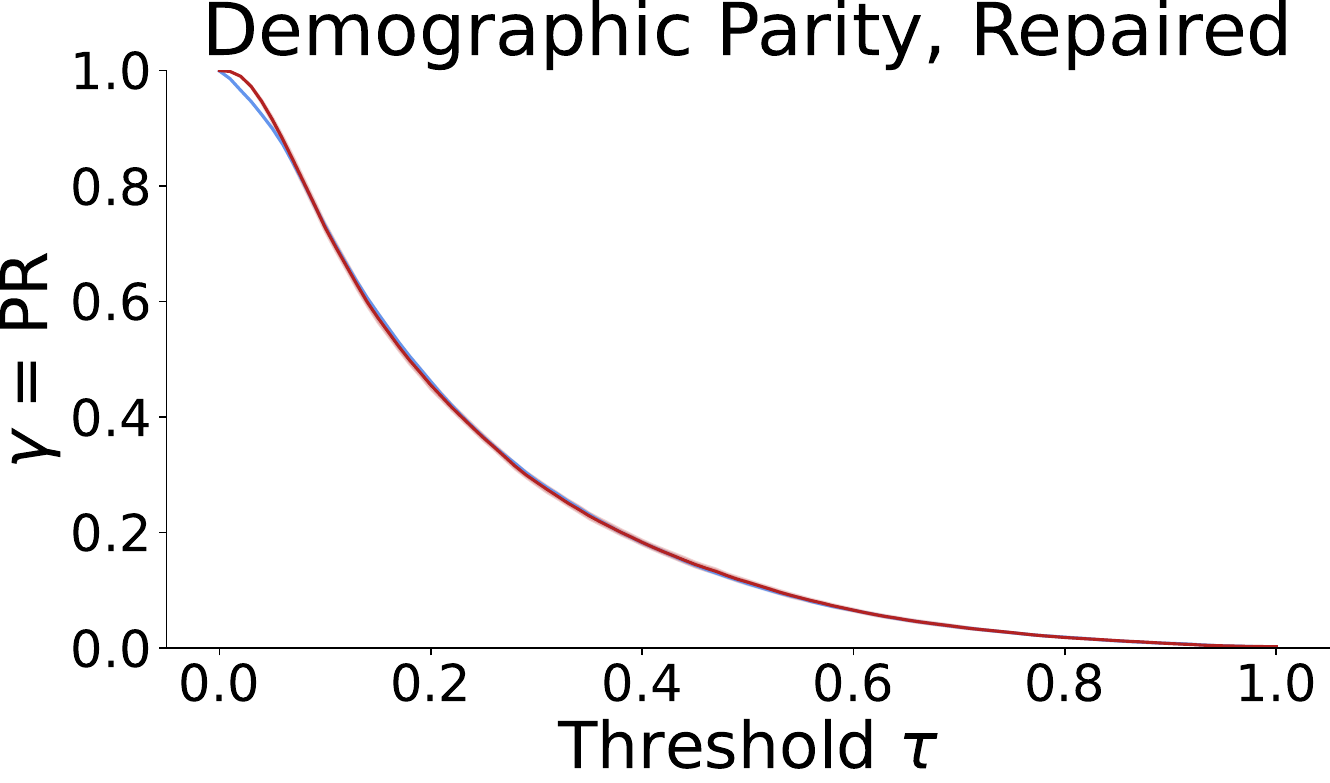}
        \subcaption{Algorithm~\ref{alg:repair} results for SDP}
        \label{fig:app:adult_old_lr-sdp}
    \end{minipage}%
    \begin{minipage}{0.66\textwidth}
        \centering
        \includegraphics[width=0.45\linewidth]{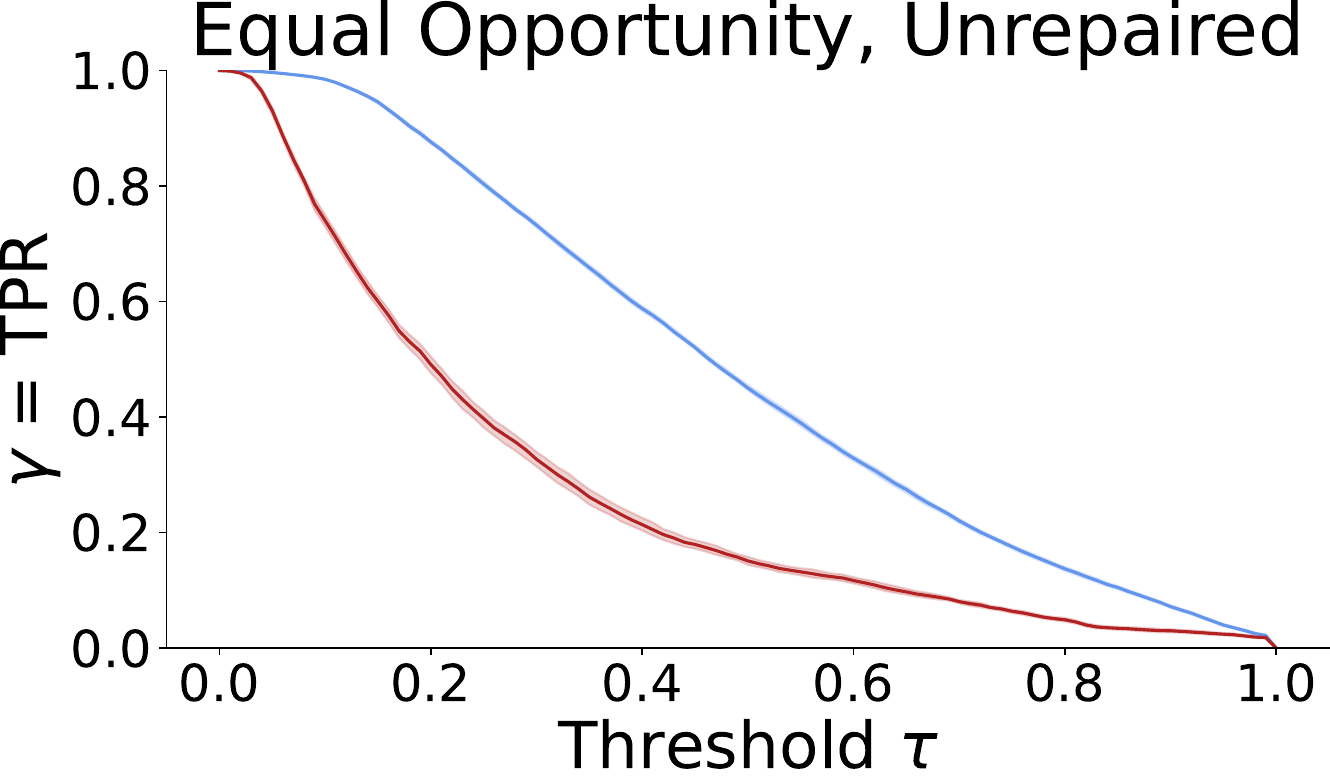}
        \includegraphics[width=0.45\linewidth]{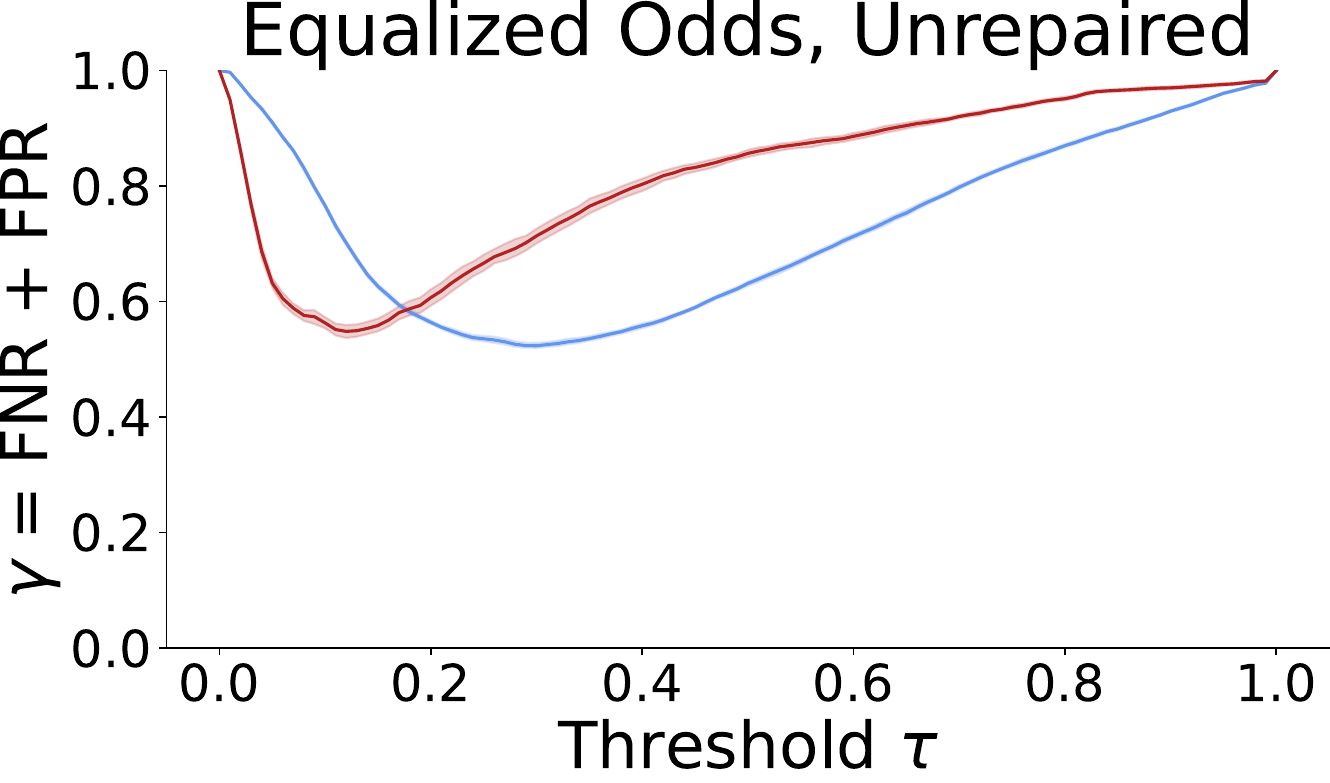}\\
        \includegraphics[width=0.45\linewidth]{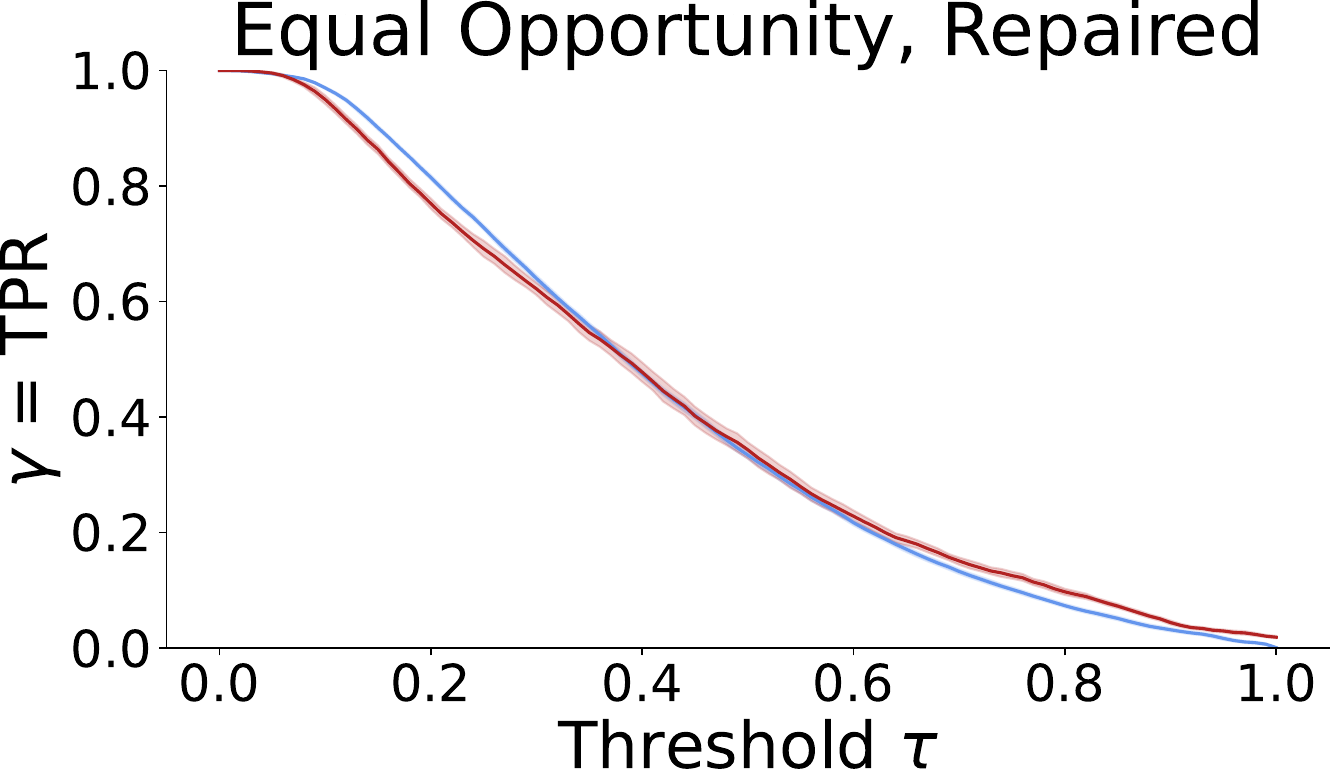}
        \includegraphics[width=0.45\linewidth]{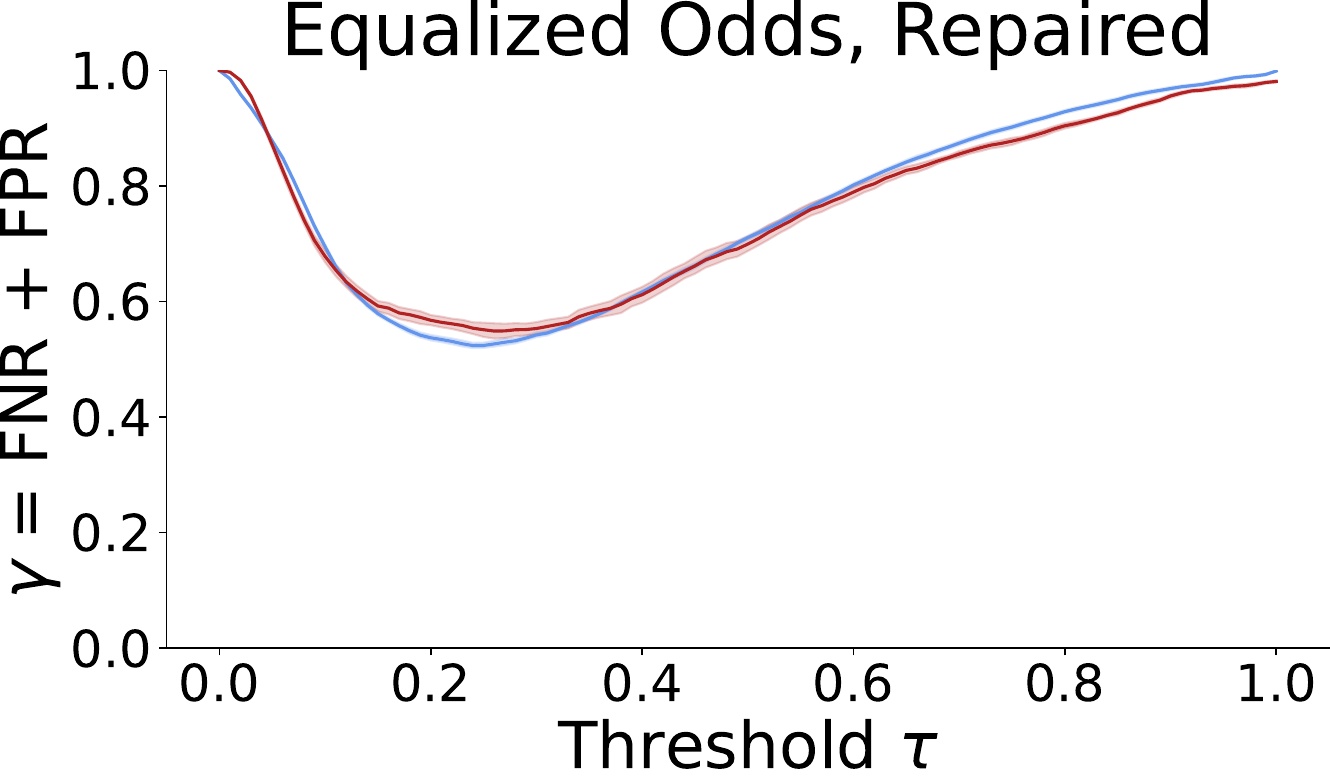}\\
        \subcaption{Algorithm~\ref{alg:repair} results for Eq. Odds and Eq. Opportunity}
        \label{fig:app:adult_old_lr-ours}
    \end{minipage}
    \vspace{-.2cm}
    \caption{Comparing unrepaired and repaired logistic regression on \texttt{Adult} Income-Sex~\citep{dua2017uci}.}
    \label{fig:app:adult_old_lr}
    \vspace{-.2cm}
\end{figure*}

\begin{figure*}[!ht]
    \centering
    \begin{minipage}{.33\textwidth}
        \centering
        \includegraphics[width=0.9\linewidth]{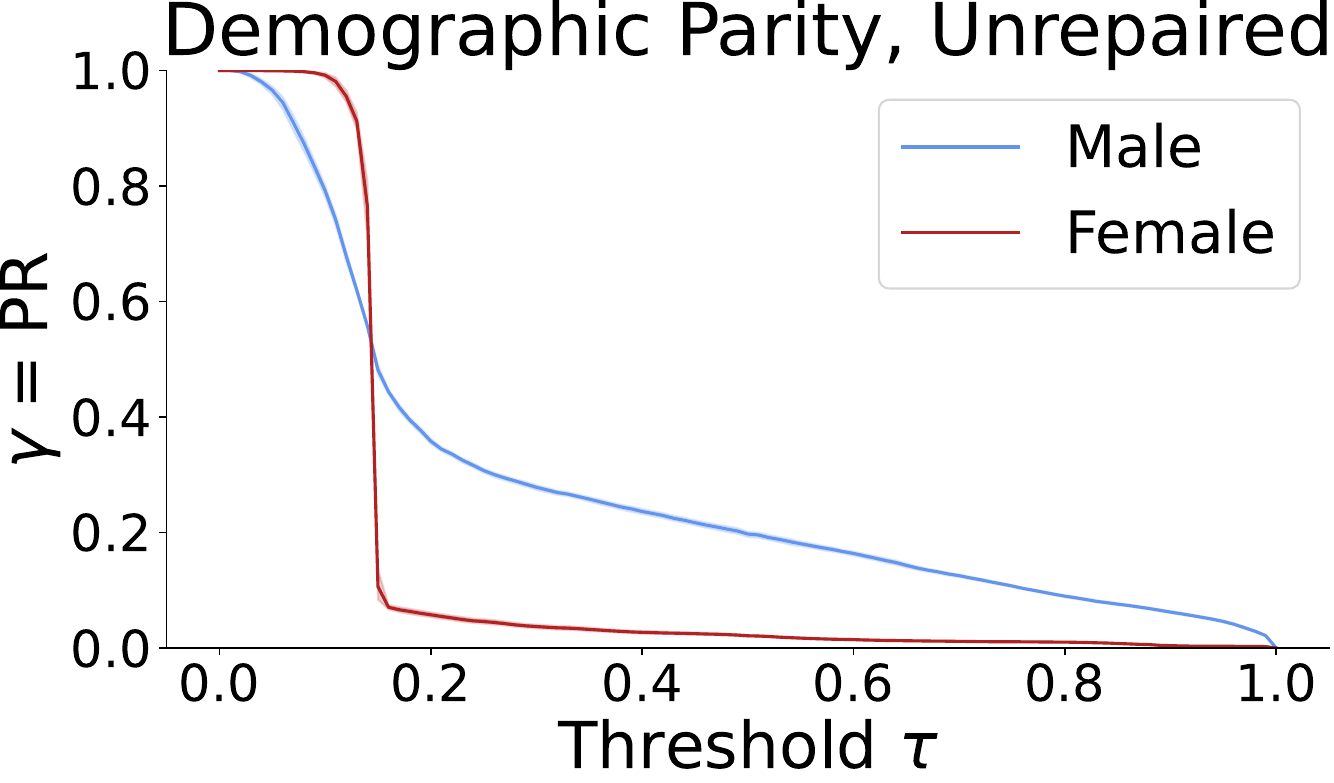}\\
        \includegraphics[width=0.9\linewidth]{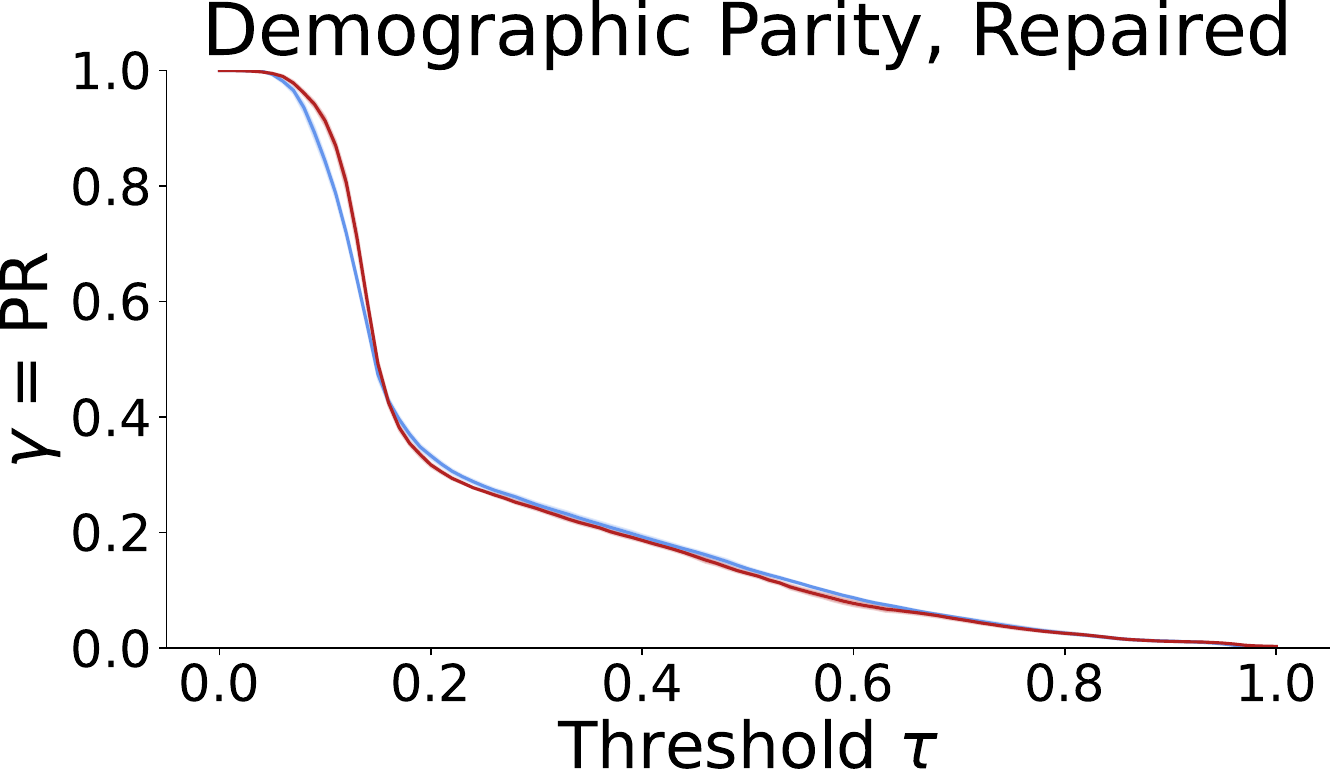}
        \subcaption{Algorithm~\ref{alg:repair} results for SDP}
        \label{fig:app:adult_old_svm-sdp}
    \end{minipage}%
    \begin{minipage}{0.66\textwidth}
        \centering
        \includegraphics[width=0.45\linewidth]{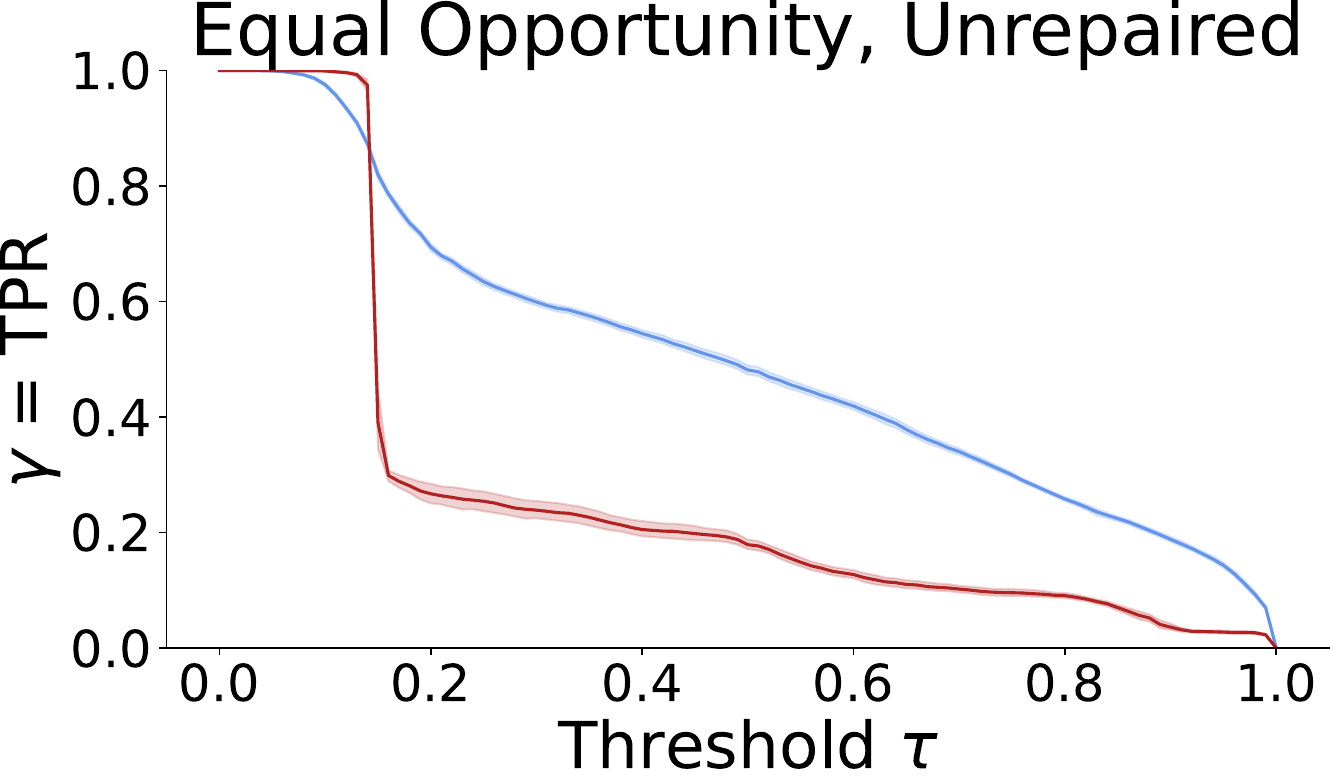}
        \includegraphics[width=0.45\linewidth]{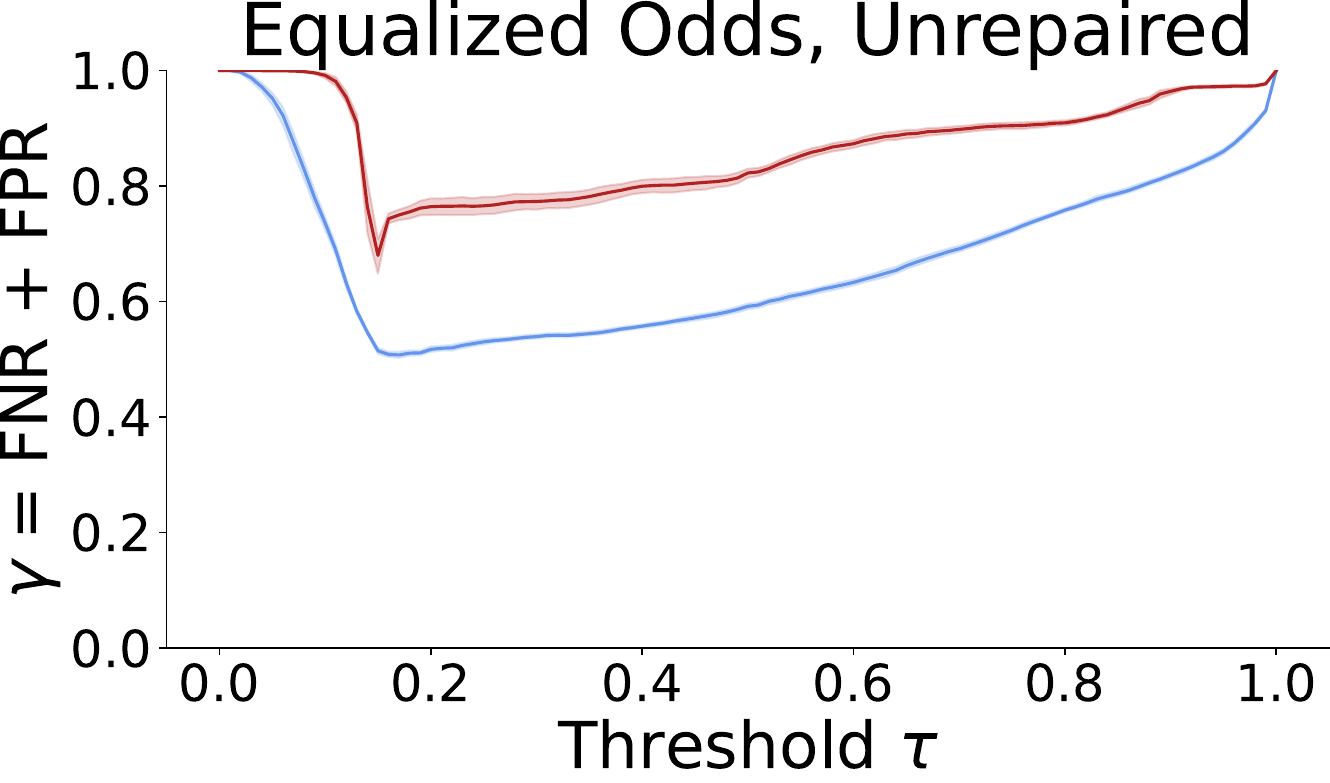}\\
        \includegraphics[width=0.45\linewidth]{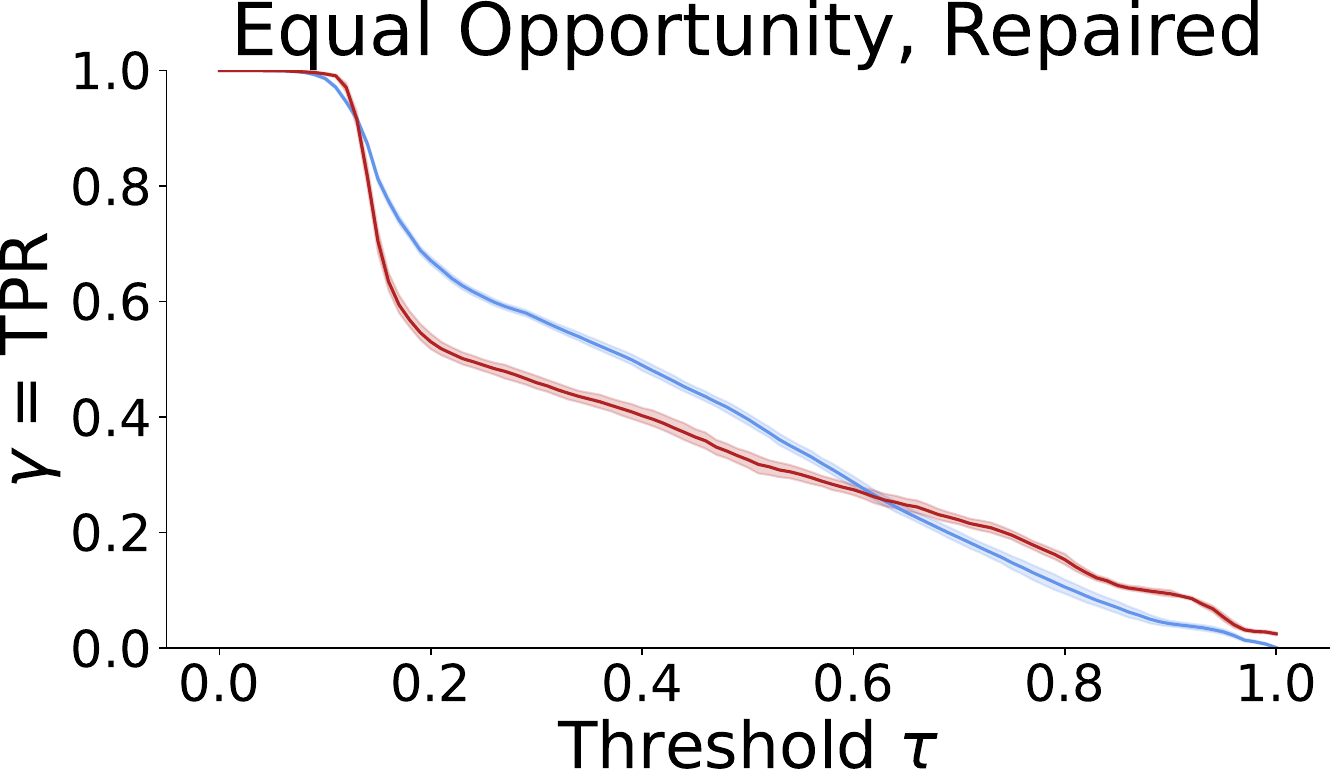}
        \includegraphics[width=0.45\linewidth]{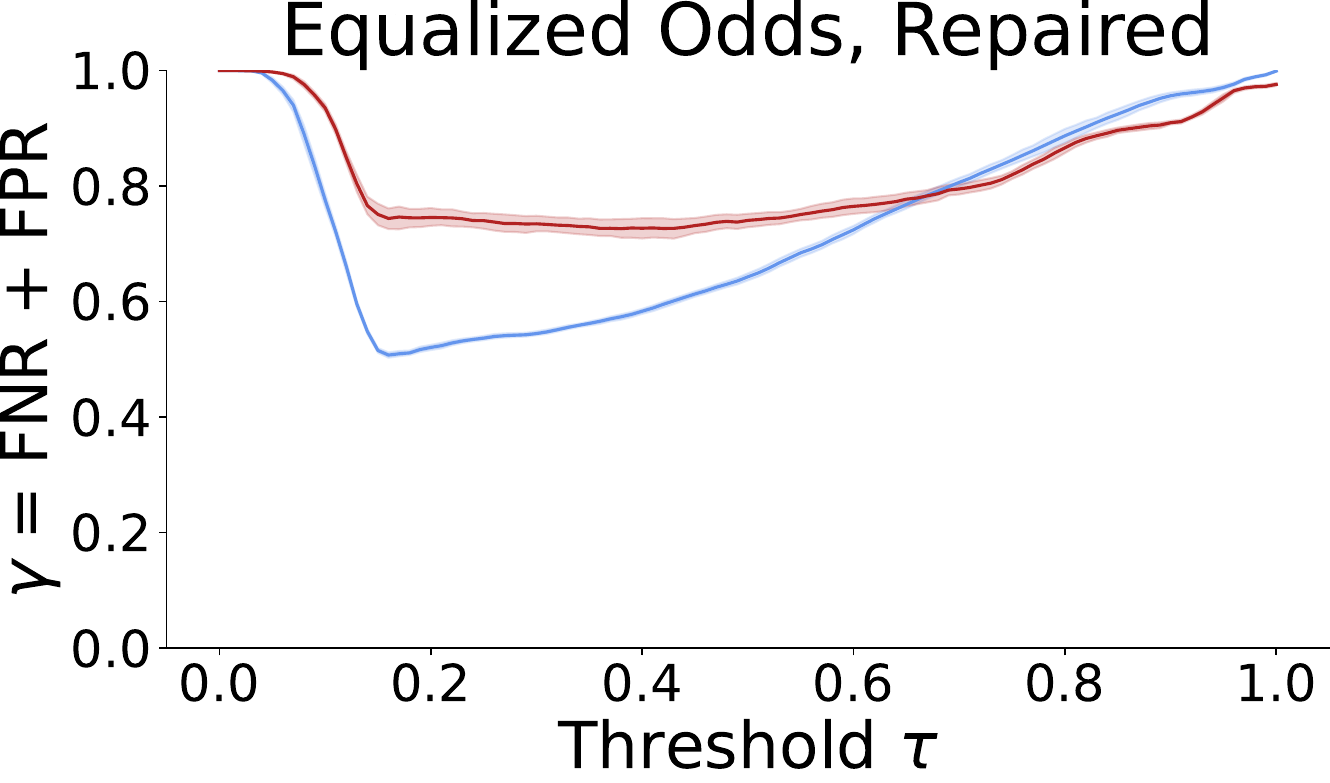}\\
        \subcaption{Algorithm~\ref{alg:repair} results for Eq. Odds and Eq. Opportunity}
        \label{fig:app:adult_old_svm-ours}
    \end{minipage}
    \vspace{-.2cm}
    \caption{Comparing unrepaired and repaired SVMs on \texttt{Adult} Income-Sex~\citep{dua2017uci}.} 
    \label{fig:app:adult_old_svm}
    \vspace{-.2cm}
\end{figure*}

\begin{figure*}[!ht]
    \centering
    \begin{minipage}{.33\textwidth}
        \centering
        \includegraphics[width=0.9\linewidth]{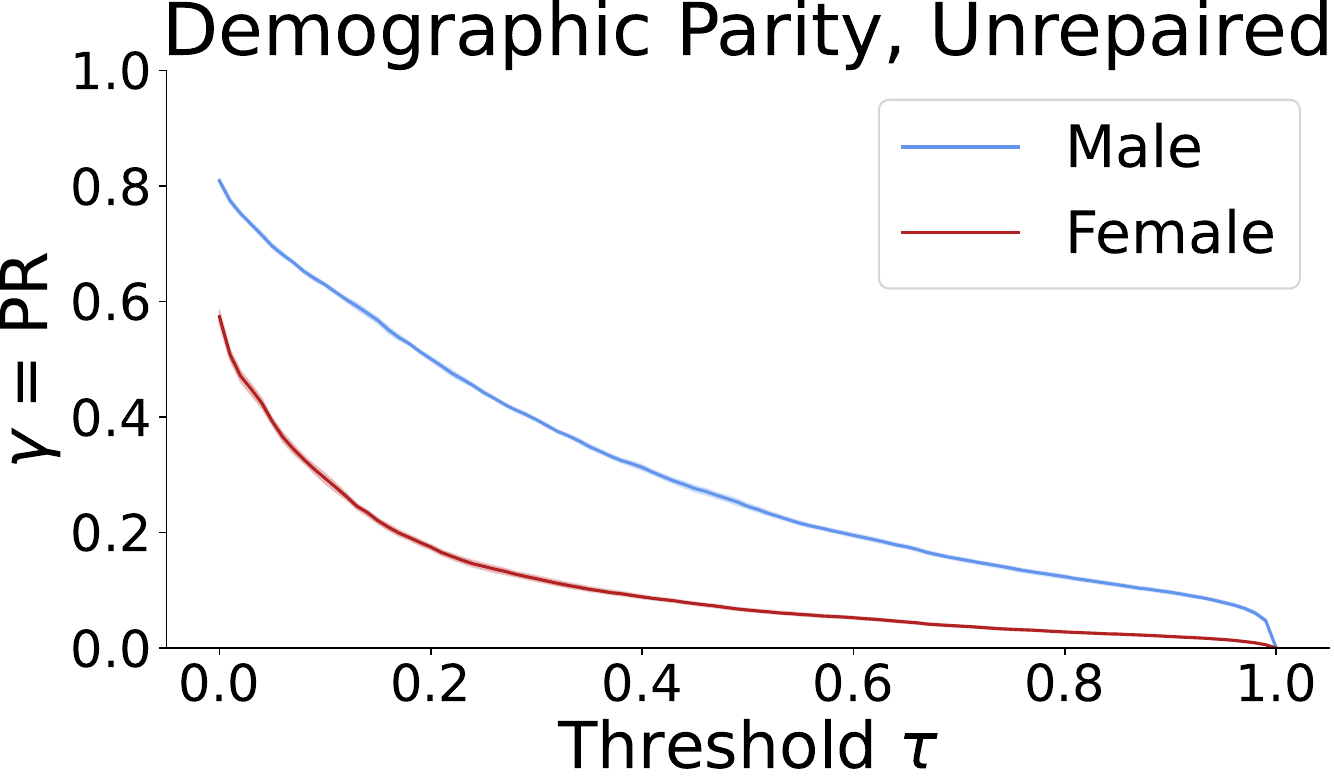}\\
        \includegraphics[width=0.9\linewidth]{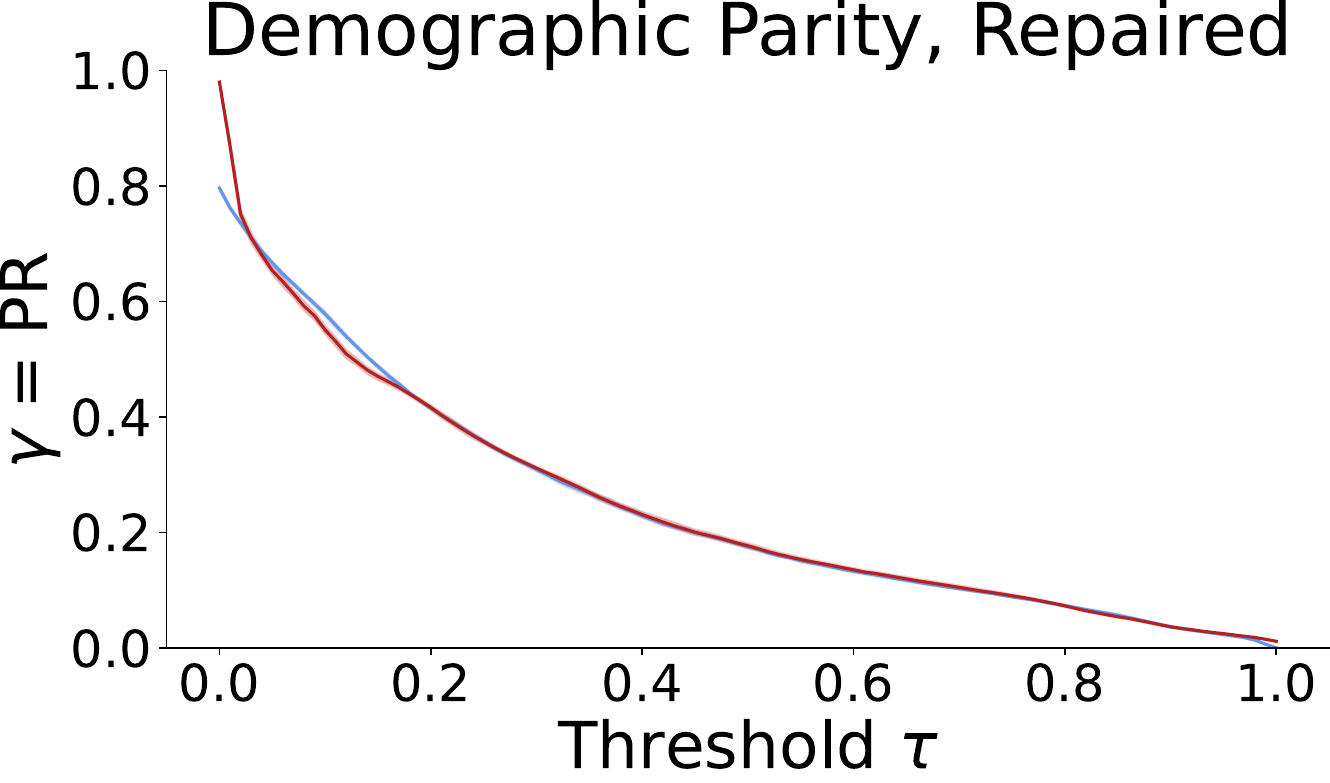}
        \subcaption{Algorithm~\ref{alg:repair} results for SDP}
        \label{fig:app:adult_old_rf-sdp}
    \end{minipage}%
    \begin{minipage}{0.66\textwidth}
        \centering
        \includegraphics[width=0.45\linewidth]{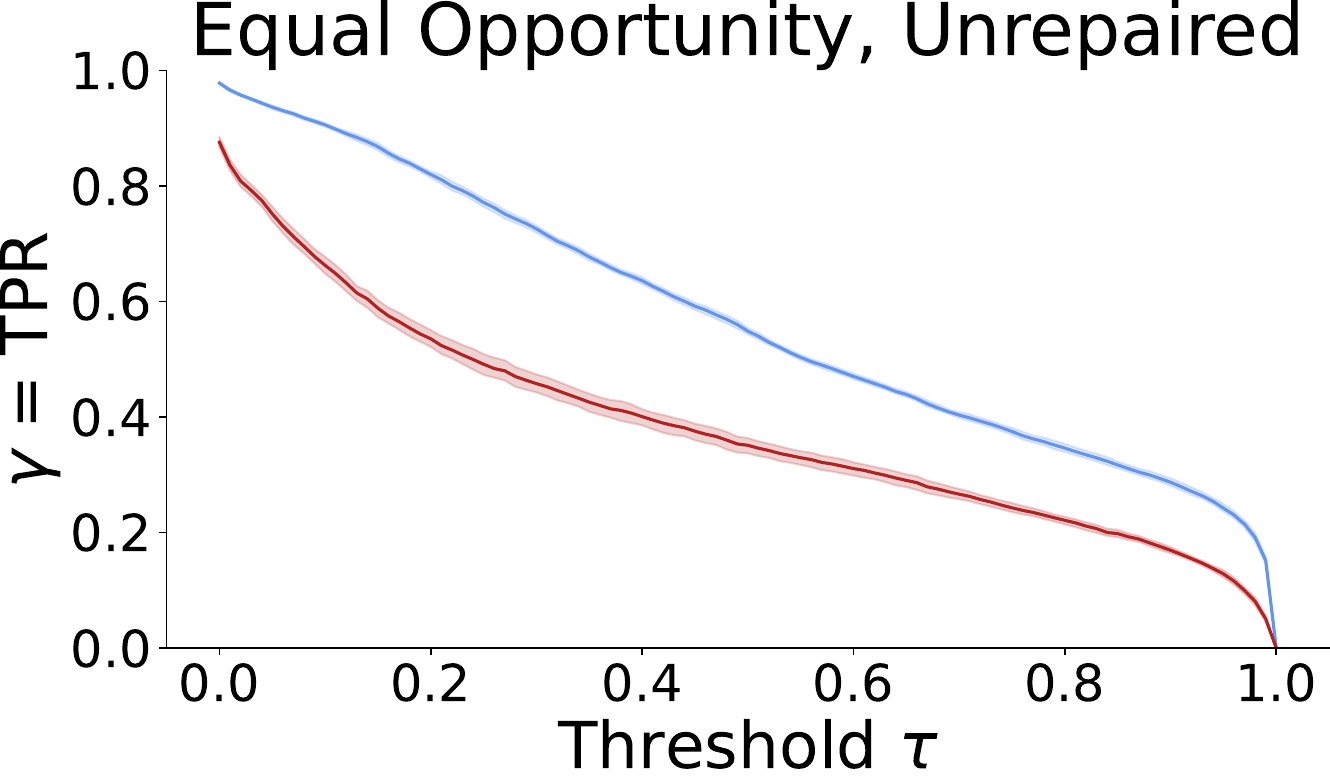}
        \includegraphics[width=0.45\linewidth]{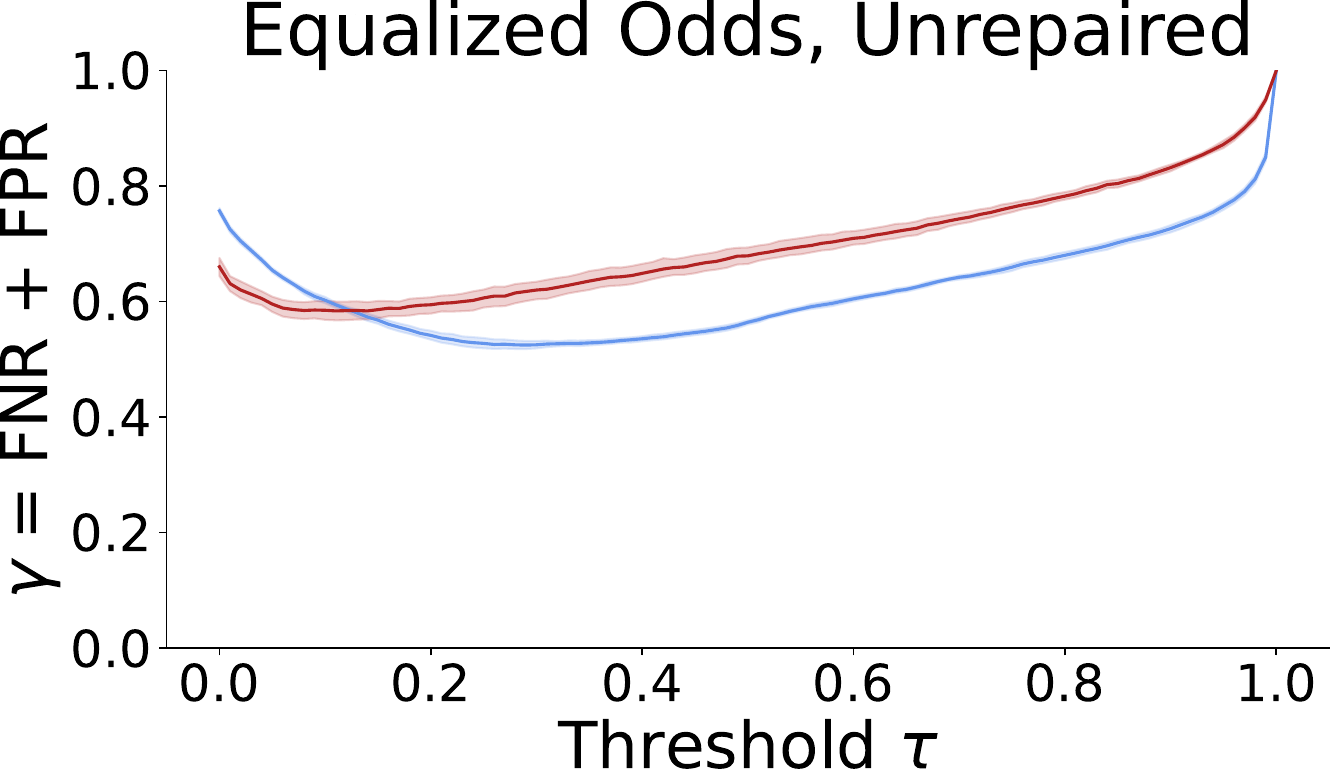}\\
        \includegraphics[width=0.45\linewidth]{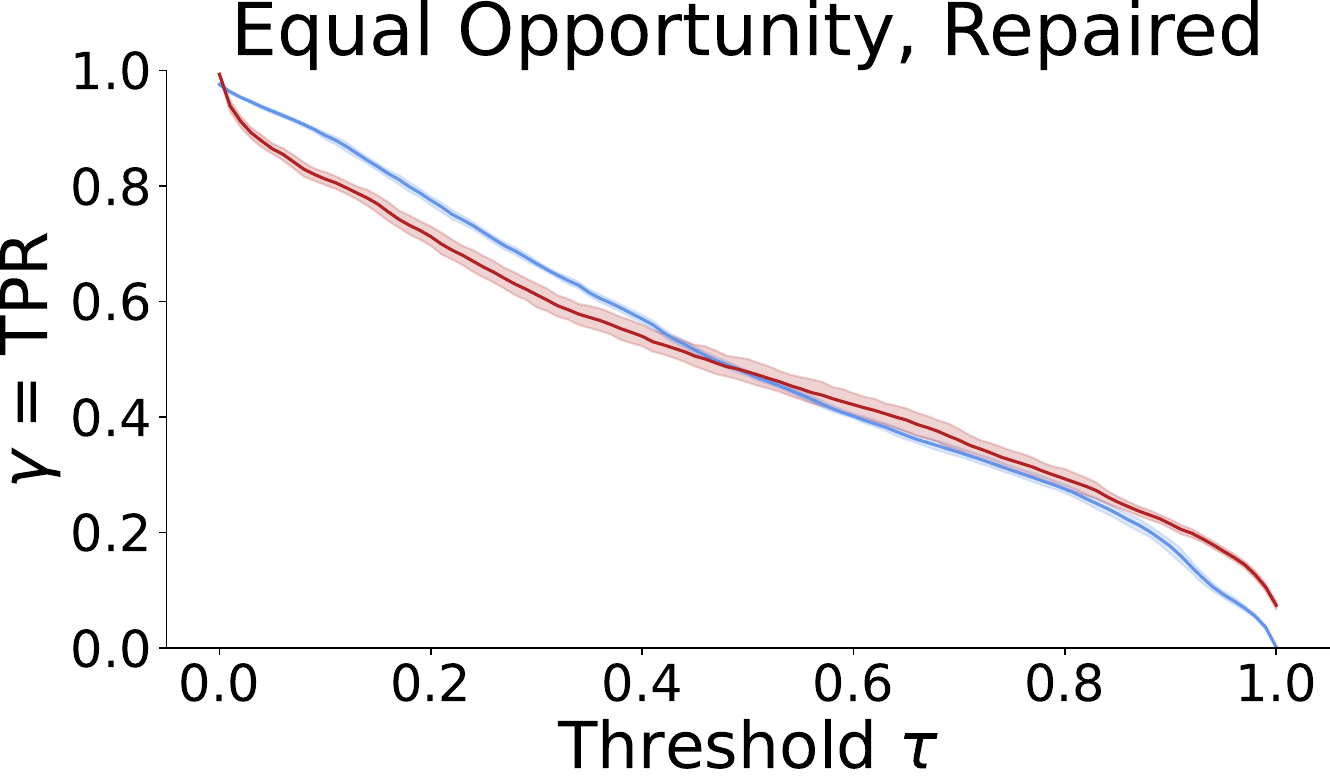}
        \includegraphics[width=0.45\linewidth]{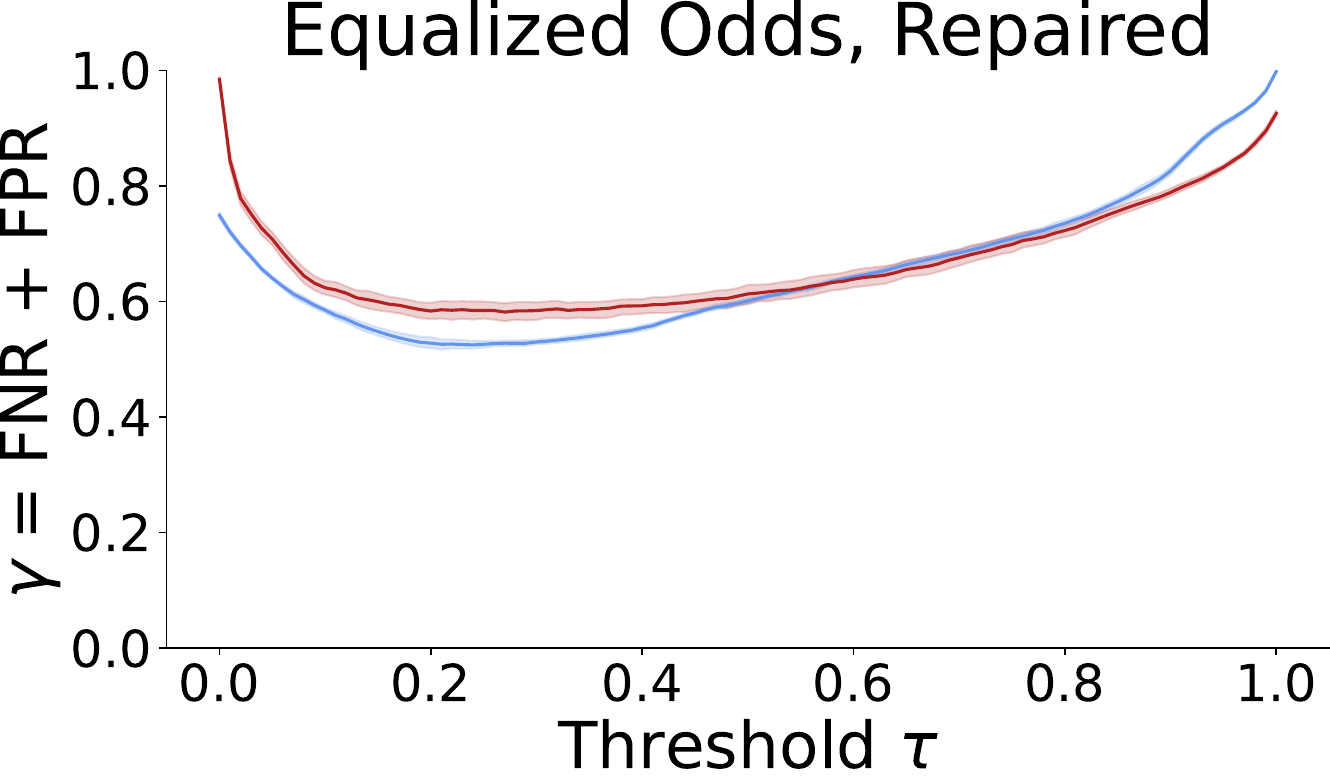}\\
        \subcaption{Algorithm~\ref{alg:repair} results for Eq. Odds and Eq. Opportunity}
        \label{fig:app:adult_old_rf-ours}
    \end{minipage}
    \vspace{-.2cm}
    \caption{Comparing unrepaired and repaired Random Forests on \texttt{Adult} Income-Sex~\citep{dua2017uci}.} 
    \label{fig:app:adult_old_rf}
    \vspace{-.2cm}
\end{figure*}

\begin{figure*}[!ht]
    \centering
    \begin{minipage}{.33\textwidth}
        \centering
        \includegraphics[width=0.9\linewidth]{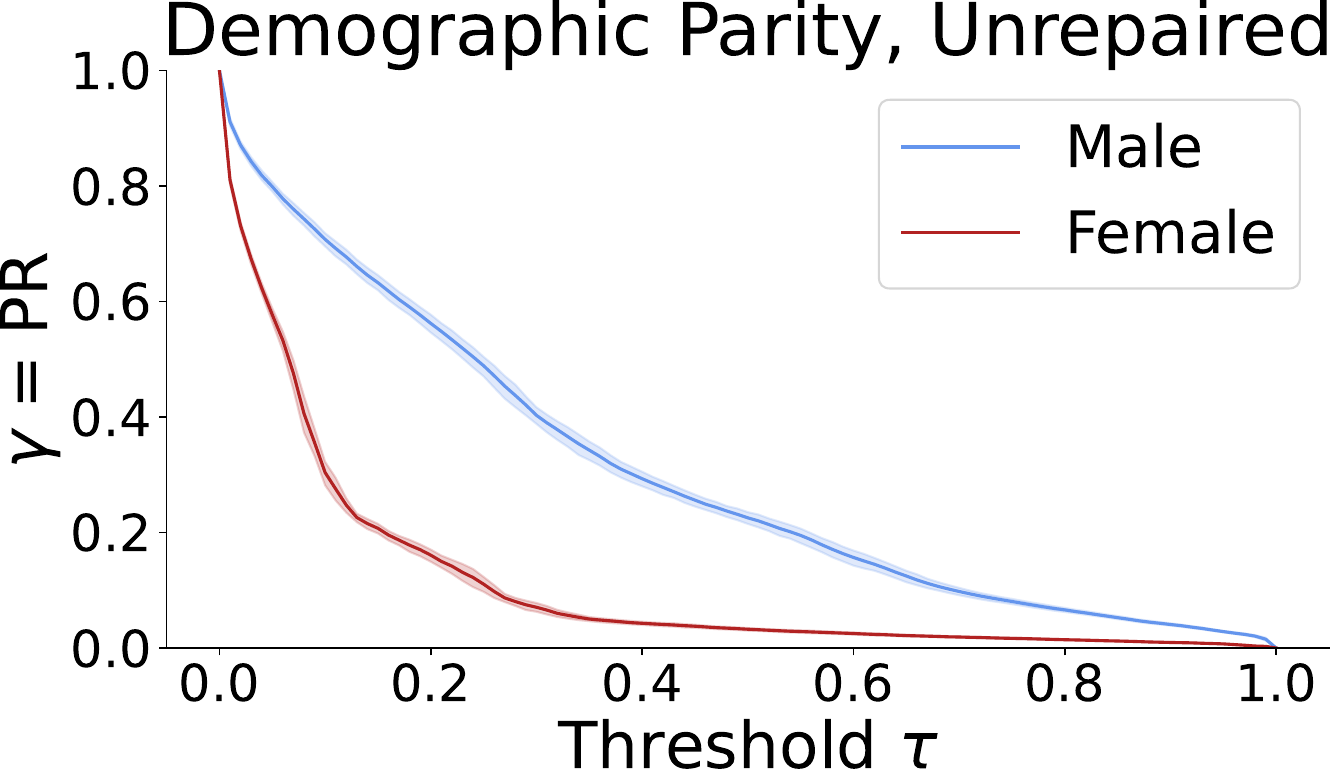}\\
        \includegraphics[width=0.9\linewidth]{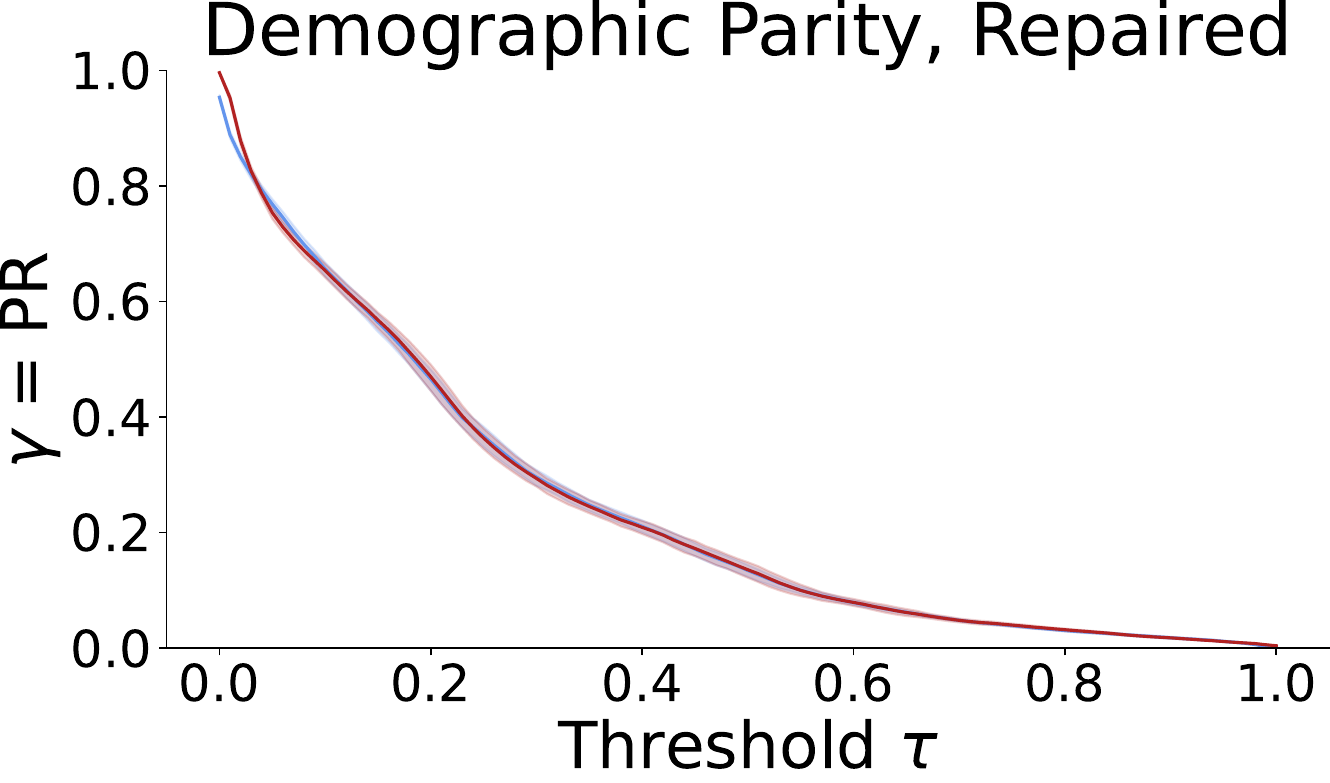}
        \subcaption{Algorithm~\ref{alg:repair} results for SDP}
        \label{fig:app:adult_old_mlp-sdp}
    \end{minipage}%
    \begin{minipage}{0.66\textwidth}
        \centering
        \includegraphics[width=0.45\linewidth]{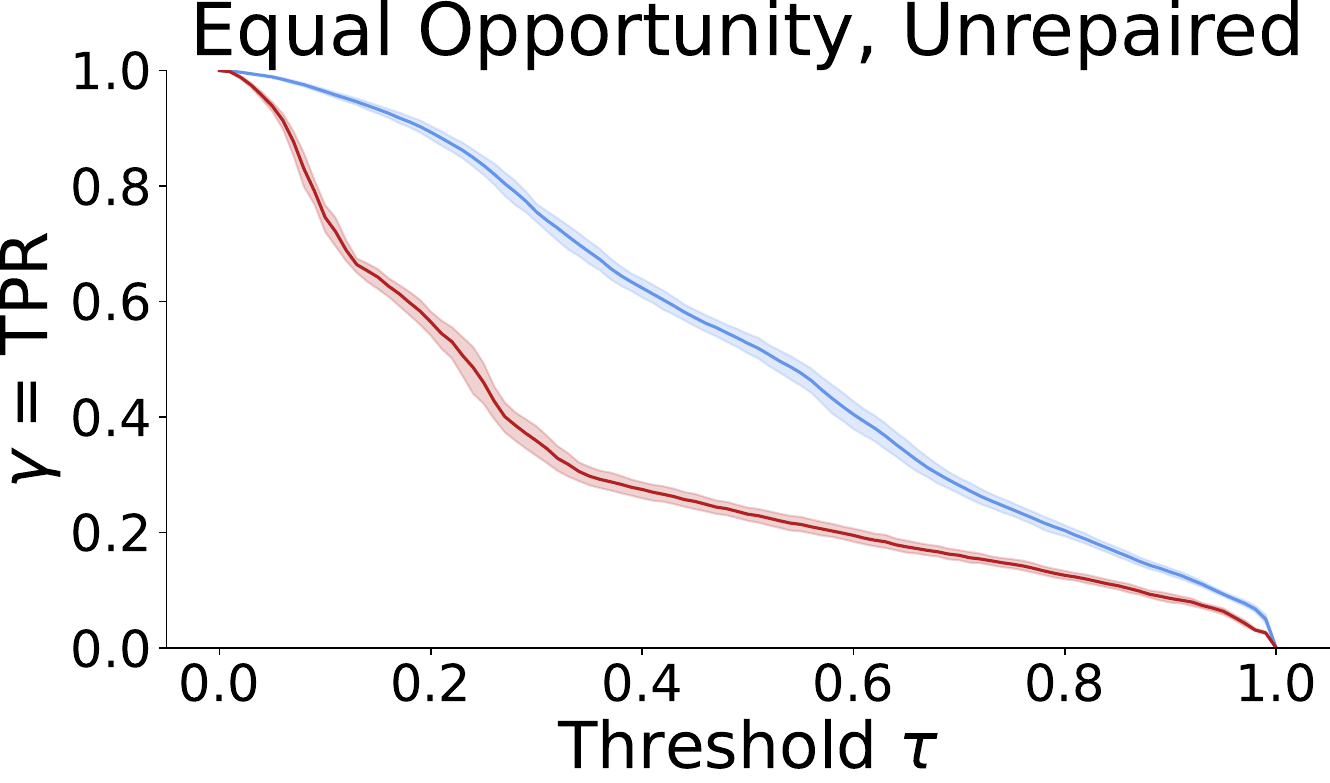}
        \includegraphics[width=0.45\linewidth]{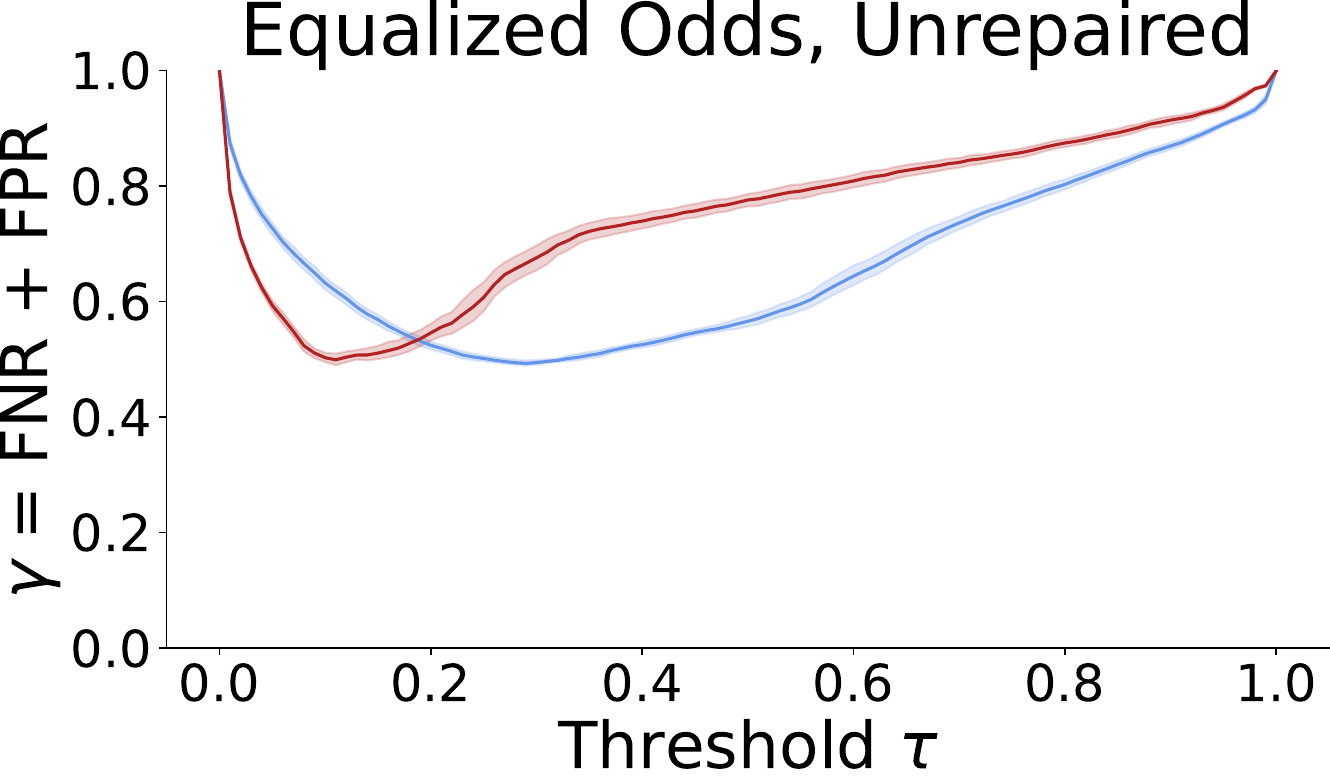}\\
        \includegraphics[width=0.45\linewidth]{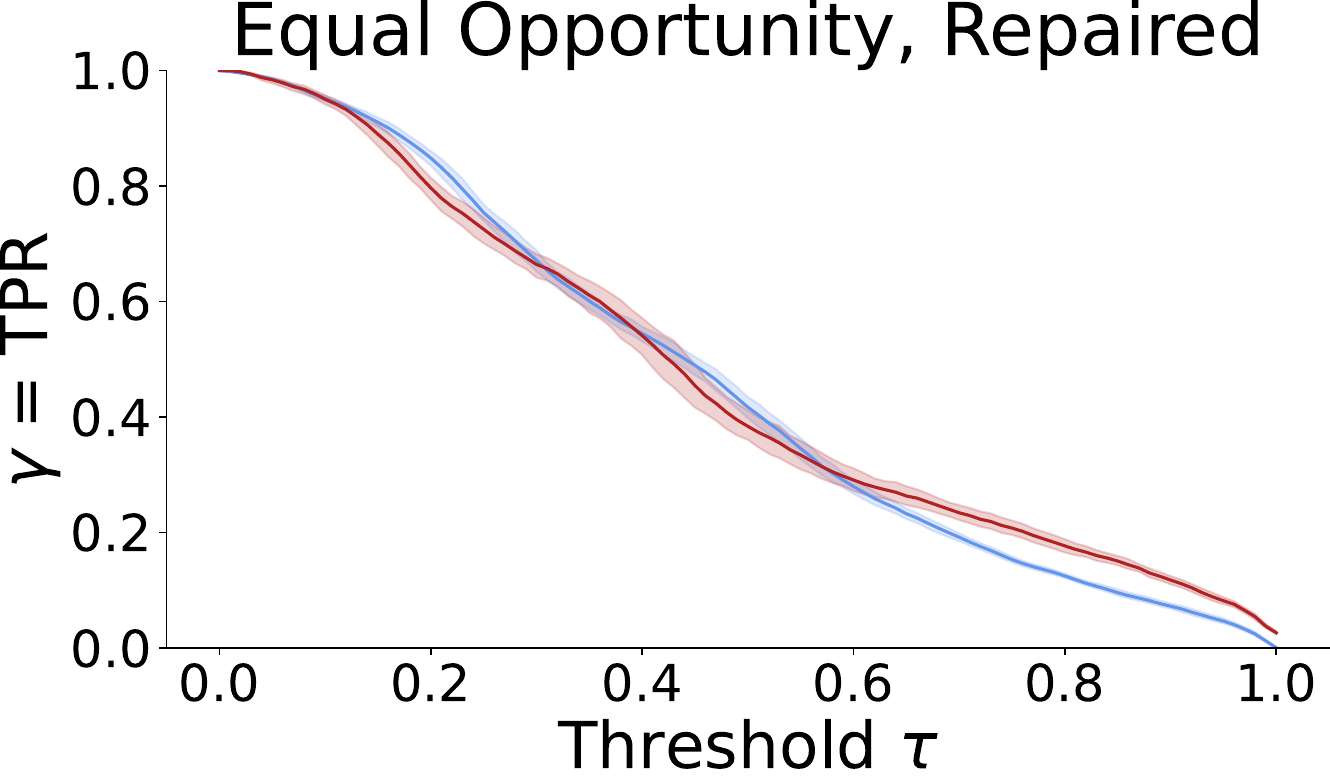}
        \includegraphics[width=0.45\linewidth]{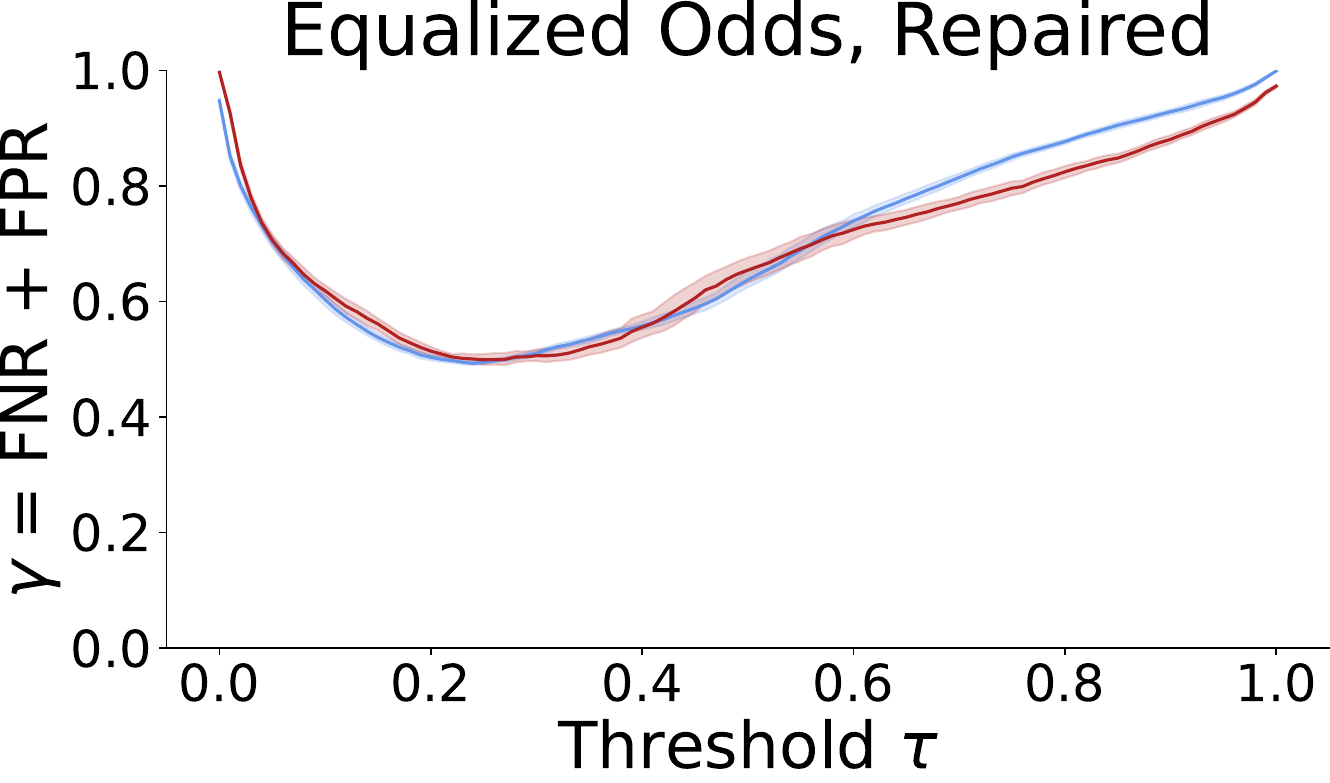}\\
        \subcaption{Algorithm~\ref{alg:repair} results for Eq. Odds and Eq. Opportunity}
        \label{fig:app:adult_old_mlp-ours}
    \end{minipage}
    \vspace{-.2cm}
    \caption{Comparing unrepaired and repaired MLPs on \texttt{Adult} Income-Race~\citep{dua2017uci}.} 
    \label{fig:app:adult_old_mlp}
    \vspace{-.2cm}
\end{figure*}

% %%%% ADULT NEW 

\begin{figure*}[!ht]
    \centering
    \begin{minipage}{.33\textwidth}
        \centering
        \includegraphics[width=0.9\linewidth]{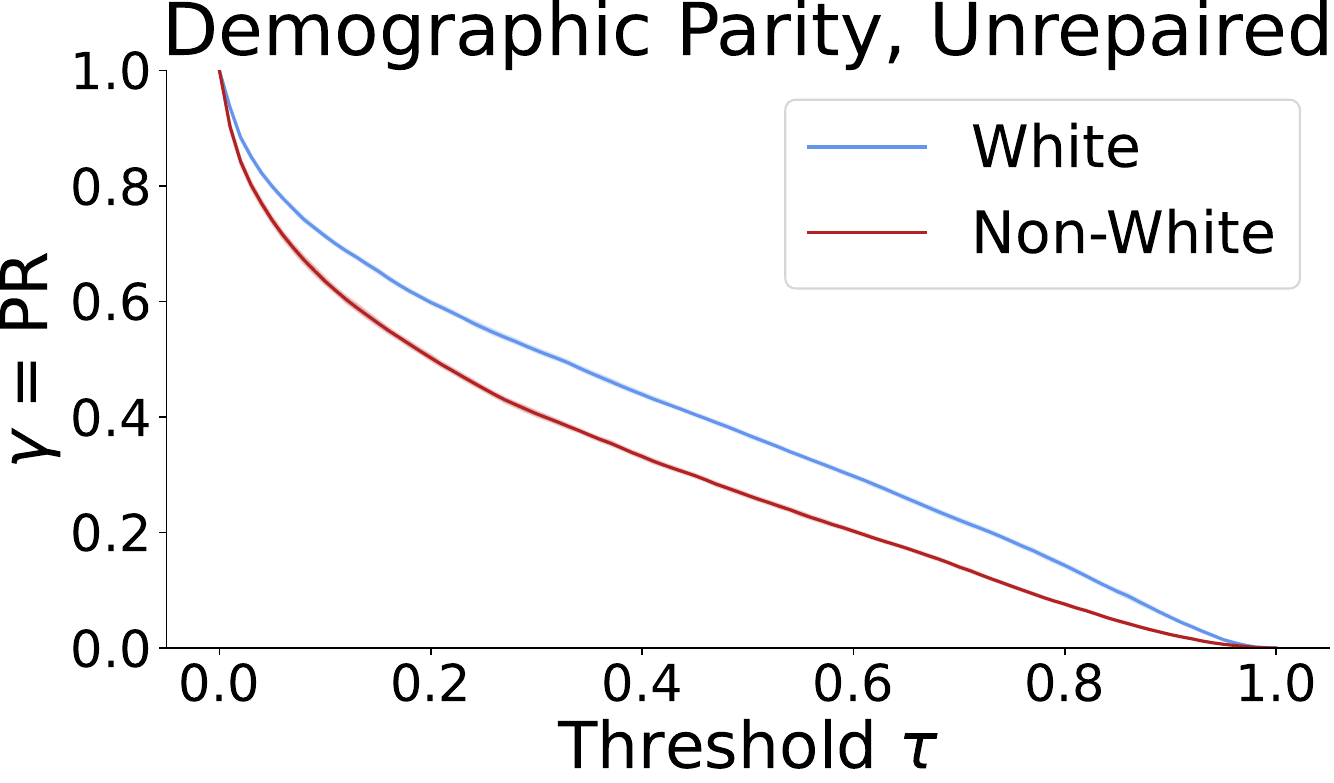}\\
        \includegraphics[width=0.9\linewidth]{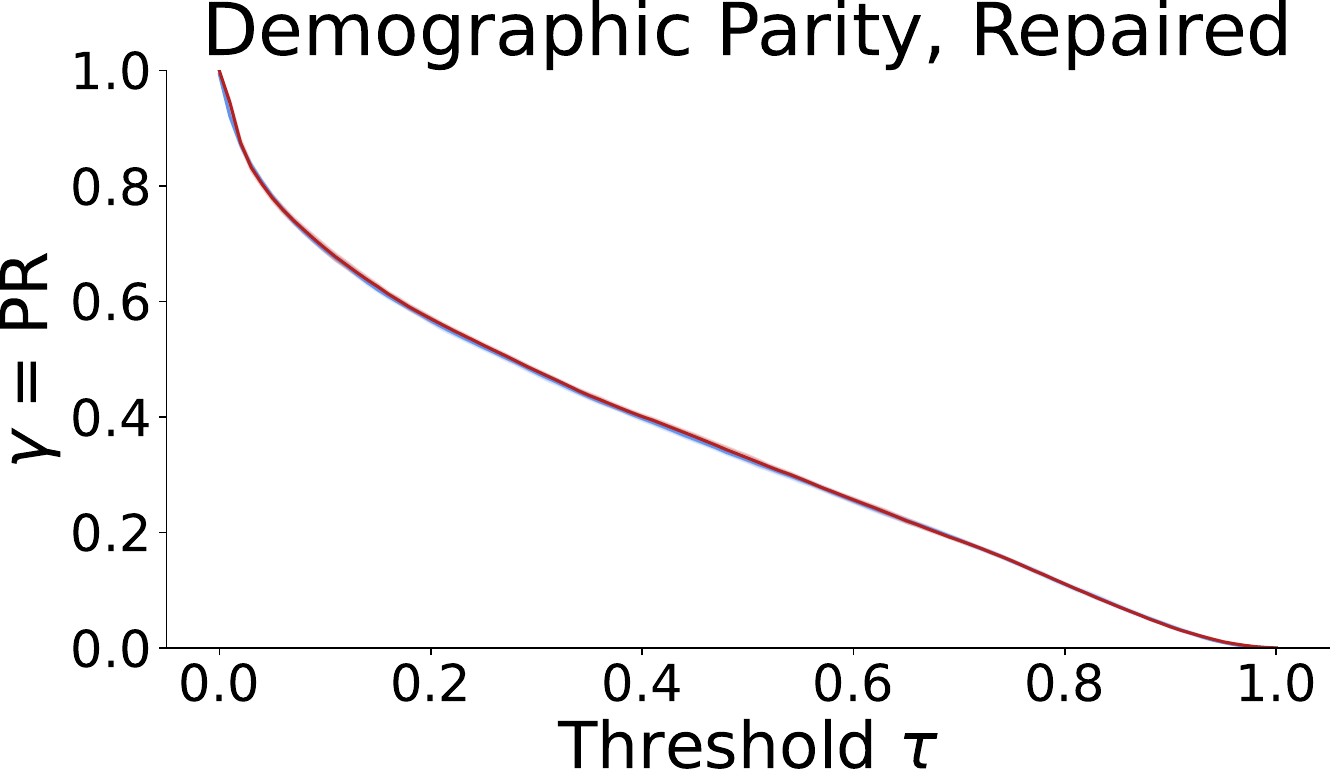}
        \subcaption{Algorithm~\ref{alg:repair} results for SDP}
        \label{fig:app:adult_new_lr-sdp}
    \end{minipage}%
    \begin{minipage}{0.66\textwidth}
        \centering
        \includegraphics[width=0.45\linewidth]{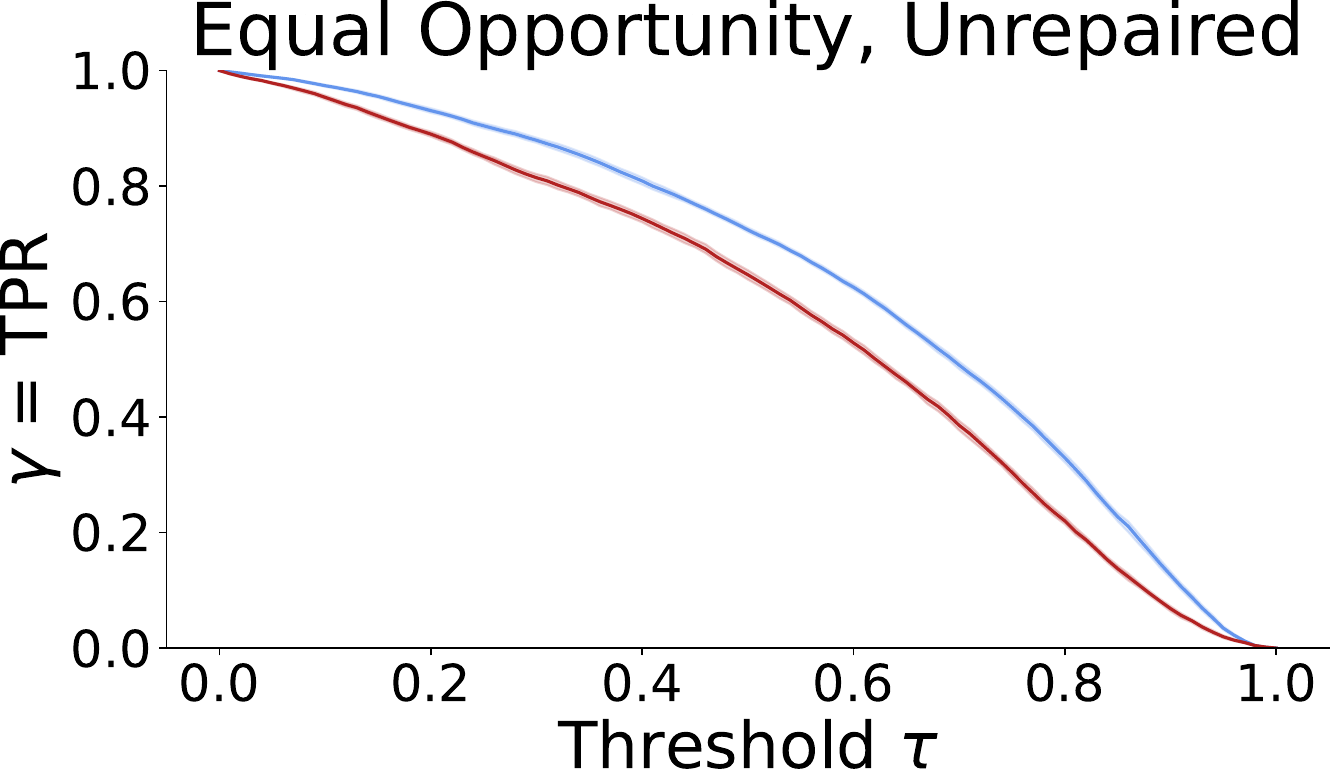}
        \includegraphics[width=0.45\linewidth]{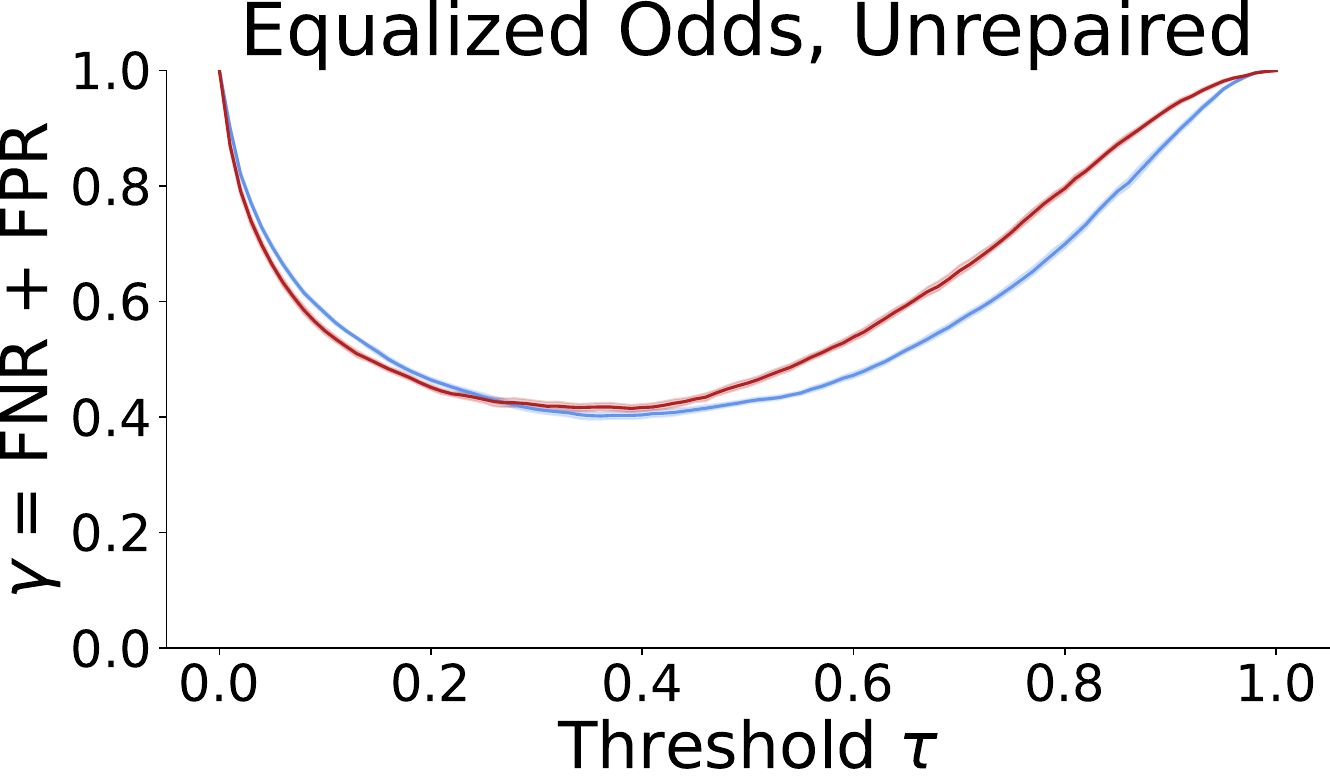}\\
        \includegraphics[width=0.45\linewidth]{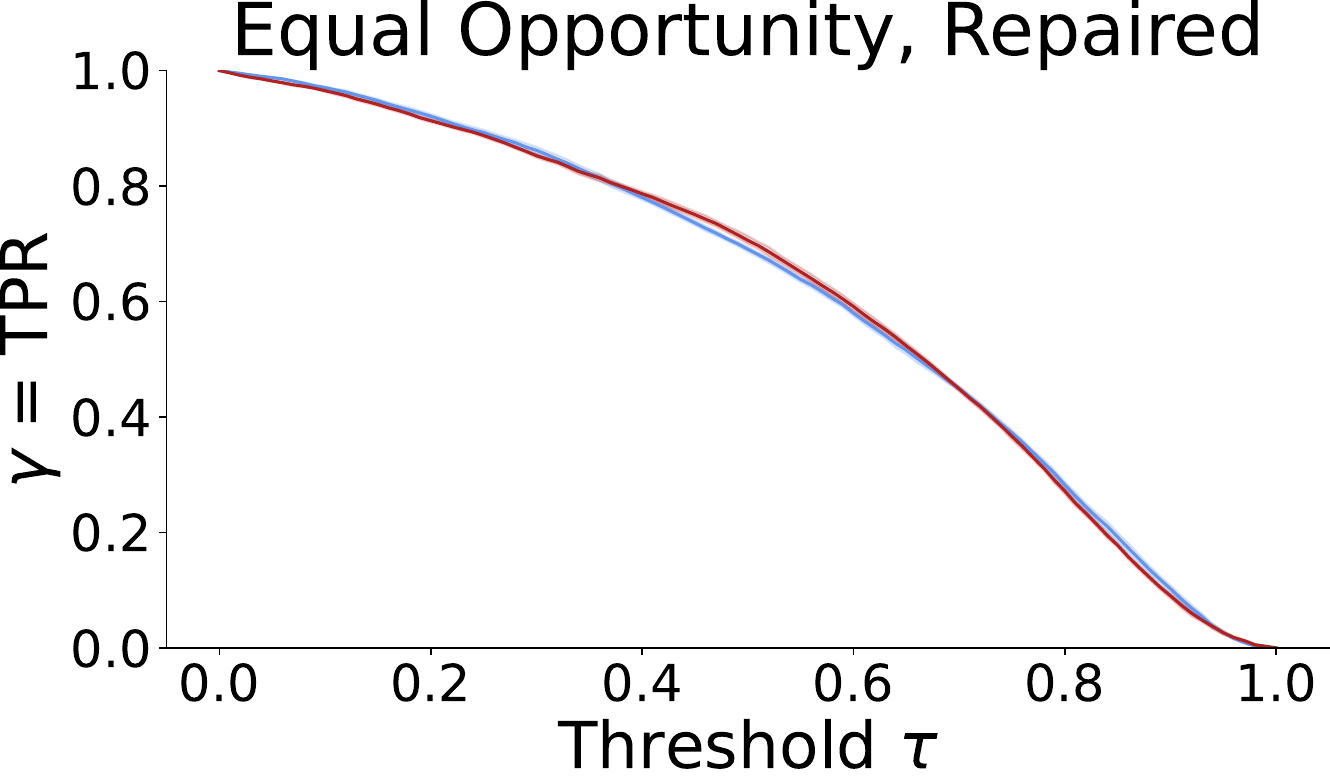}
        \includegraphics[width=0.45\linewidth]{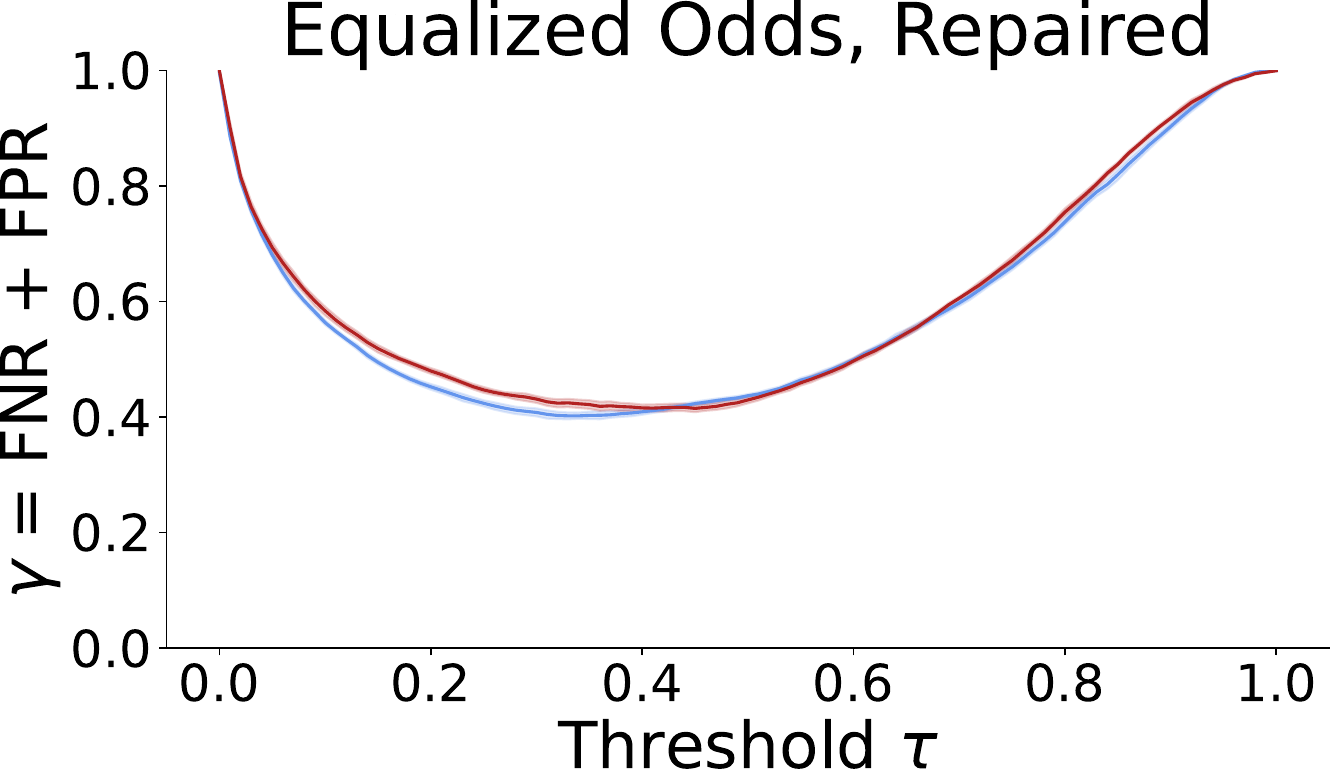}\\
        \subcaption{Algorithm~\ref{alg:repair} results for Eq. Odds and Eq. Opportunity}
        \label{fig:app:adult_new_lr-ours}
    \end{minipage}
    \vspace{-.2cm}
    \caption{Comparing unrepaired and repaired logistic regression on New \texttt{Adult} Income-Race~\citep{ding2021retiring}.} 
    \label{fig:app:adult_new_lr}
    \vspace{-.2cm}
\end{figure*}

\begin{figure*}[!ht]
    \centering
    \begin{minipage}{.33\textwidth}
        \centering
        \includegraphics[width=0.9\linewidth]{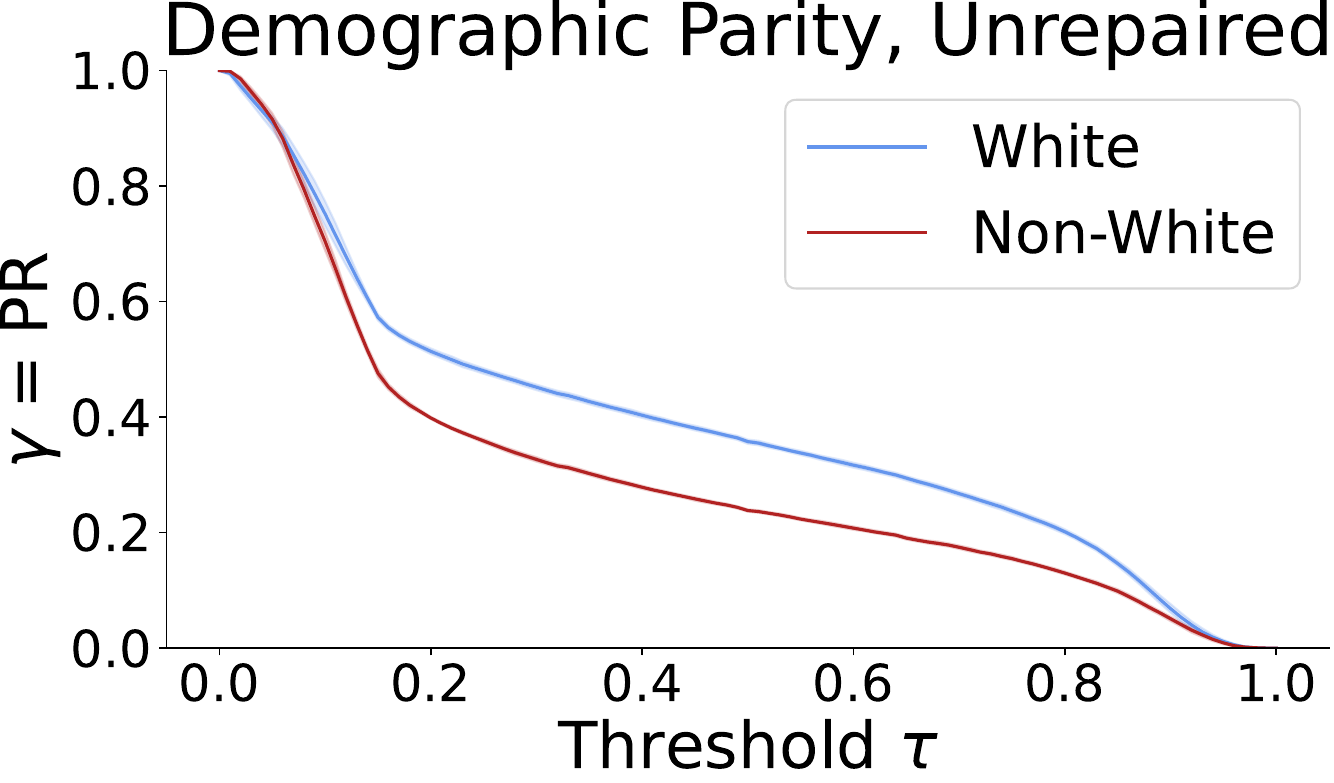}\\
        \includegraphics[width=0.9\linewidth]{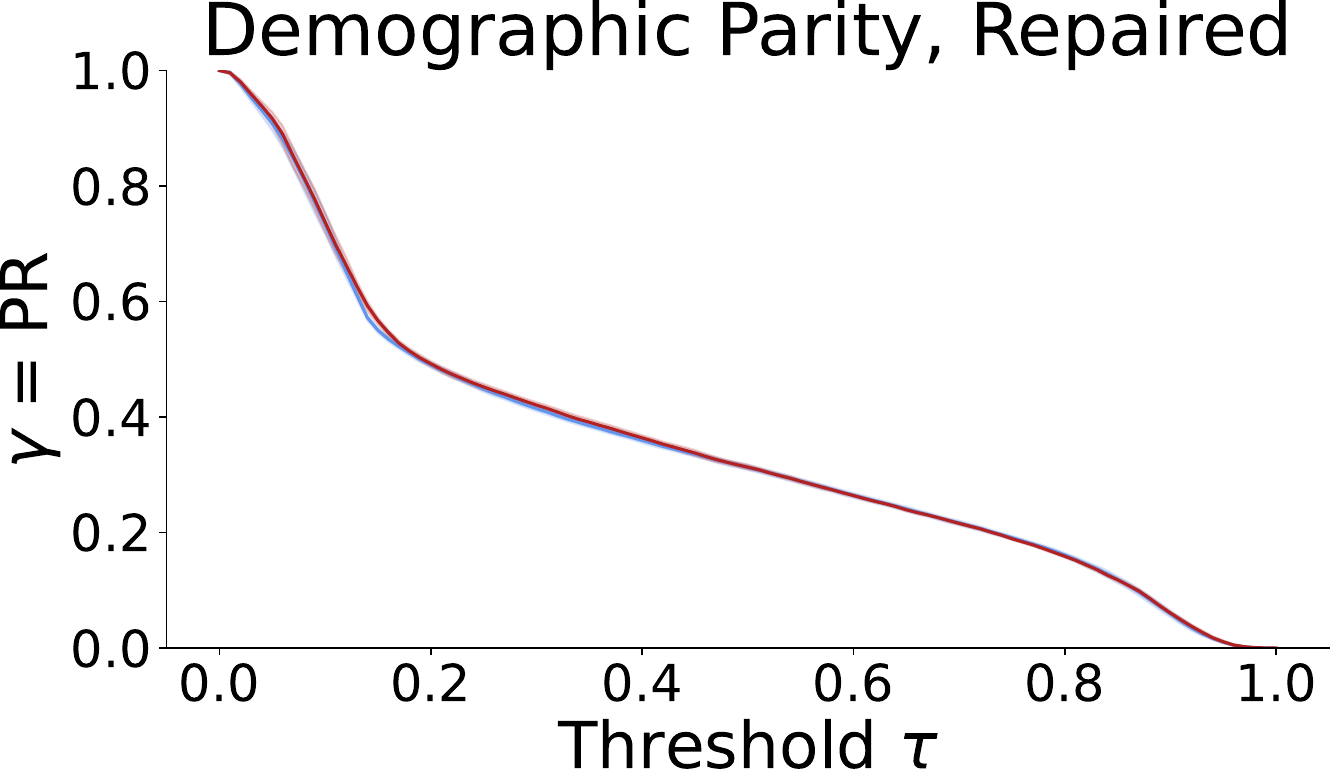}
        \subcaption{Algorithm~\ref{alg:repair} results for SDP}
        \label{fig:app:adult_new_svm-sdp}
    \end{minipage}%
    \begin{minipage}{0.66\textwidth}
        \centering
        \includegraphics[width=0.45\linewidth]{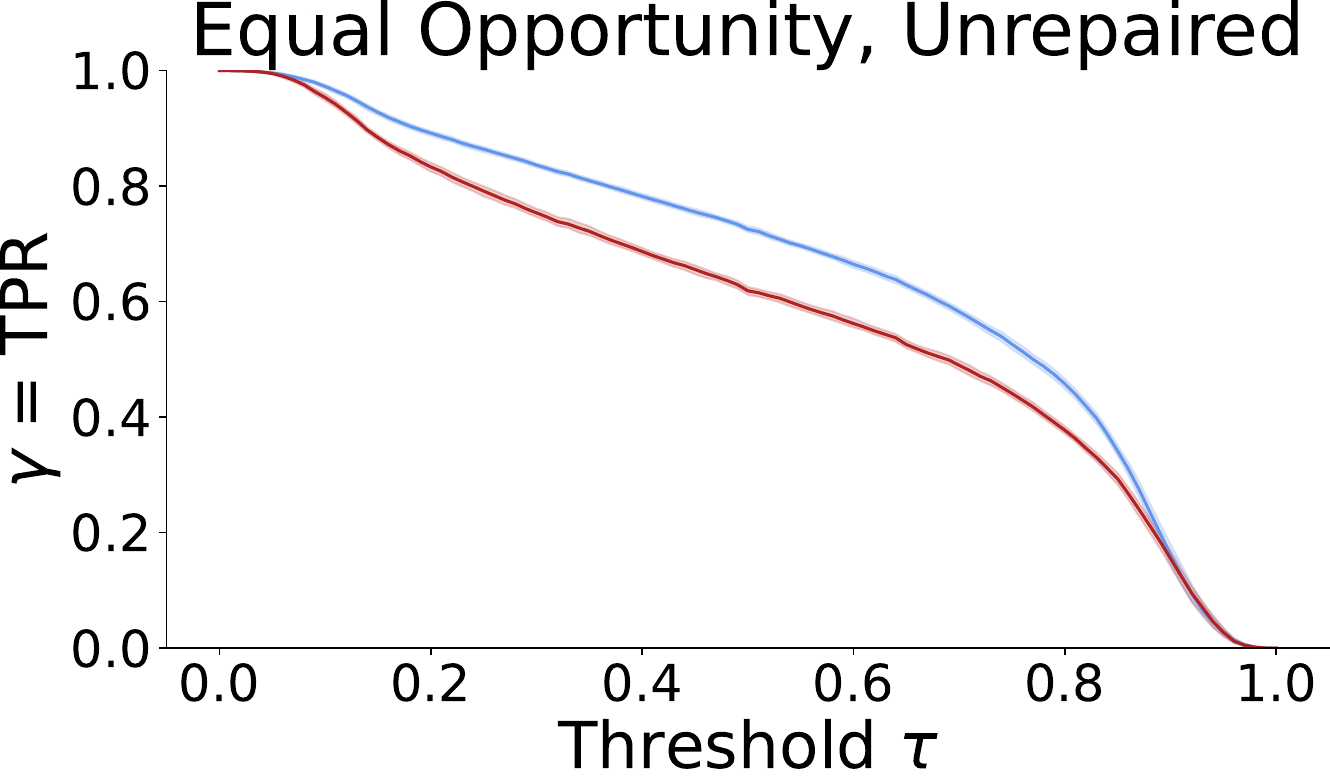}
        \includegraphics[width=0.45\linewidth]{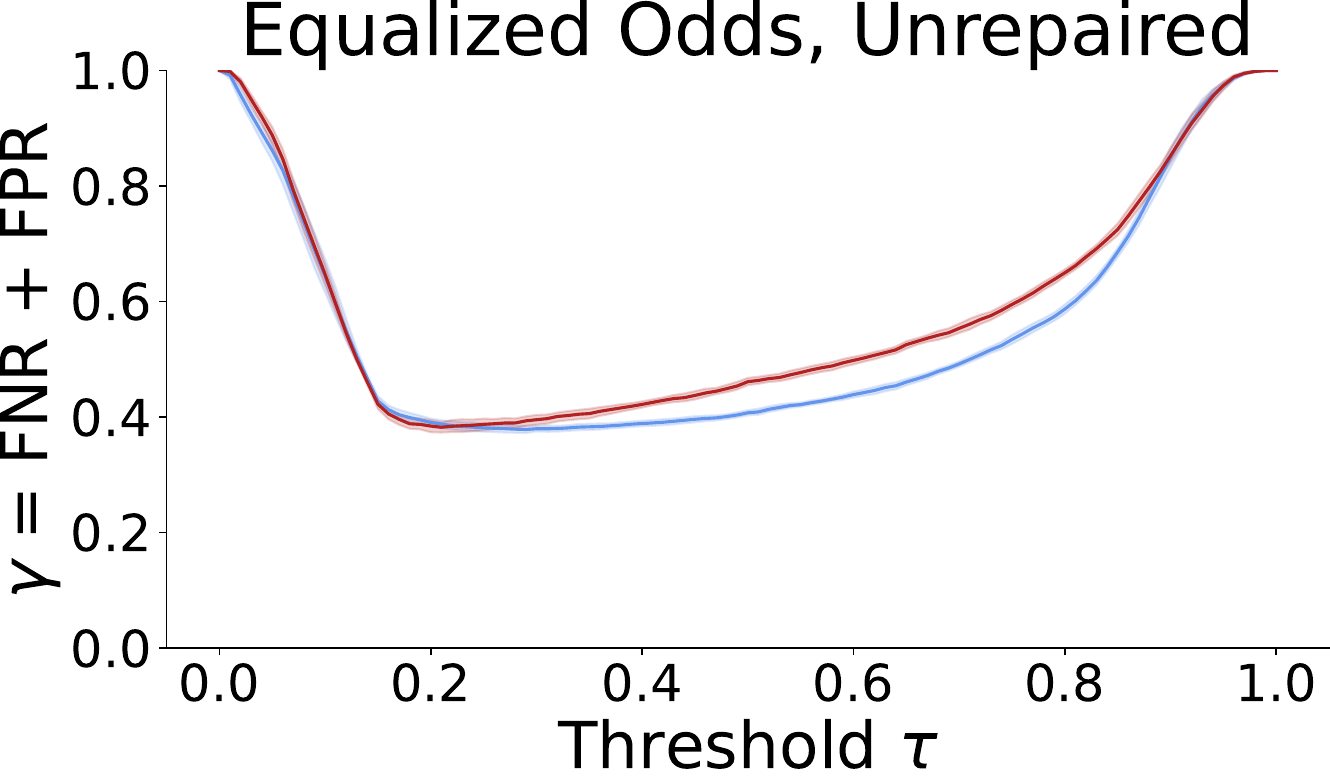}\\
        \includegraphics[width=0.45\linewidth]{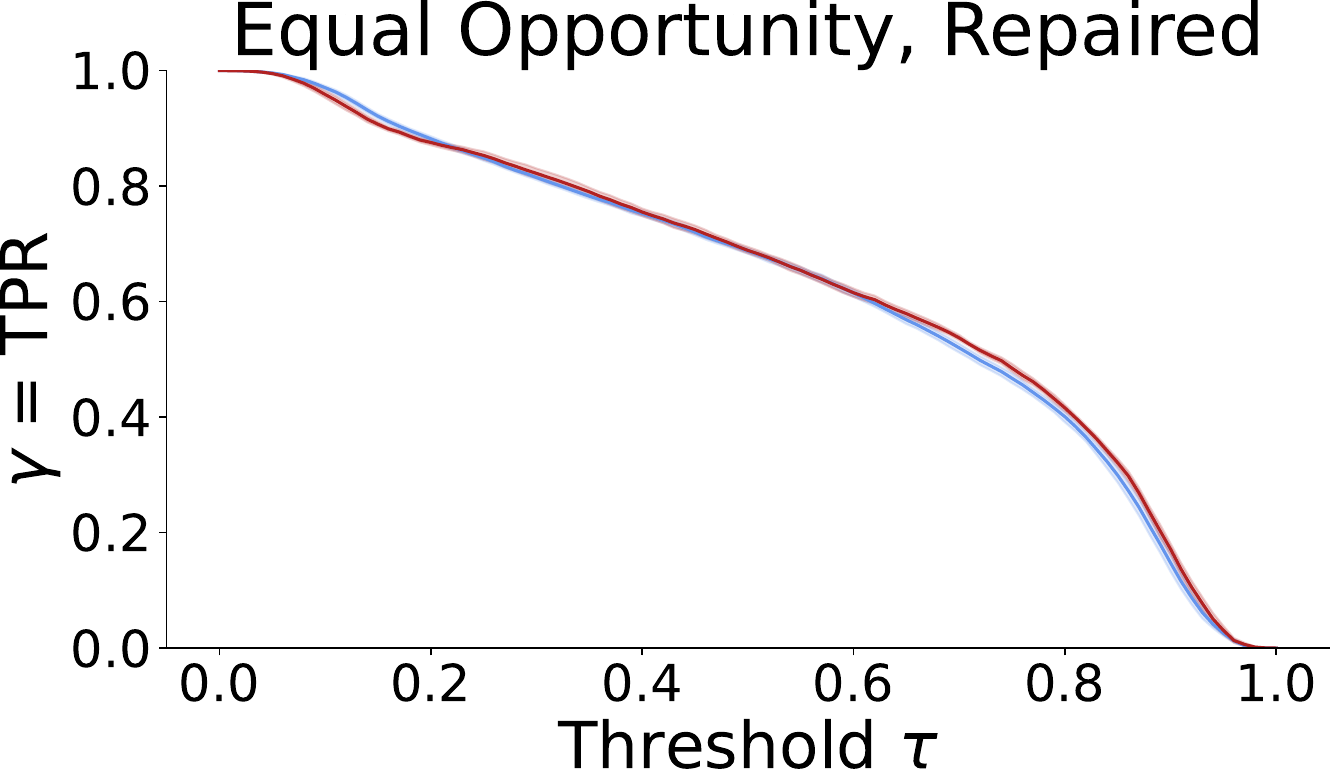}
        \includegraphics[width=0.45\linewidth]{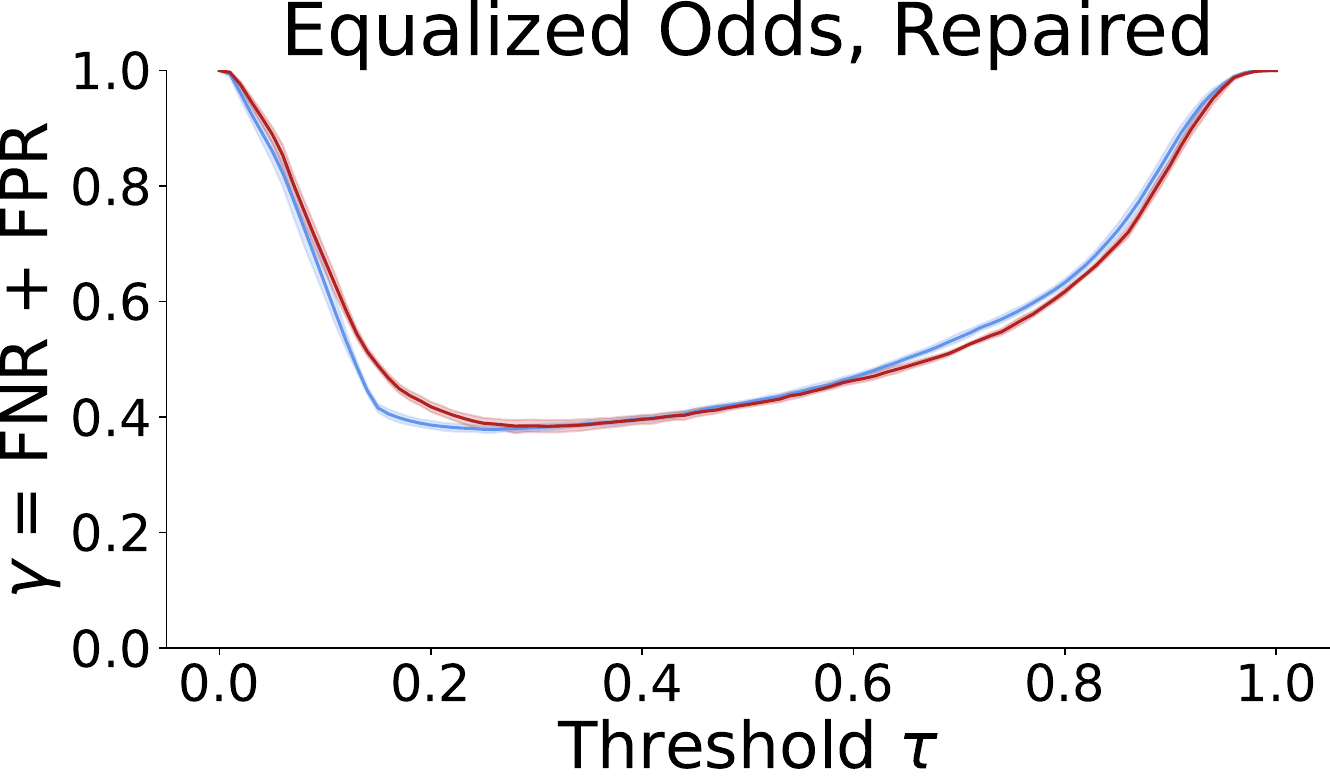}\\
        \subcaption{Algorithm~\ref{alg:repair} results for Eq. Odds and Eq. Opportunity}
        \label{fig:app:adult_new_svm-ours}
    \end{minipage}
    \vspace{-.2cm}
    \caption{Comparing unrepaired and repaired SVMs on New \texttt{Adult} Income-Race~\citep{ding2021retiring}.} 
    \label{fig:app:adult_new_svm}
    \vspace{-.2cm}
\end{figure*}

\begin{figure*}[!ht]
    \centering
    \begin{minipage}{.33\textwidth}
        \centering
        \includegraphics[width=0.9\linewidth]{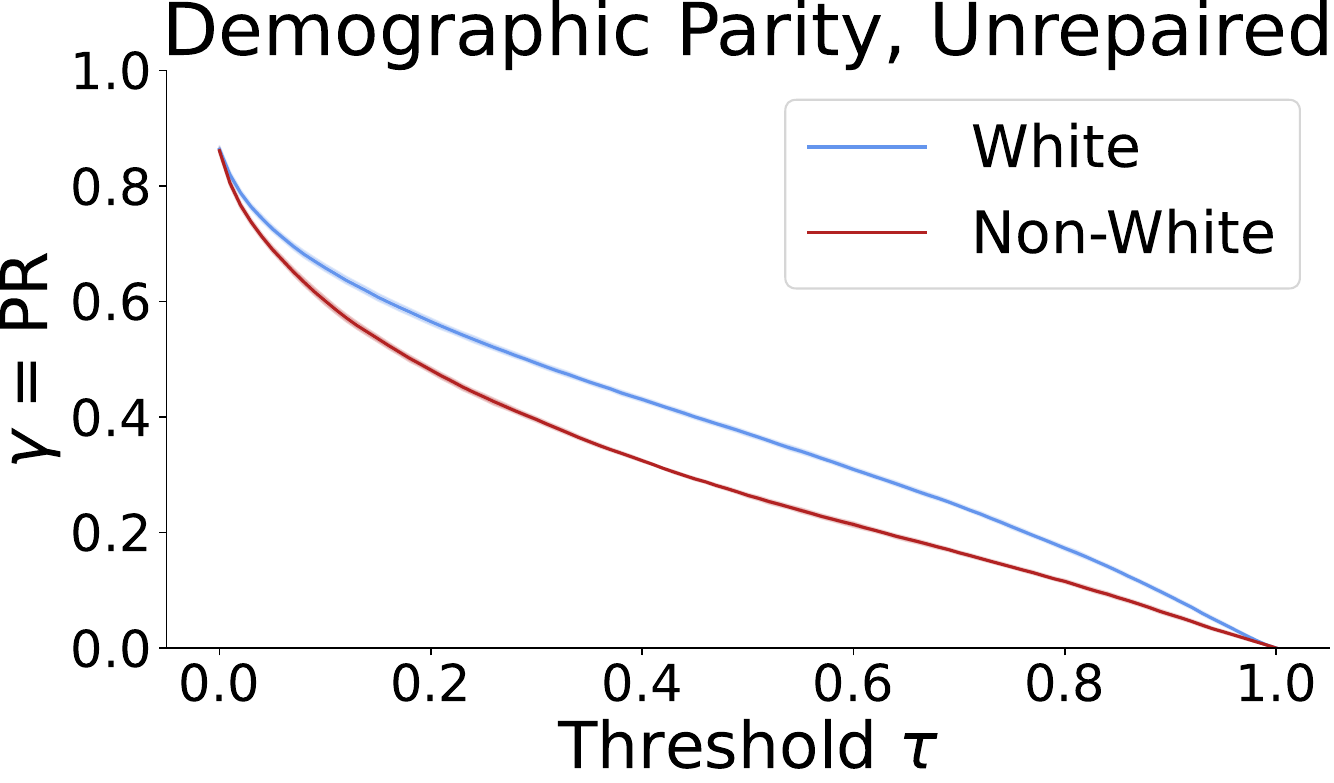}\\
        \includegraphics[width=0.9\linewidth]{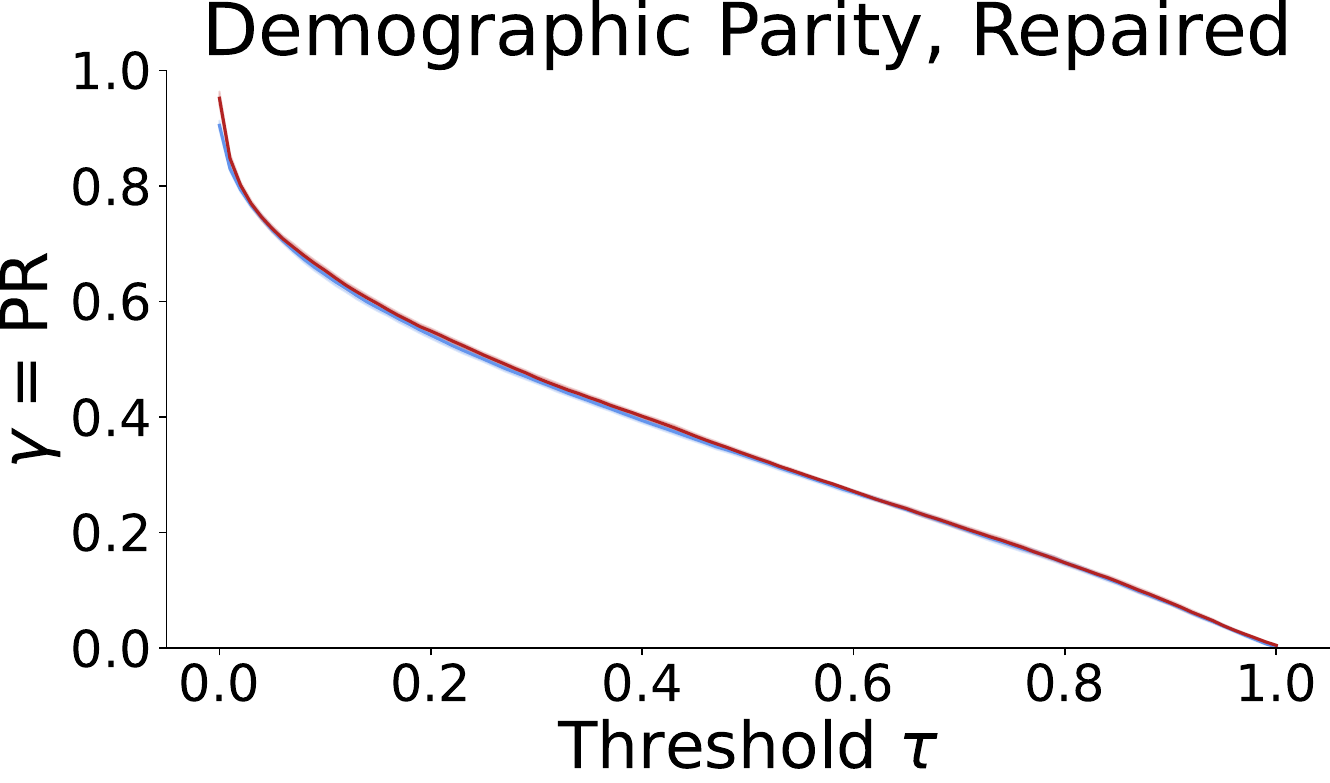}
        \subcaption{Algorithm~\ref{alg:repair} results for SDP}
        \label{fig:app:adult_new_rf-sdp}
    \end{minipage}%
    \begin{minipage}{0.66\textwidth}
        \centering
        \includegraphics[width=0.45\linewidth]{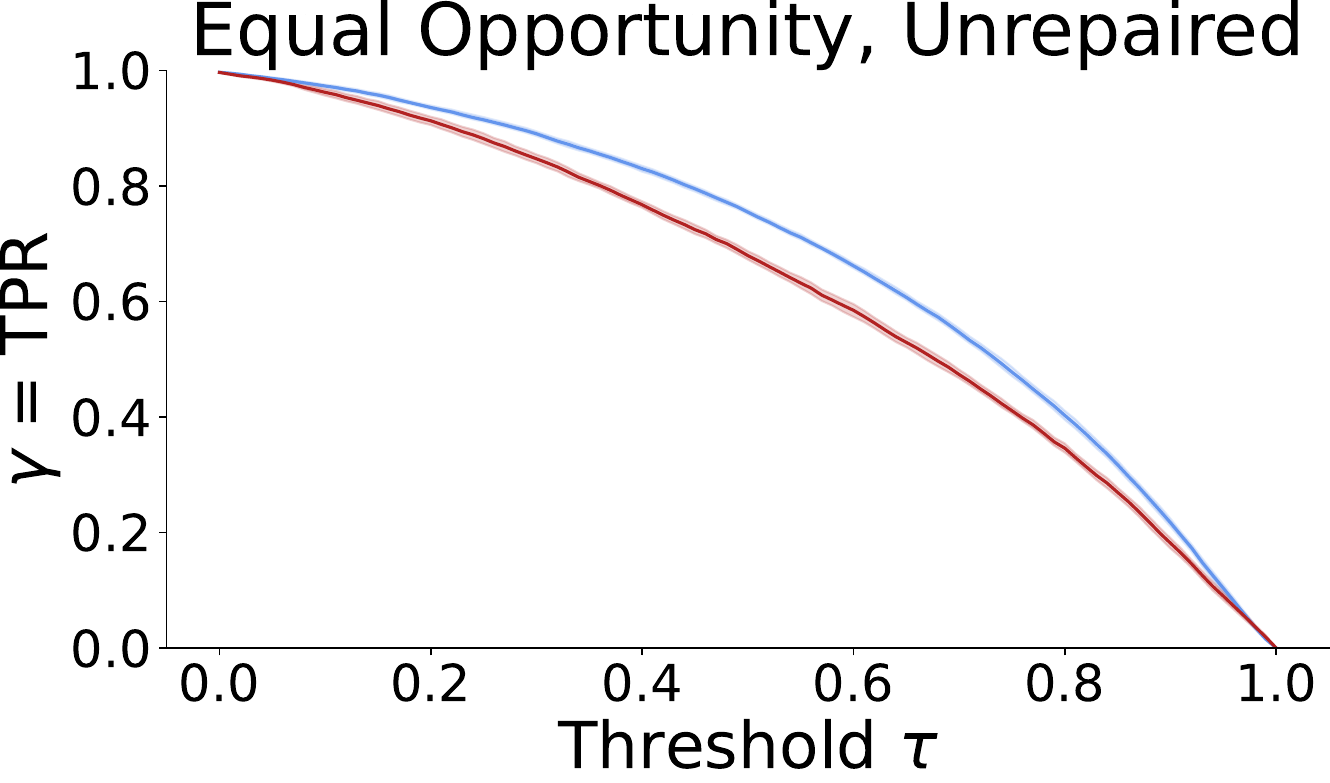}
        \includegraphics[width=0.45\linewidth]{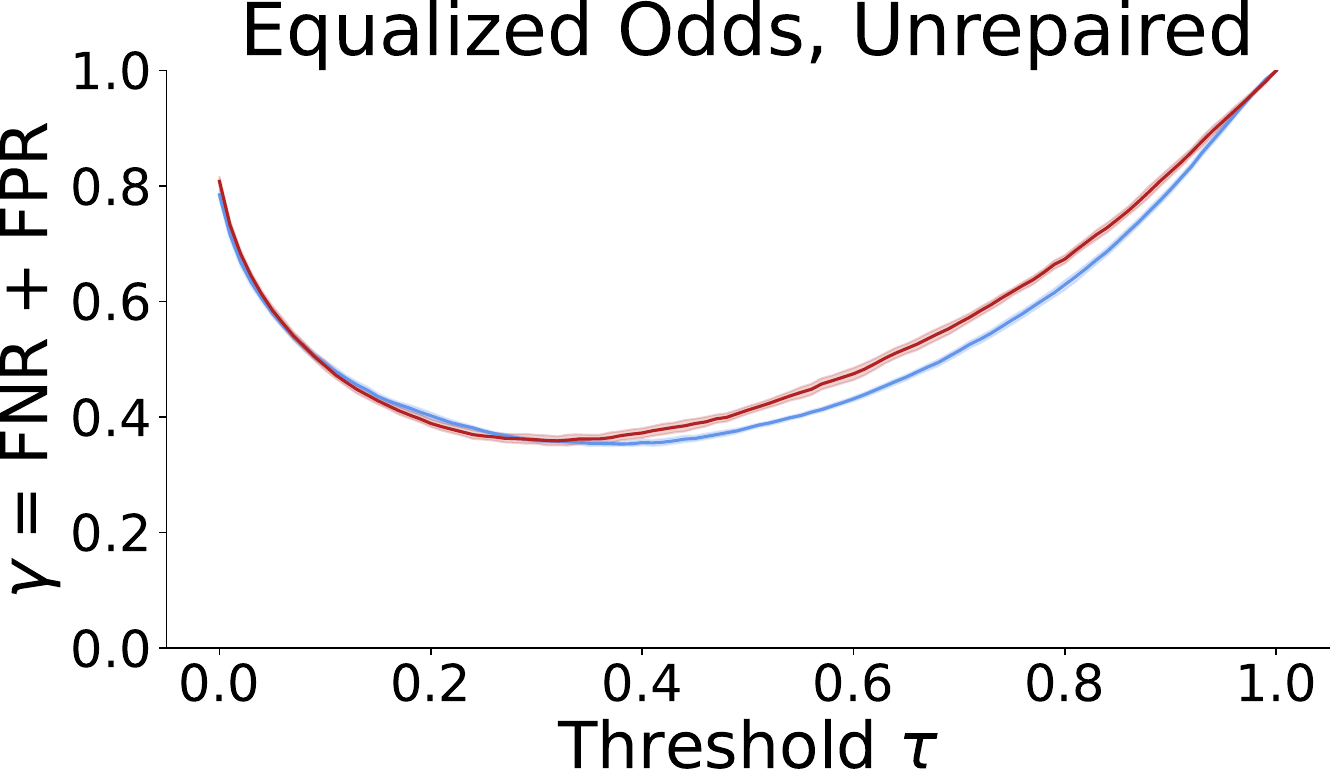}\\
        \includegraphics[width=0.45\linewidth]{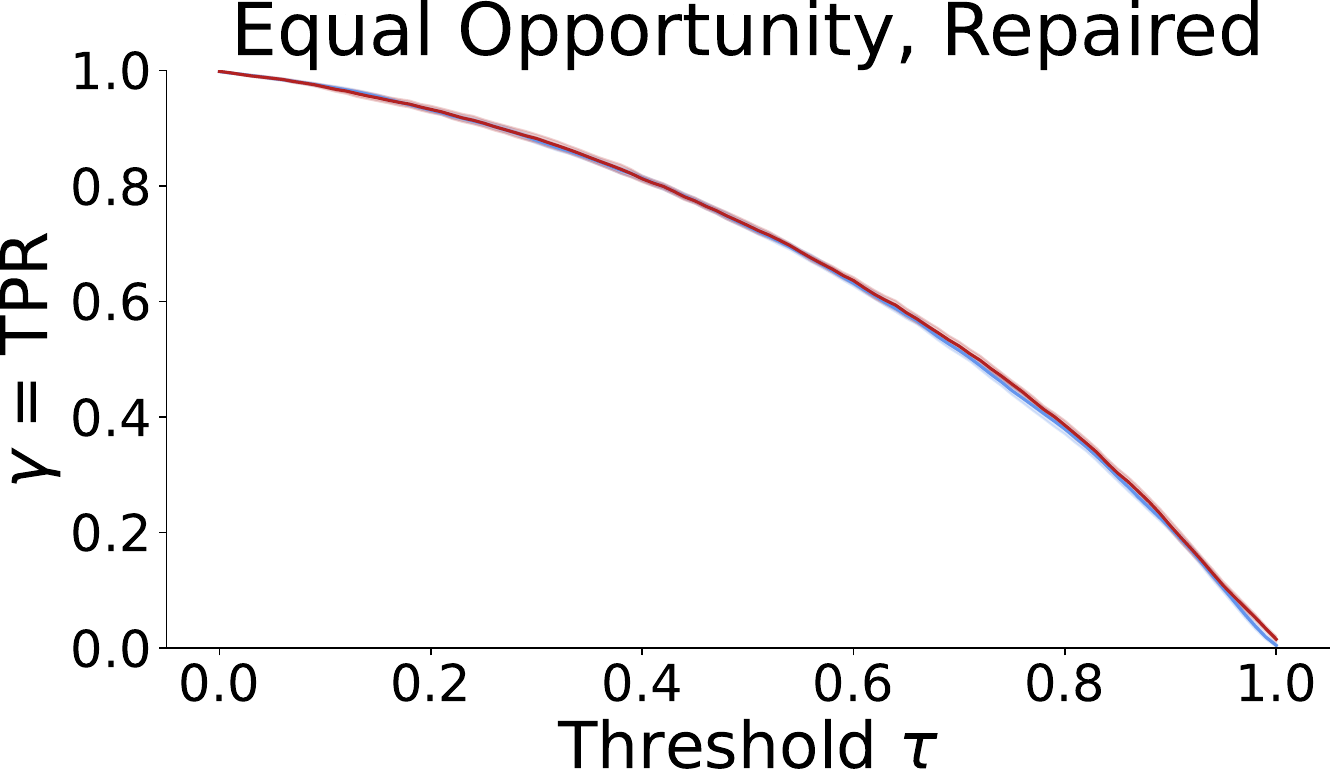}
        \includegraphics[width=0.45\linewidth]{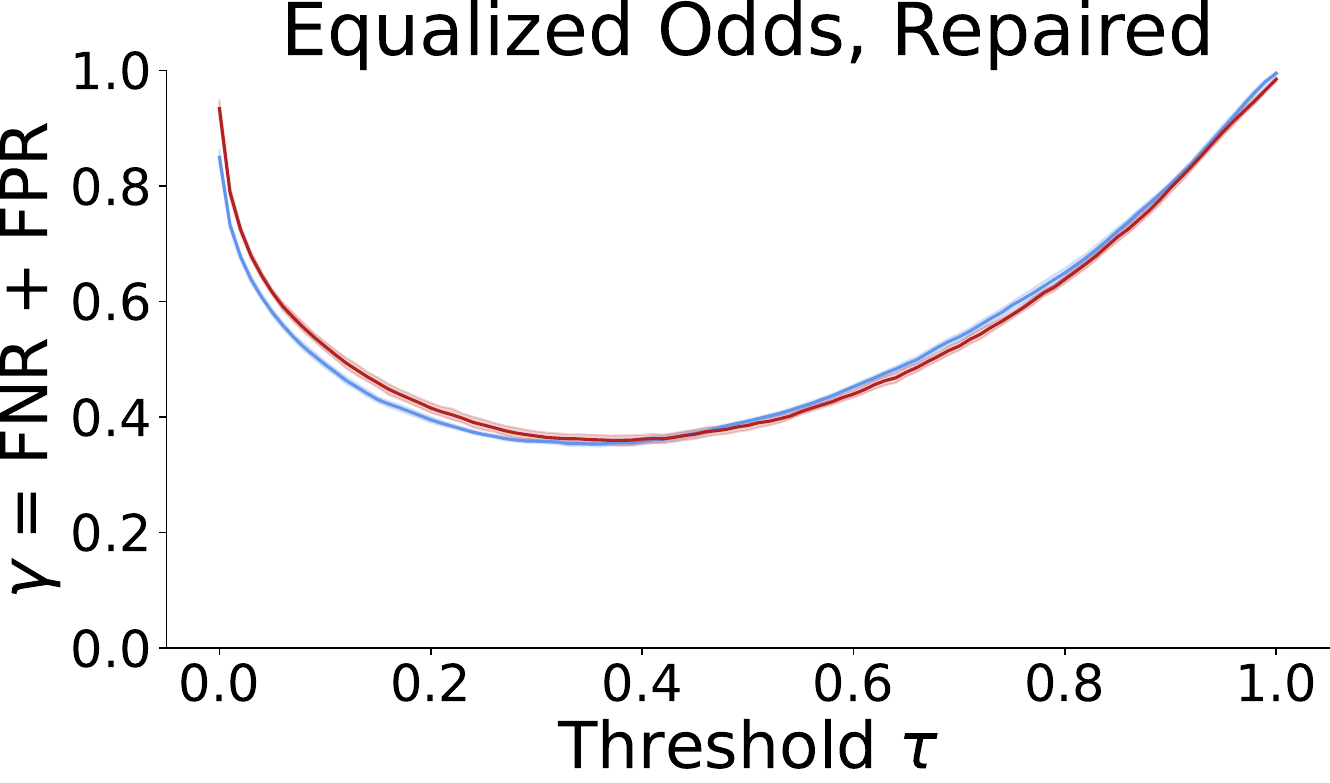}\\
        \subcaption{Algorithm~\ref{alg:repair} results for Eq. Odds and Eq. Opportunity}
        \label{fig:app:adult_new_rf-ours}
    \end{minipage}
    \vspace{-.2cm}
    \caption{Comparing unrepaired and repaired Random Forests on New \texttt{Adult} Income-Race~\citep{ding2021retiring}.} 
    \label{fig:app:adult_new_rf}
    \vspace{-.2cm}
\end{figure*}

\begin{figure*}[!ht]
    \centering
    \begin{minipage}{.33\textwidth}
        \centering
        \includegraphics[width=0.9\linewidth]{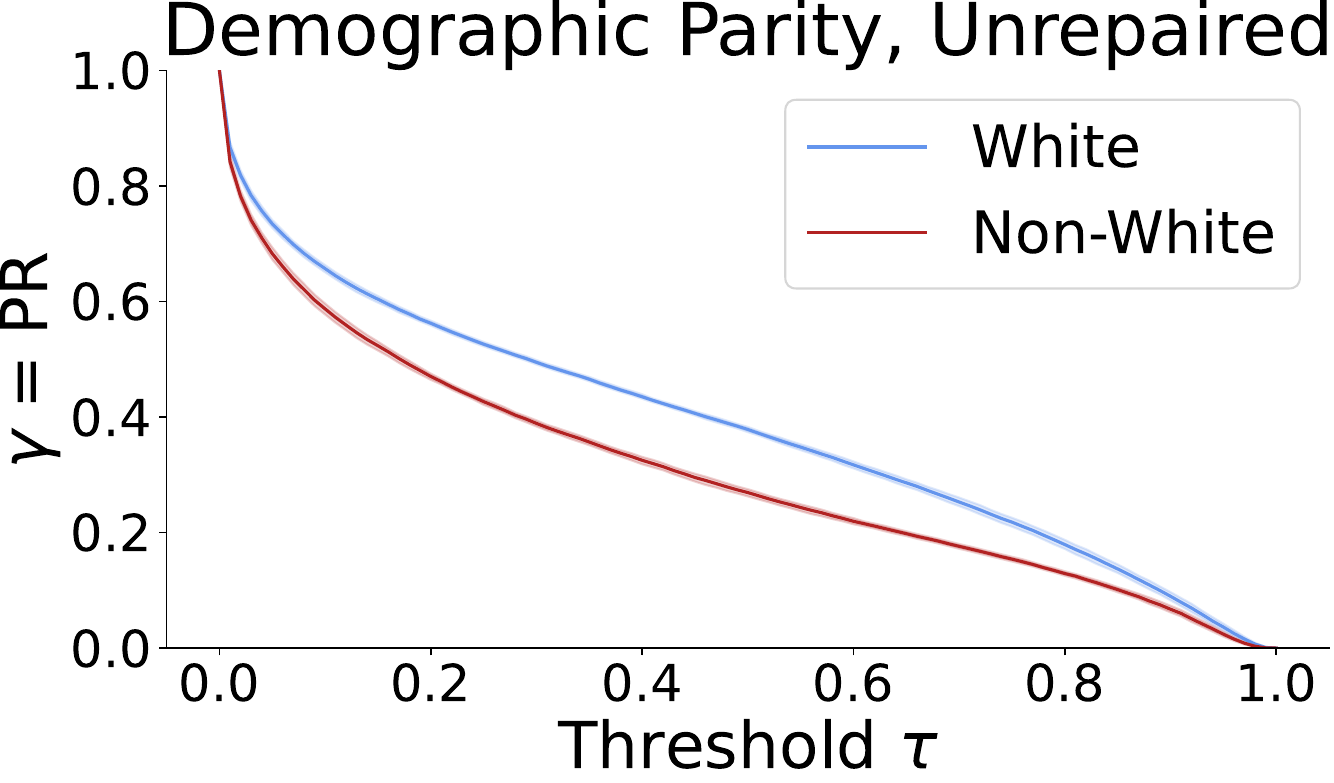}\\
        \includegraphics[width=0.9\linewidth]{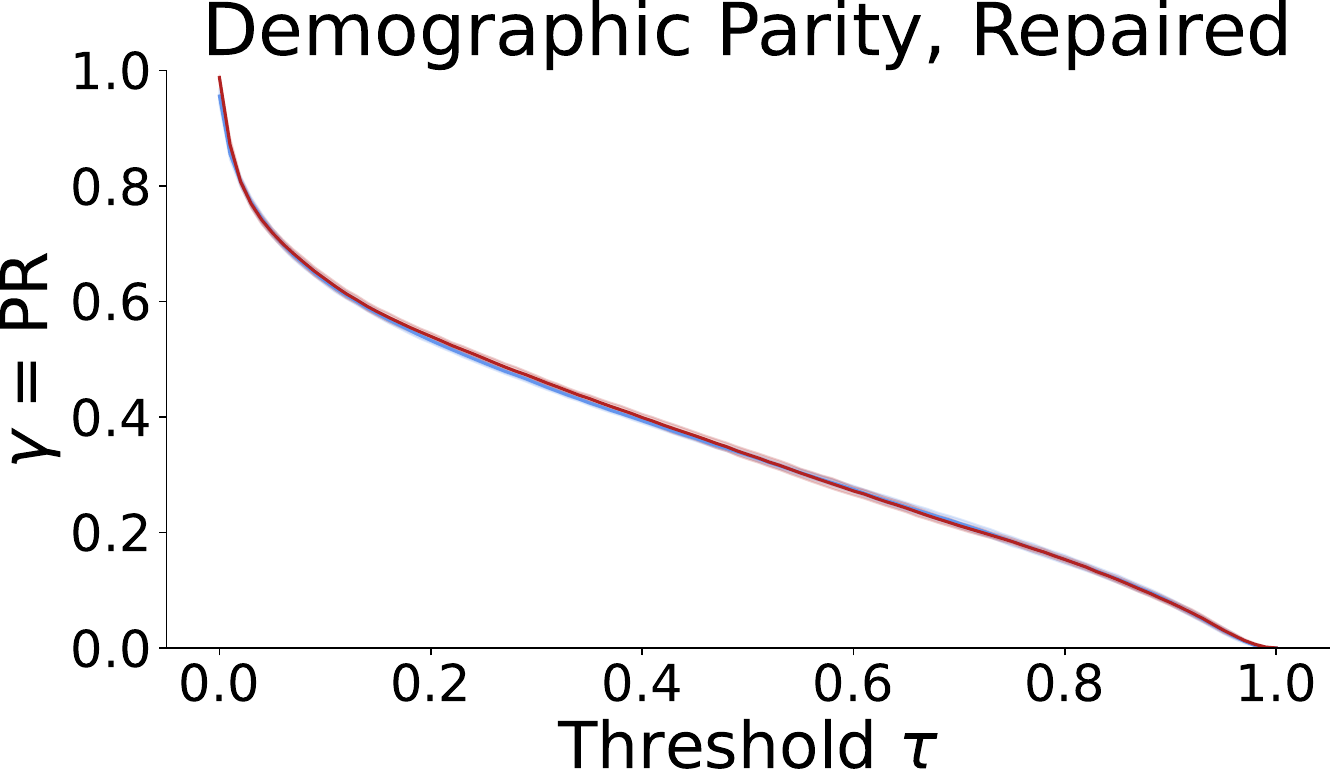}
        \subcaption{Algorithm~\ref{alg:repair} results for SDP}
        \label{fig:app:adult_new_mlp-sdp}
    \end{minipage}%
    \begin{minipage}{0.66\textwidth}
        \centering
        \includegraphics[width=0.45\linewidth]{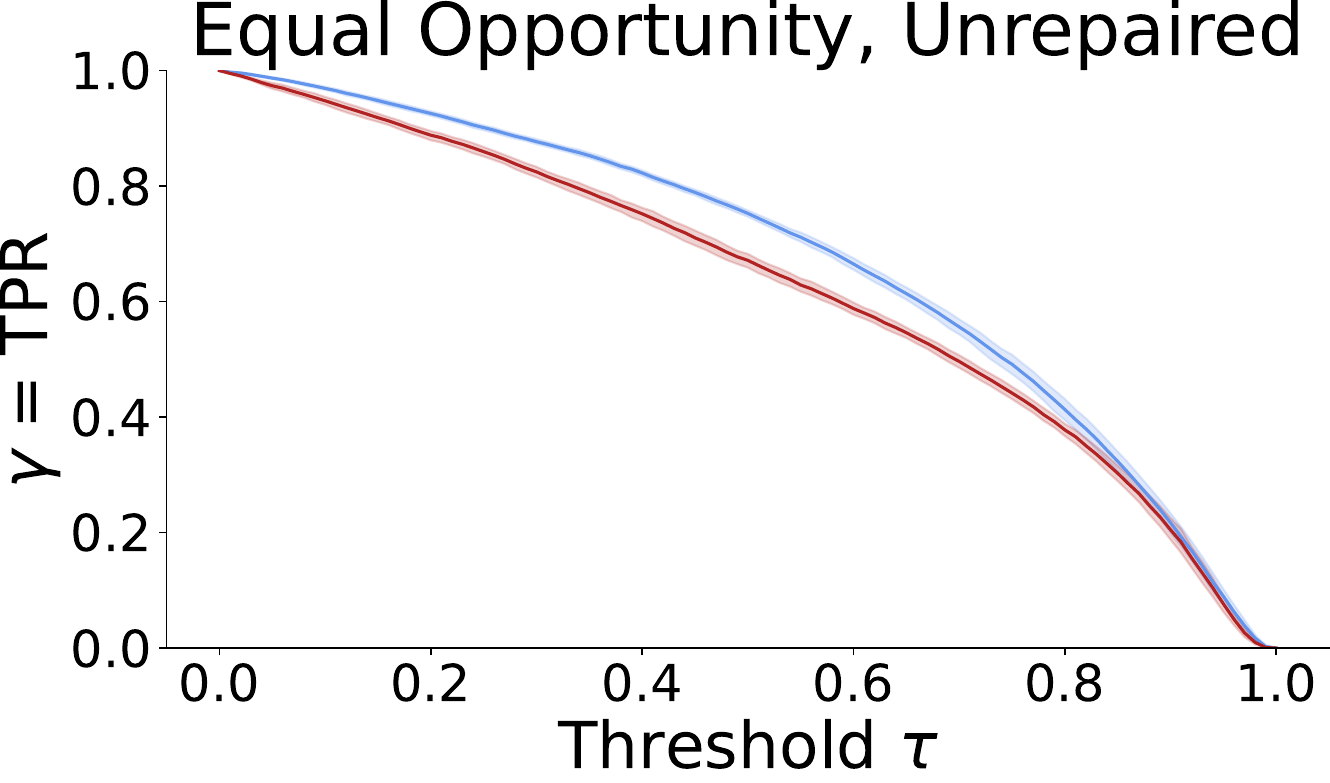}
        \includegraphics[width=0.45\linewidth]{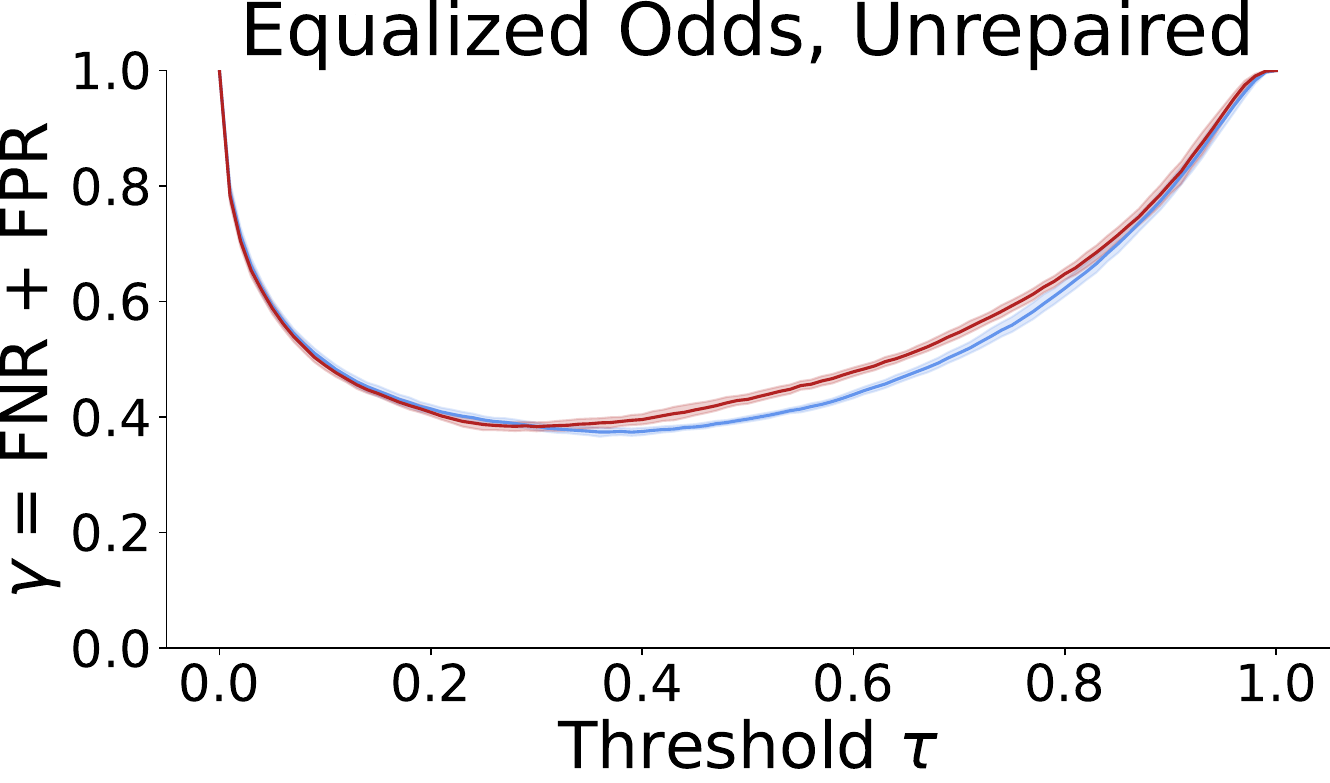}\\
        \includegraphics[width=0.45\linewidth]{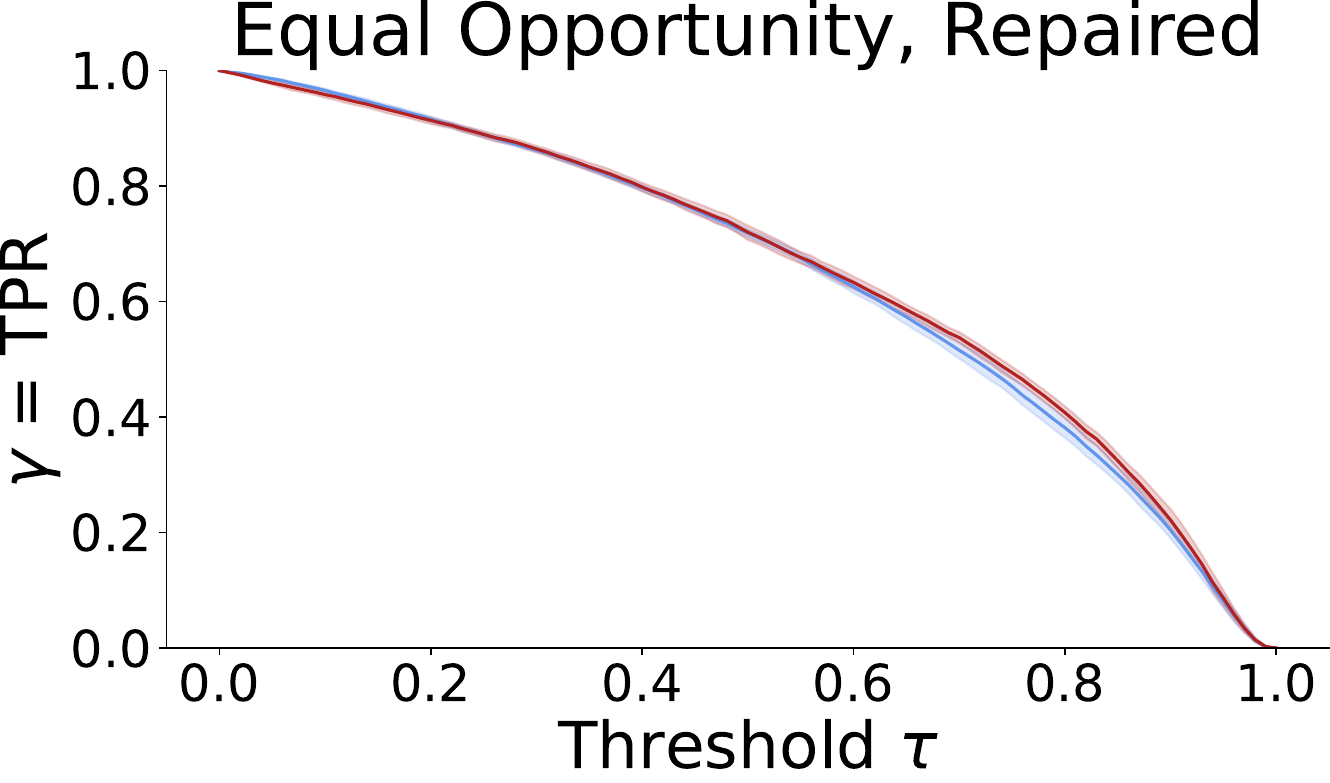}
        \includegraphics[width=0.45\linewidth]{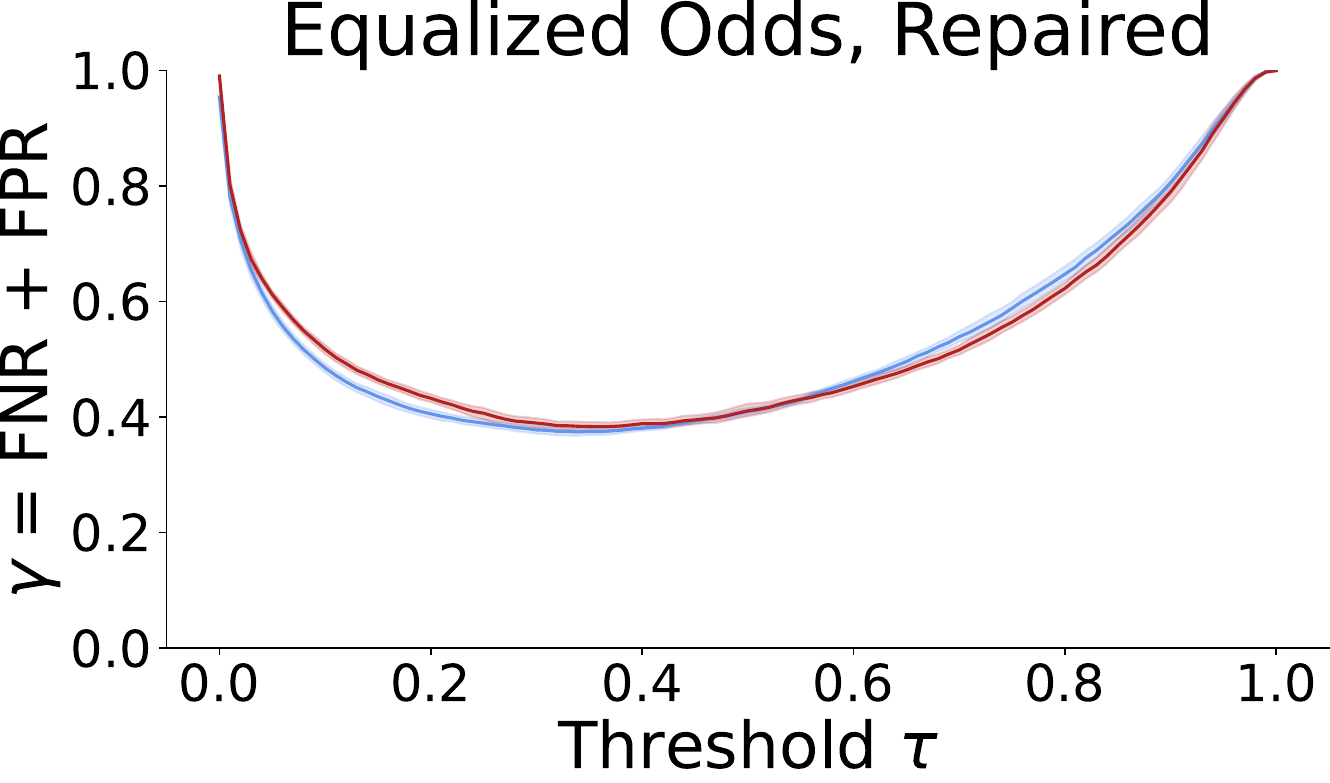}\\
        \subcaption{Algorithm~\ref{alg:repair} results for Eq. Odds and Eq. Opportunity}
        \label{fig:app:adult_new_mlp-ours}
    \end{minipage}
    \vspace{-.2cm}
    \caption{Comparing unrepaired and repaired MLPs on New \texttt{Adult} Income-Race~\citep{ding2021retiring}.} 
    \label{fig:app:adult_new_mlp}
    \vspace{-.2cm}
\end{figure*}

% \subsubsection{Additional Results for New \texttt{Adult} \citep{ding2021retiring}, Public Coverage task}

% \begin{figure*}[!ht]
%     \centering
%     \begin{minipage}{.33\textwidth}
%         \centering
%         \includegraphics[width=0.9\linewidth]{figures_appendix/public_lr_selection_lmbd=orig.pdf}\\
%         \includegraphics[width=0.9\linewidth]{figures_appendix/public_lr_selection_lmbd=full.pdf}
%         \subcaption{Algorithm~\ref{alg:repair} results for SDP}
%         \label{fig:app:public_lr-sdp}
%     \end{minipage}%
%     \begin{minipage}{0.66\textwidth}
%         \centering
%         \includegraphics[width=0.45\linewidth]{figures_appendix/public_lr_tpr_lmbd=orig.pdf}
%         \includegraphics[width=0.45\linewidth]{figures_appendix/public_lr_eqodds_lmbd=orig.pdf}\\
%         \includegraphics[width=0.45\linewidth]{figures_appendix/public_lr_tpr_lmbd=tpr.pdf}
%         \includegraphics[width=0.45\linewidth]{figures_appendix/public_lr_eqodds_lmbd=eo_1.pdf}\\
%         \subcaption{Algorithm~\ref{alg:repair} results for Eq. Odds and Eq. Opportunity}
%         \label{fig:app:public_lr-ours}
%     \end{minipage}
%     \vspace{-.2cm}
%     \caption{Comparing unrepaired and repaired logistic regression on New \texttt{Adult} \citep{ding2021retiring}, Public Coverage.} 
%     \label{fig:app:public_lr}
%     \vspace{-.2cm}
% \end{figure*}

% \begin{figure*}[!ht]
%     \centering
%     \begin{minipage}{.33\textwidth}
%         \centering
%         \includegraphics[width=0.9\linewidth]{figures_appendix/public_svm_selection_lmbd=orig.pdf}\\
%         \includegraphics[width=0.9\linewidth]{figures_appendix/public_svm_selection_lmbd=full.pdf}
%         \subcaption{Algorithm~\ref{alg:repair} results for SDP}
%         \label{fig:app:public_svm-sdp}
%     \end{minipage}%
%     \begin{minipage}{0.66\textwidth}
%         \centering
%         \includegraphics[width=0.45\linewidth]{figures_appendix/public_svm_tpr_lmbd=orig.pdf}
%         \includegraphics[width=0.45\linewidth]{figures_appendix/public_svm_eqodds_lmbd=orig.pdf}\\
%         \includegraphics[width=0.45\linewidth]{figures_appendix/public_svm_tpr_lmbd=tpr.pdf}
%         \includegraphics[width=0.45\linewidth]{figures_appendix/public_svm_eqodds_lmbd=eo_1.pdf}\\
%         \subcaption{Algorithm~\ref{alg:repair} results for Eq. Odds and Eq. Opportunity}
%         \label{fig:app:public_svm-ours}
%     \end{minipage}
%     \vspace{-.2cm}
%     \caption{Comparing unrepaired and repaired SVMs on New \texttt{Adult} \citep{ding2021retiring}, Public Coverage.} 
%     \label{fig:app:public_svm}
%     \vspace{-.2cm}
% \end{figure*}

% \begin{figure*}[!ht]
%     \centering
%     \begin{minipage}{.33\textwidth}
%         \centering
%         \includegraphics[width=0.9\linewidth]{figures_appendix/public_rf_selection_lmbd=orig.pdf}\\
%         \includegraphics[width=0.9\linewidth]{figures_appendix/public_rf_selection_lmbd=full.pdf}
%         \subcaption{Algorithm~\ref{alg:repair} results for SDP}
%         \label{fig:app:public_rf-sdp}
%     \end{minipage}%
%     \begin{minipage}{0.66\textwidth}
%         \centering
%         \includegraphics[width=0.45\linewidth]{figures_appendix/public_rf_tpr_lmbd=orig.pdf}
%         \includegraphics[width=0.45\linewidth]{figures_appendix/public_rf_eqodds_lmbd=orig.pdf}\\
%         \includegraphics[width=0.45\linewidth]{figures_appendix/public_rf_tpr_lmbd=tpr.pdf}
%         \includegraphics[width=0.45\linewidth]{figures_appendix/public_rf_eqodds_lmbd=eo_1.pdf}\\
%         \subcaption{Algorithm~\ref{alg:repair} results for Eq. Odds and Eq. Opportunity}
%         \label{fig:app:public_rf-ours}
%     \end{minipage}
%     \vspace{-.2cm}
%     \caption{Comparing unrepaired and repaired Random Forests on New \texttt{Adult} \citep{ding2021retiring}, Public Coverage.} 
%     \label{fig:app:public_rf}
%     \vspace{-.2cm}
% \end{figure*}

% \begin{figure*}[!ht]
%     \centering
%     \begin{minipage}{.33\textwidth}
%         \centering
%         \includegraphics[width=0.9\linewidth]{figures_appendix/public_mlp_selection_lmbd=orig.pdf}\\
%         \includegraphics[width=0.9\linewidth]{figures_appendix/public_mlp_selection_lmbd=full.pdf}
%         \subcaption{Algorithm~\ref{alg:repair} results for SDP}
%         \label{fig:app:public_mlp-sdp}
%     \end{minipage}%
%     \begin{minipage}{0.66\textwidth}
%         \centering
%         \includegraphics[width=0.45\linewidth]{figures_appendix/public_mlp_tpr_lmbd=orig.pdf}
%         \includegraphics[width=0.45\linewidth]{figures_appendix/public_mlp_eqodds_lmbd=orig.pdf}\\
%         \includegraphics[width=0.45\linewidth]{figures_appendix/public_mlp_tpr_lmbd=tpr.pdf}
%         \includegraphics[width=0.45\linewidth]{figures_appendix/public_mlp_eqodds_lmbd=eo_1.pdf}\\
%         \subcaption{Algorithm~\ref{alg:repair} results for Eq. Odds and Eq. Opportunity}
%         \label{fig:app:public_mlp-ours}
%     \end{minipage}
%     \vspace{-.2cm}
%     \caption{Comparing unrepaired and repaired MLPs on New \texttt{Adult} \citep{ding2021retiring}, Public Coverage.} 
%     \label{fig:app:public_mlp}
%     \vspace{-.2cm}
% \end{figure*}

\begin{figure*}[!ht]
    \centering
    \begin{minipage}{.33\textwidth}
        \centering
        \includegraphics[width=0.9\linewidth]{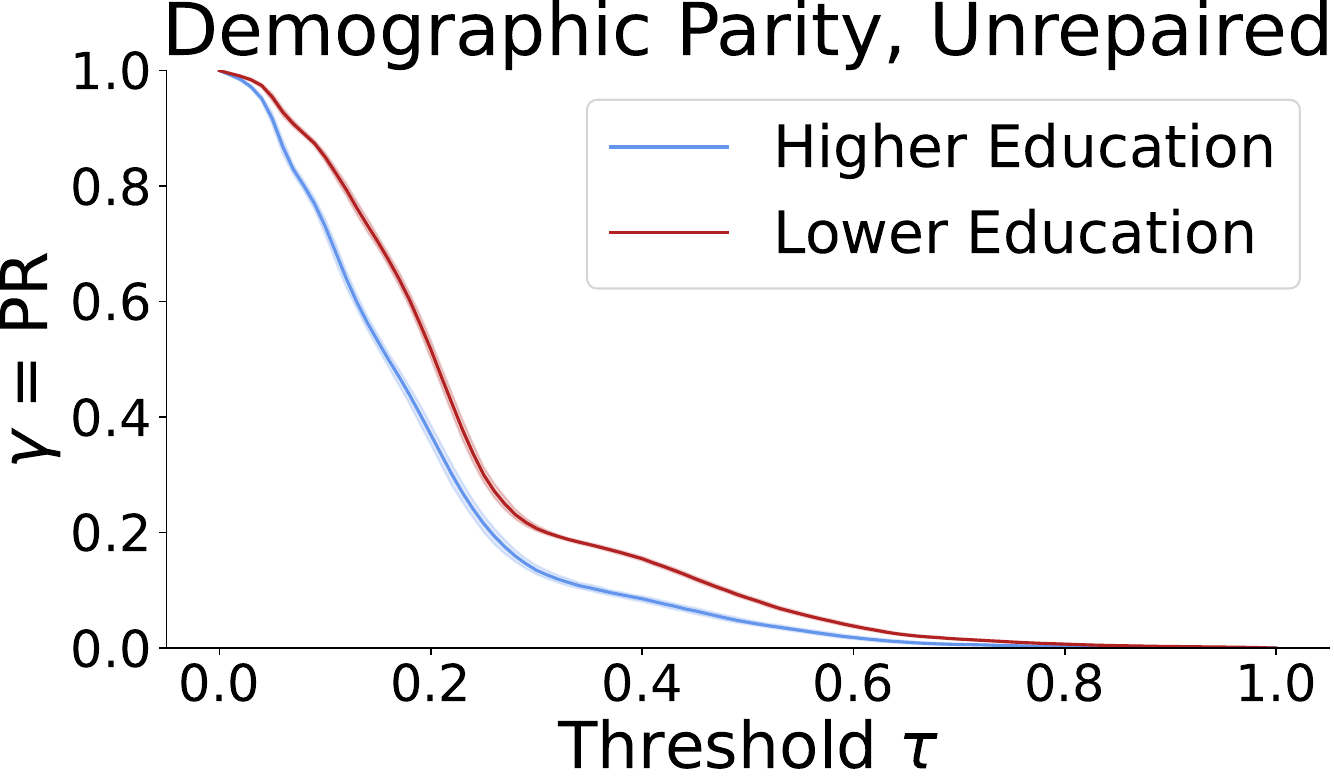}\\
        \includegraphics[width=0.9\linewidth]{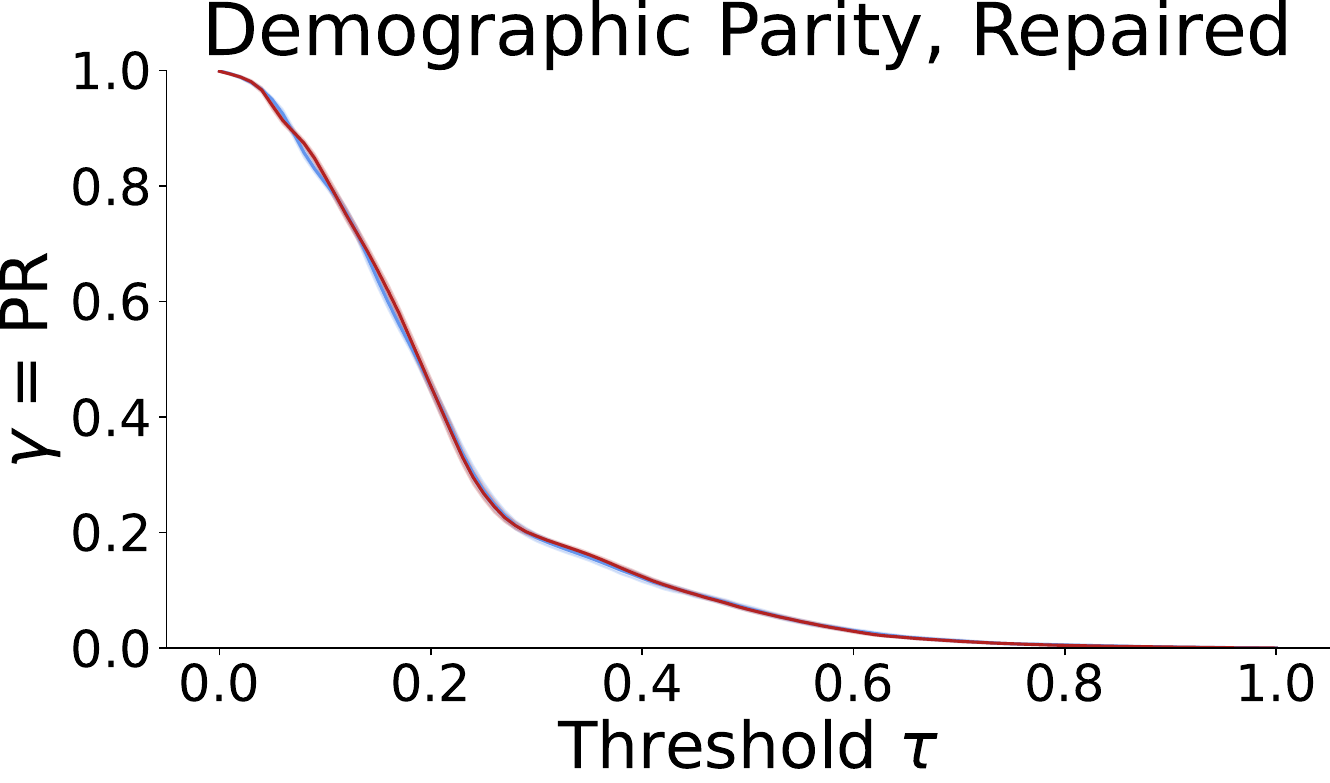}
        \subcaption{Algorithm~\ref{alg:repair} results for SDP}
        \label{fig:app:taiwan_lr-sdp}
    \end{minipage}%
    \begin{minipage}{0.66\textwidth}
        \centering
        \includegraphics[width=0.45\linewidth]{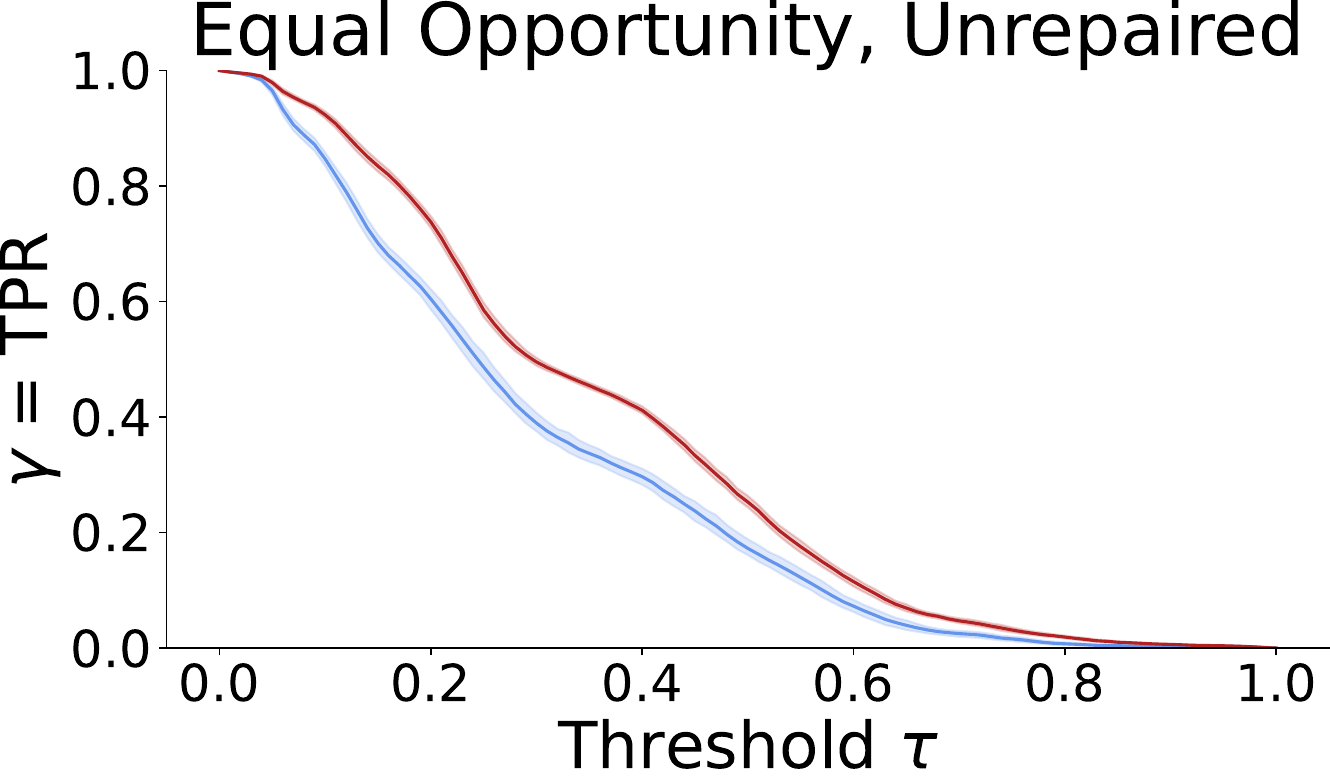}
        \includegraphics[width=0.45\linewidth]{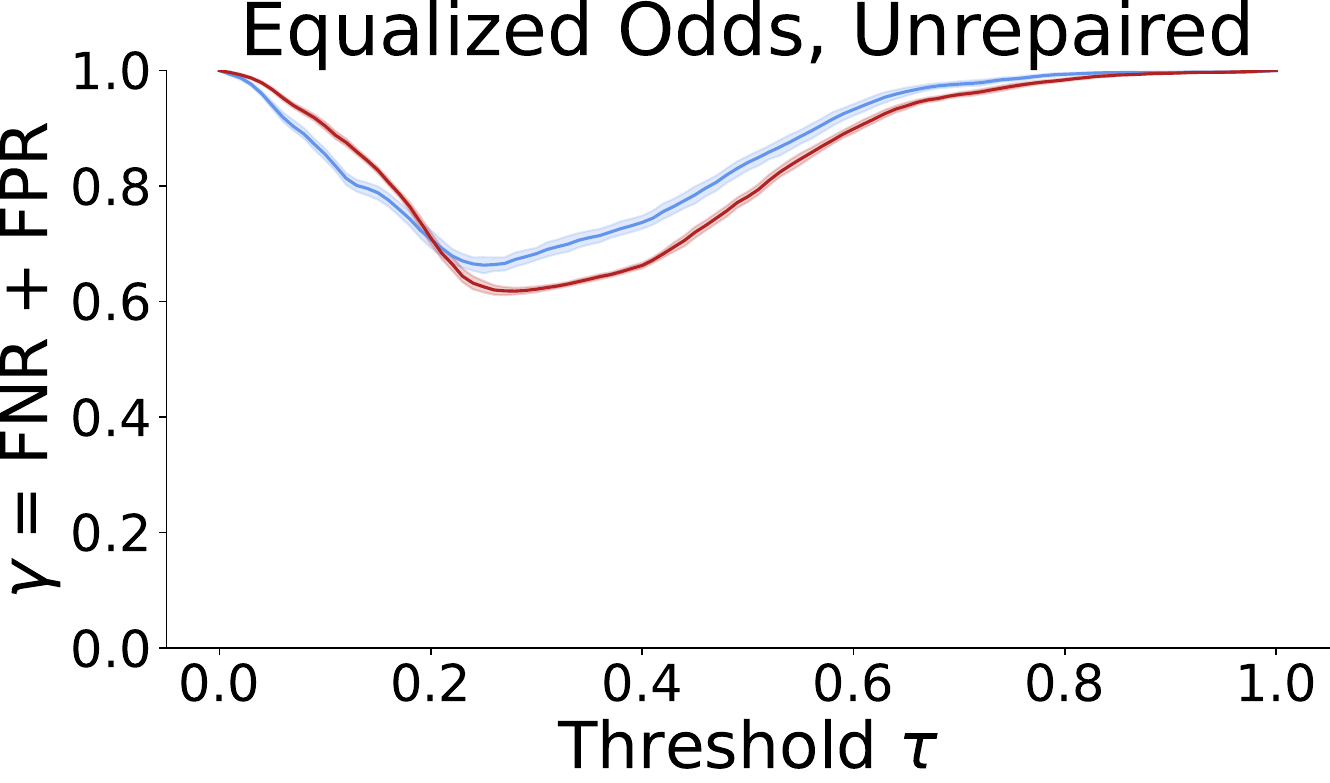}\\
        \includegraphics[width=0.45\linewidth]{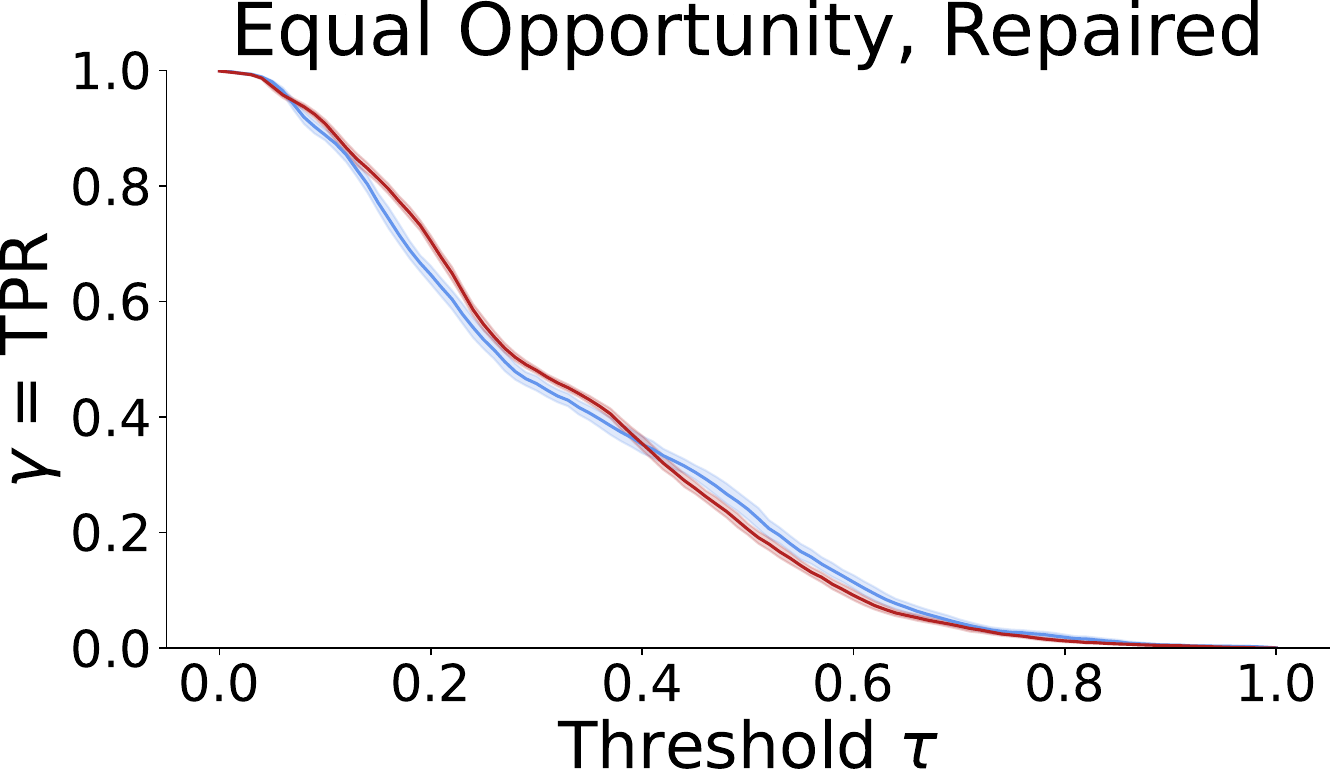}
        \includegraphics[width=0.45\linewidth]{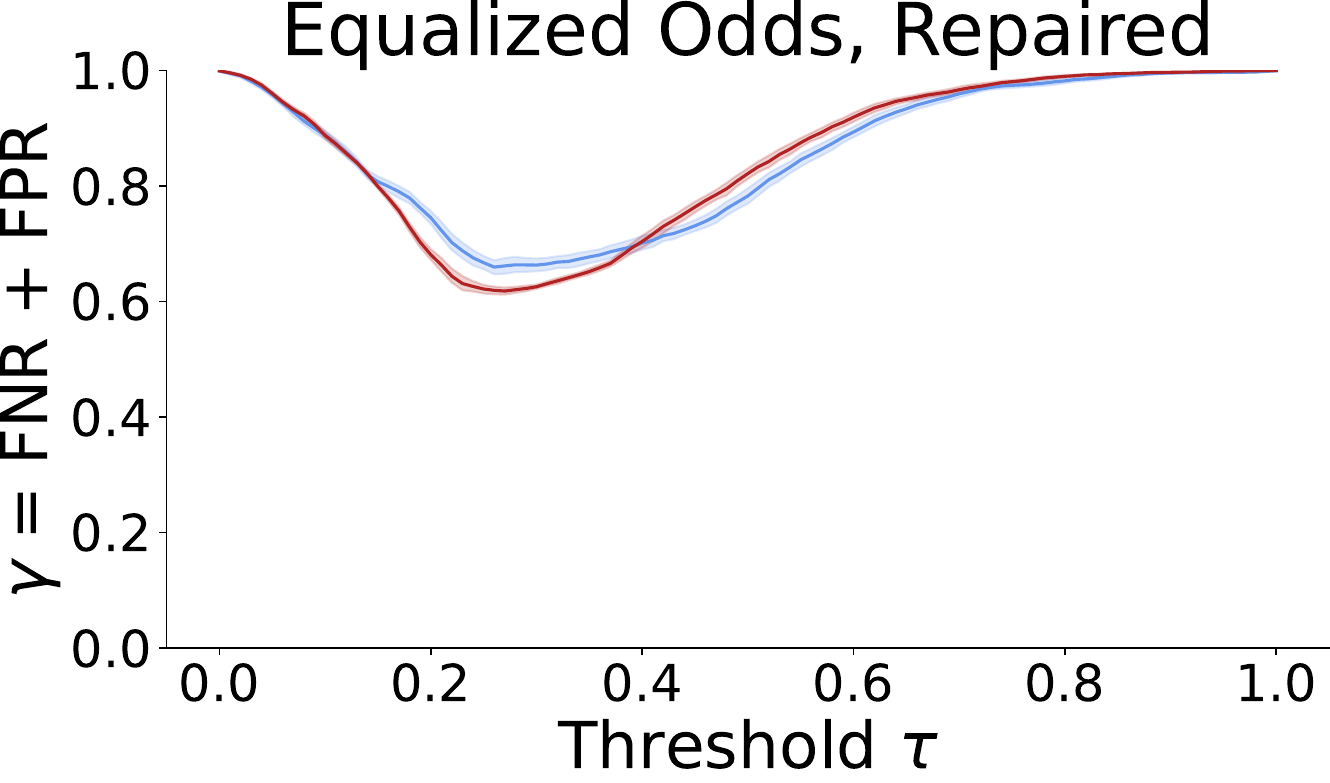}\\
        \subcaption{Algorithm~\ref{alg:repair} results for Eq. Odds and Eq. Opportunity}
        \label{fig:app:taiwan_lr-ours}
    \end{minipage}
    \vspace{-.2cm}
    \caption{Comparing unrepaired and repaired logistic regression on \texttt{Taiwan Credit} \citep{bay2000uci}.} 
    \label{fig:app:taiwan_lr}
    \vspace{-.2cm}
\end{figure*}

\begin{figure*}[!ht]
    \centering
    \begin{minipage}{.33\textwidth}
        \centering
        \includegraphics[width=0.9\linewidth]{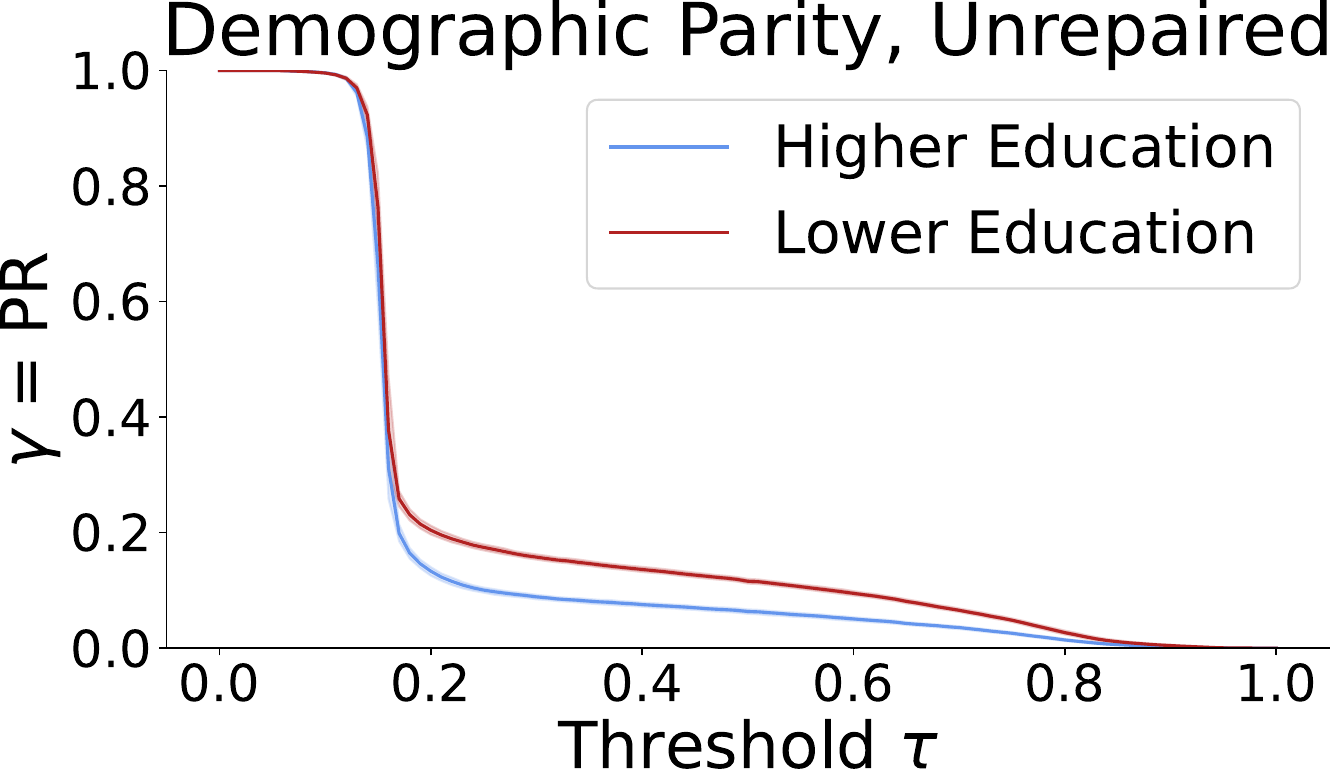}\\
        \includegraphics[width=0.9\linewidth]{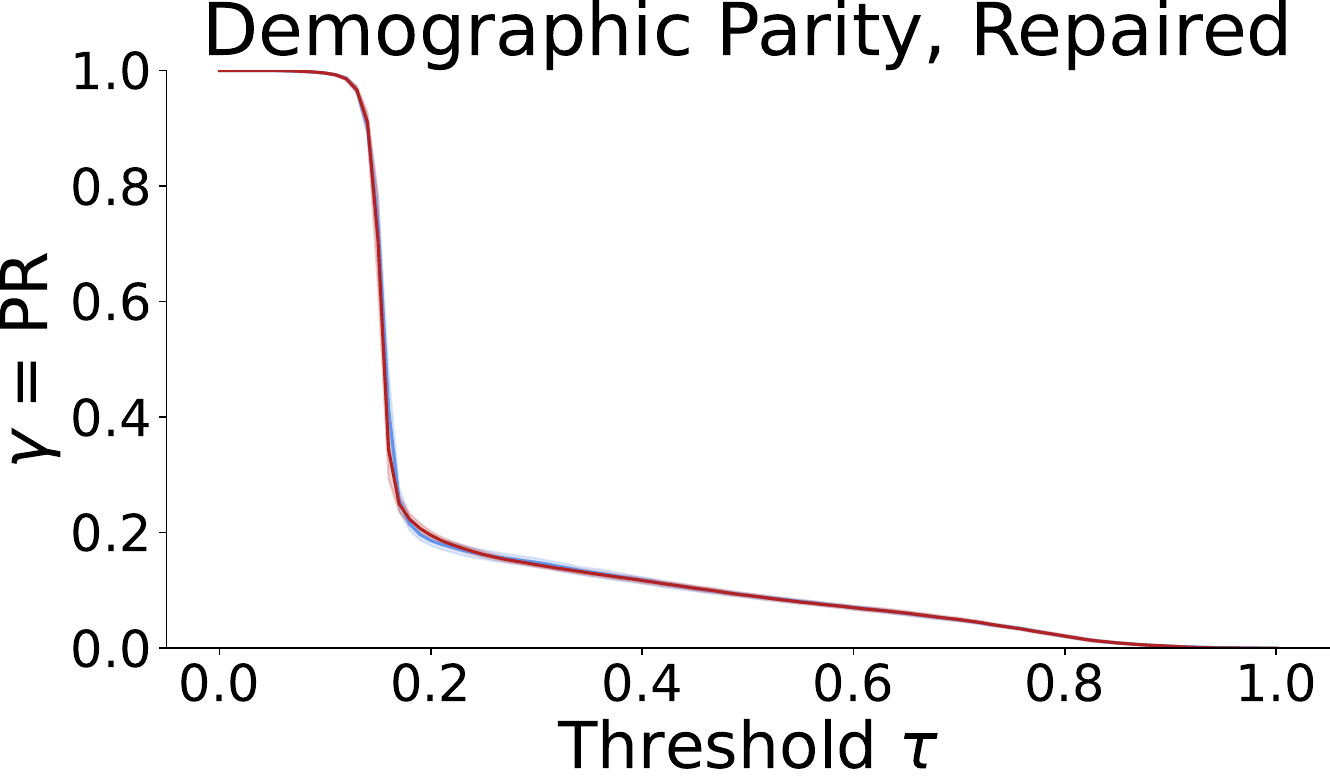}
        \subcaption{Algorithm~\ref{alg:repair} results for SDP}
        \label{fig:app:taiwan_svm-sdp}
    \end{minipage}%
    \begin{minipage}{0.66\textwidth}
        \centering
        \includegraphics[width=0.45\linewidth]{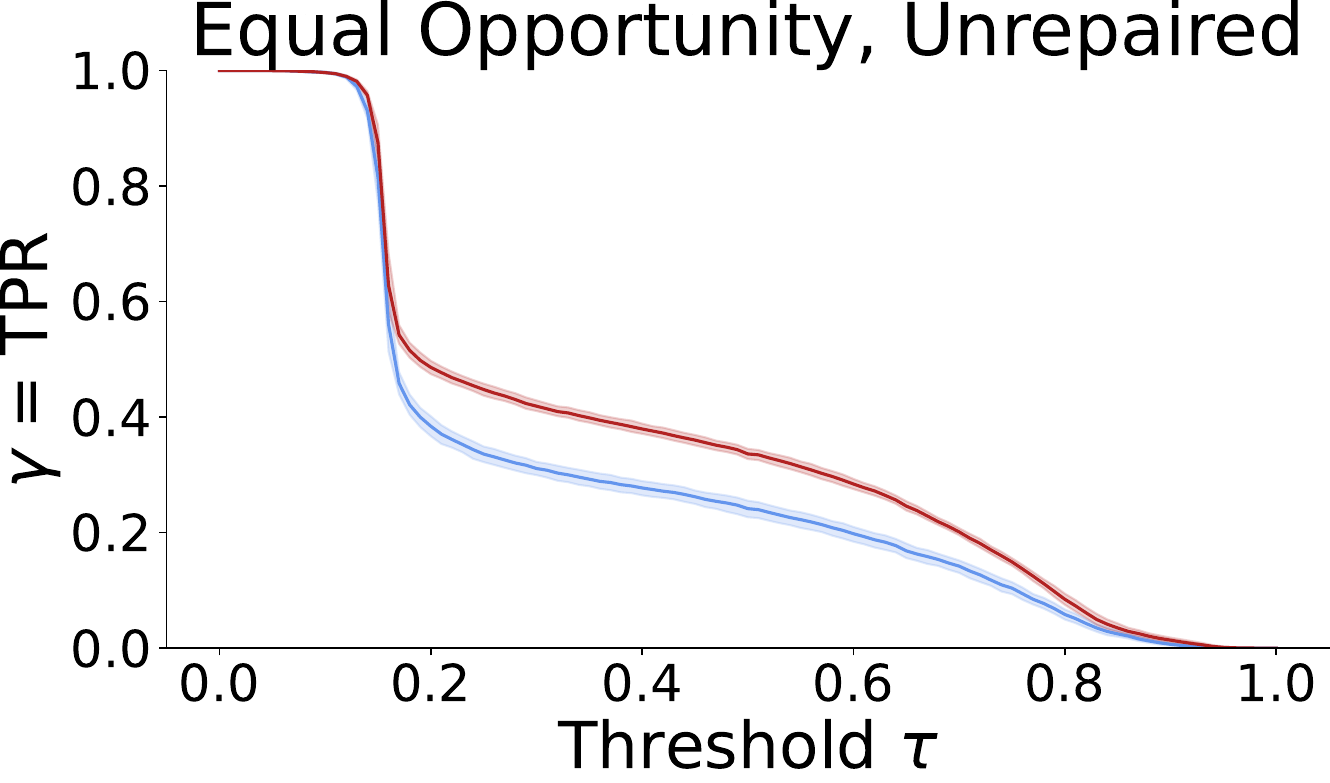}
        \includegraphics[width=0.45\linewidth]{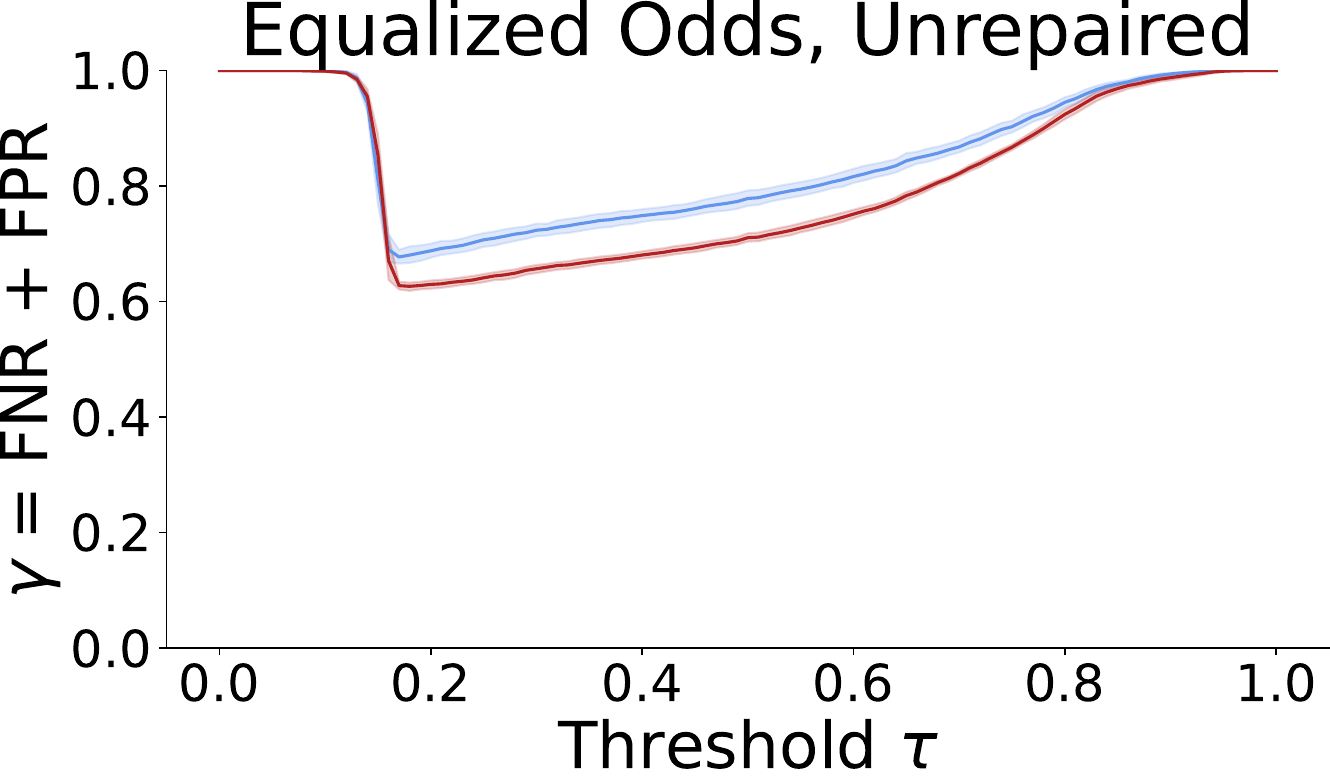}\\
        \includegraphics[width=0.45\linewidth]{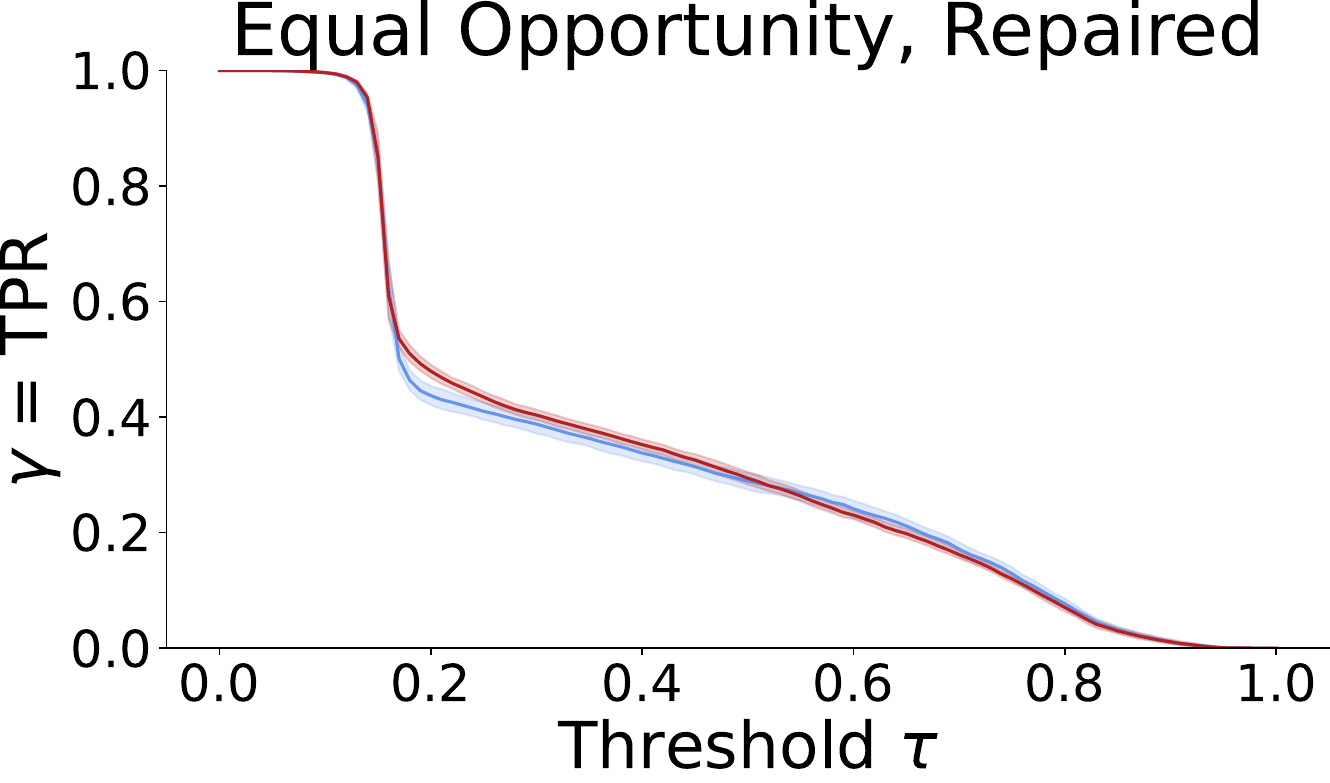}
        \includegraphics[width=0.45\linewidth]{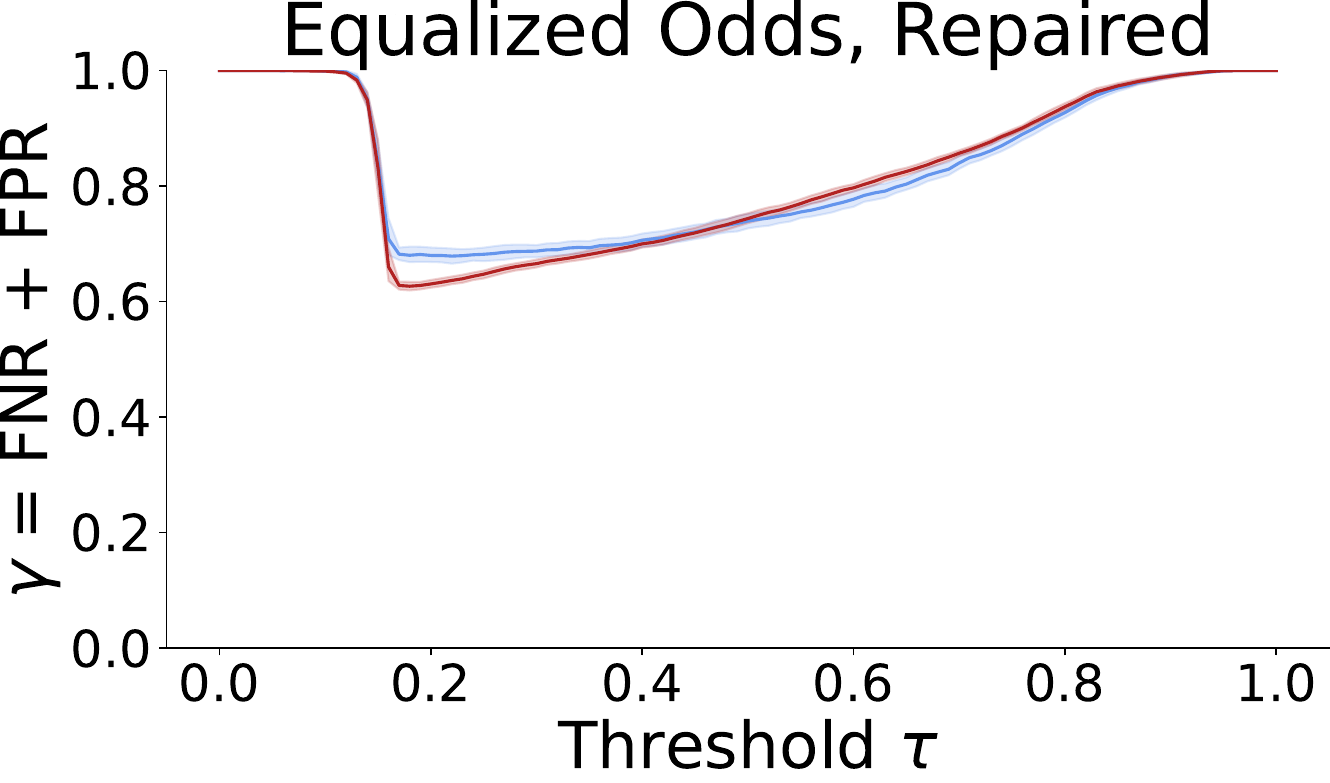}\\
        \subcaption{Algorithm~\ref{alg:repair} results for Eq. Odds and Eq. Opportunity}
        \label{fig:app:taiwan_svm-ours}
    \end{minipage}
    \vspace{-.2cm}
    \caption{Comparing unrepaired and repaired SVMs on \texttt{Taiwan Credit} \citep{bay2000uci}.} 
    \label{fig:app:taiwan_svm}
    \vspace{-.2cm}
\end{figure*}

\begin{figure*}[!ht]
    \centering
    \begin{minipage}{.33\textwidth}
        \centering
        \includegraphics[width=0.9\linewidth]{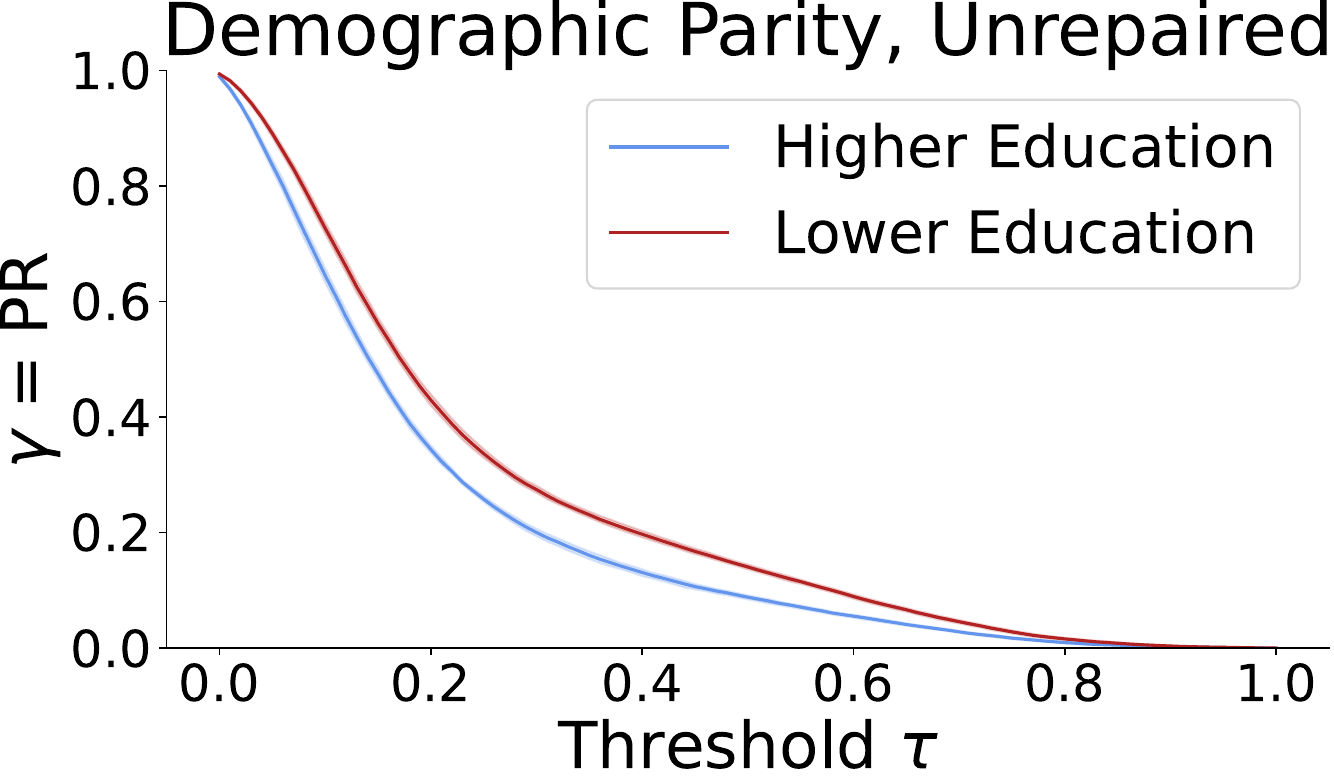}\\
        \includegraphics[width=0.9\linewidth]{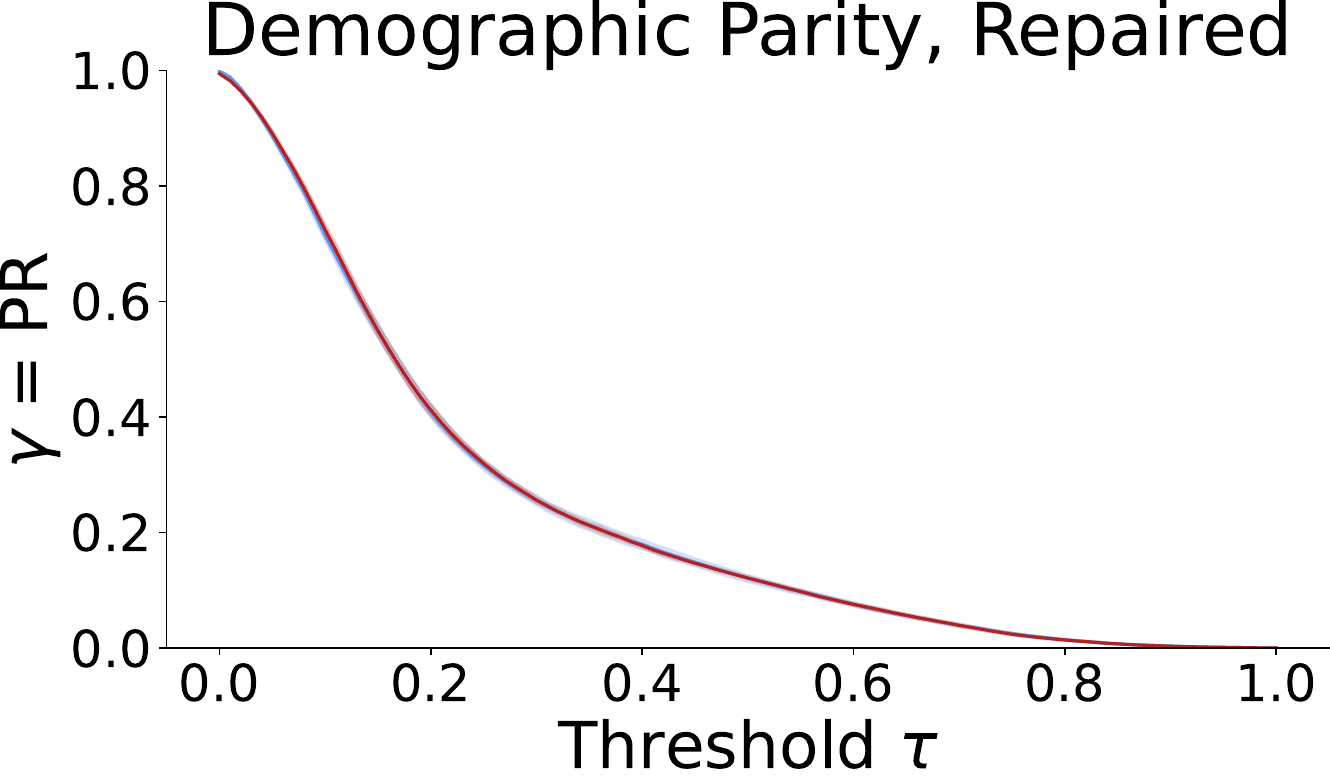}
        \subcaption{Algorithm~\ref{alg:repair} results for SDP}
        \label{fig:app:taiwan_rf-sdp}
    \end{minipage}%
    \begin{minipage}{0.66\textwidth}
        \centering
        \includegraphics[width=0.45\linewidth]{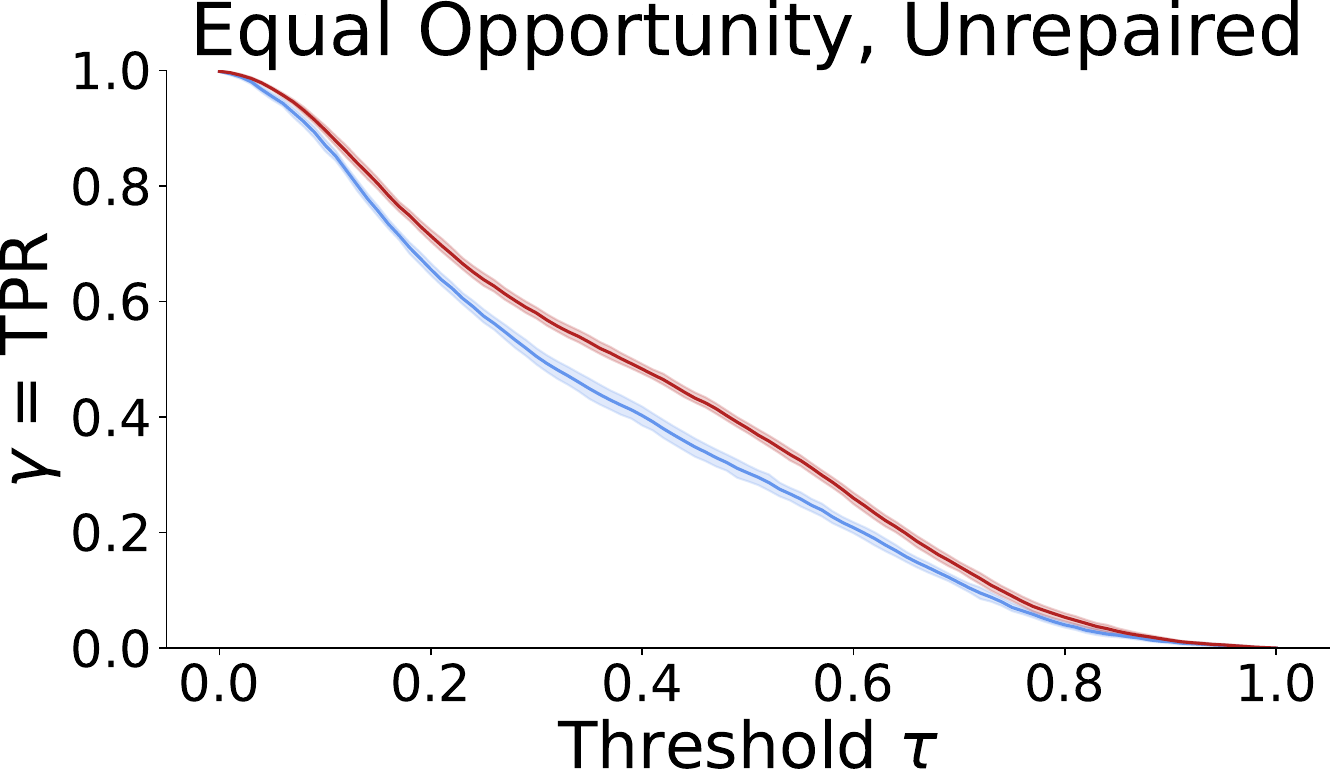}
        \includegraphics[width=0.45\linewidth]{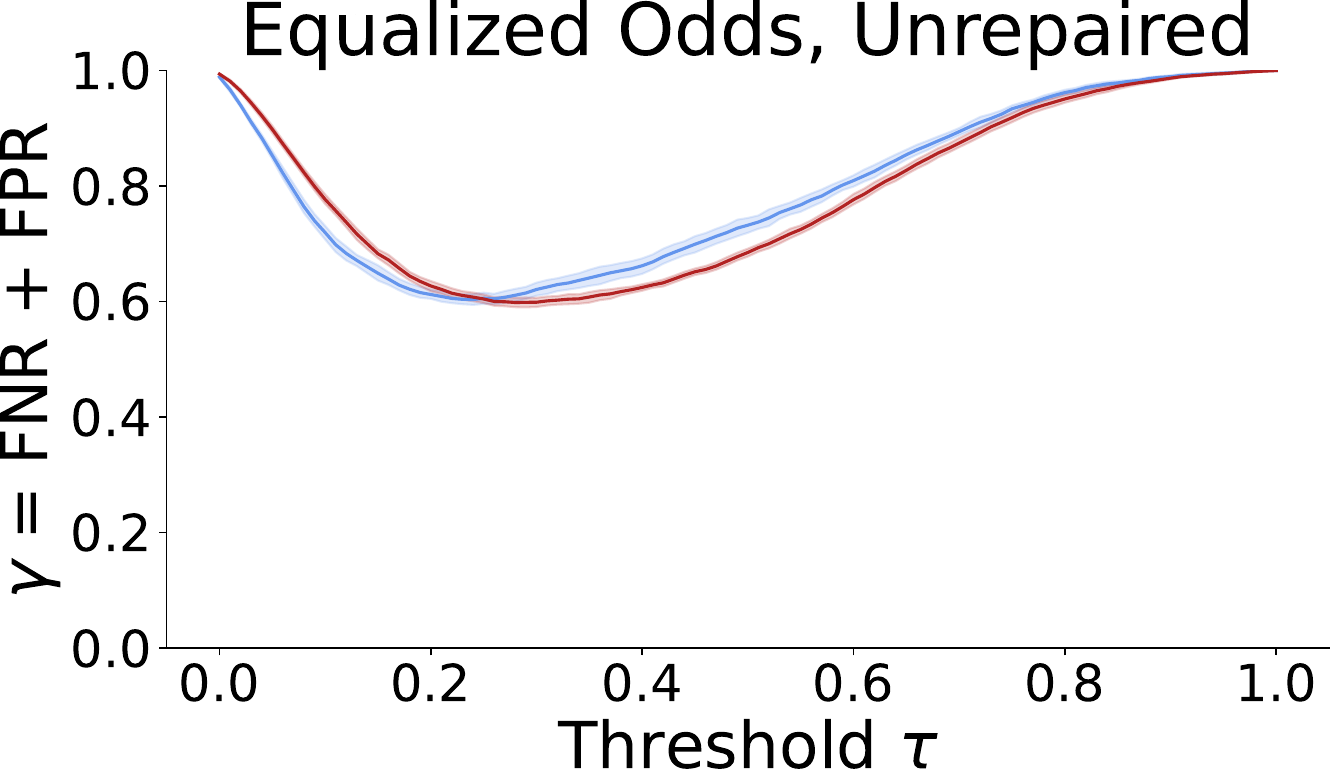}\\
        \includegraphics[width=0.45\linewidth]{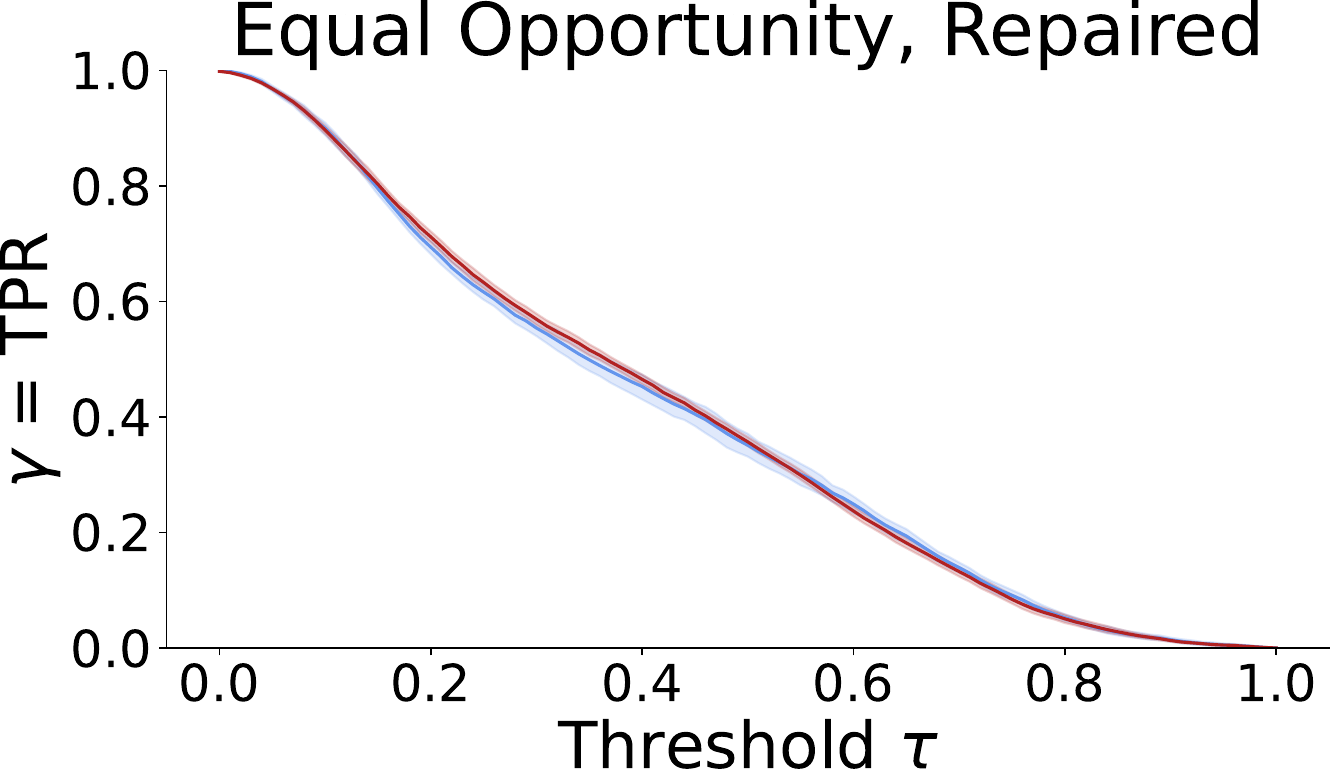}
        \includegraphics[width=0.45\linewidth]{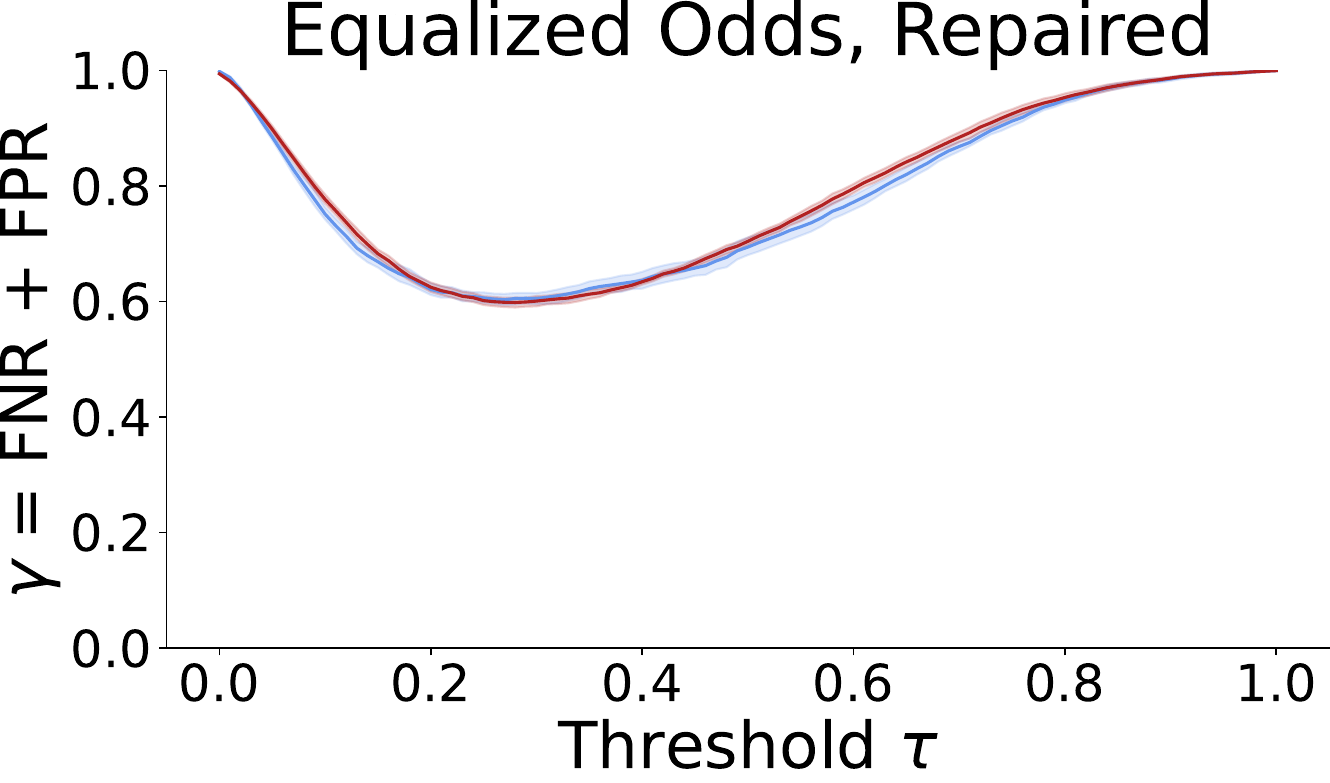}\\
        \subcaption{Algorithm~\ref{alg:repair} results for Eq. Odds and Eq. Opportunity}
        \label{fig:app:taiwan_rf-ours}
    \end{minipage}
    \vspace{-.2cm}
    \caption{Comparing unrepaired and repaired Random Forests on \texttt{Taiwan Credit} \citep{bay2000uci}.} 
    \label{fig:app:taiwan_rf}
    \vspace{-.2cm}
\end{figure*}

\begin{figure*}[!ht]
    \centering
    \begin{minipage}{.33\textwidth}
        \centering
        \includegraphics[width=0.9\linewidth]{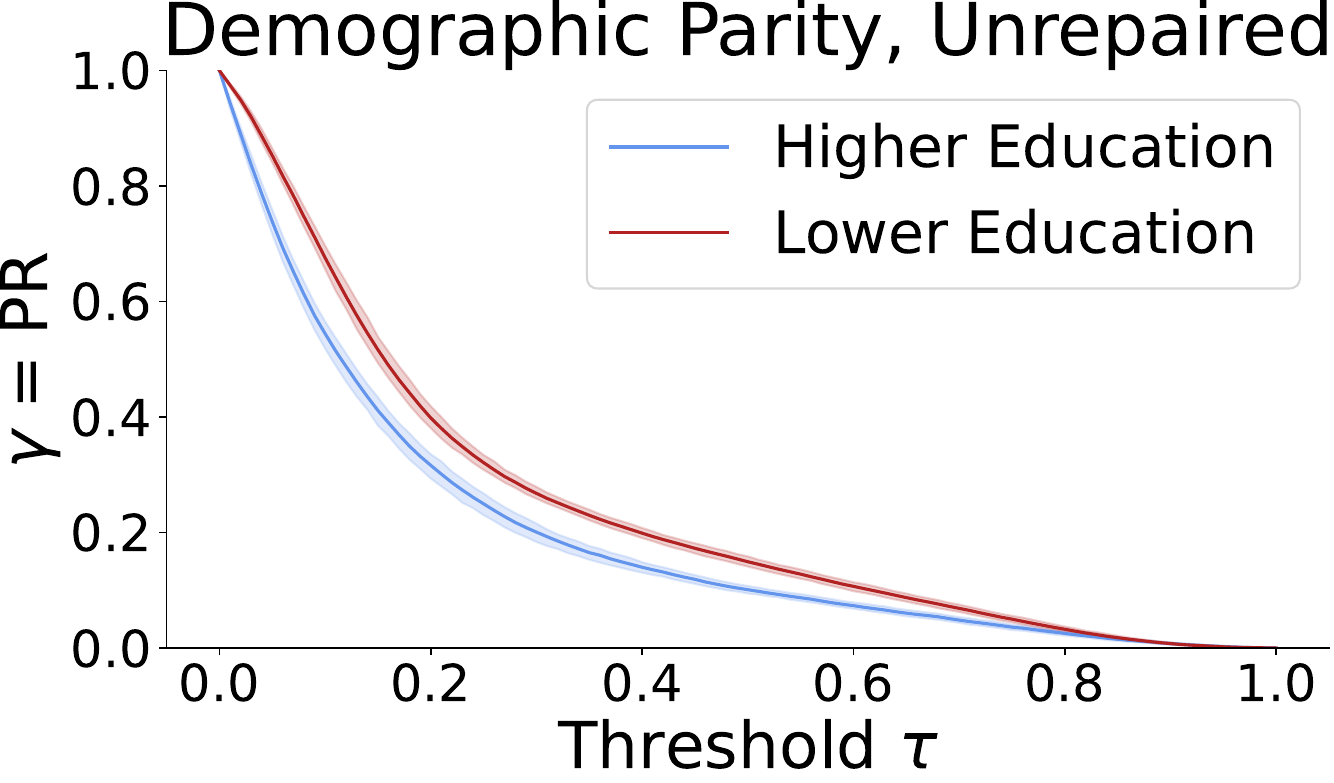}\\
        \includegraphics[width=0.9\linewidth]{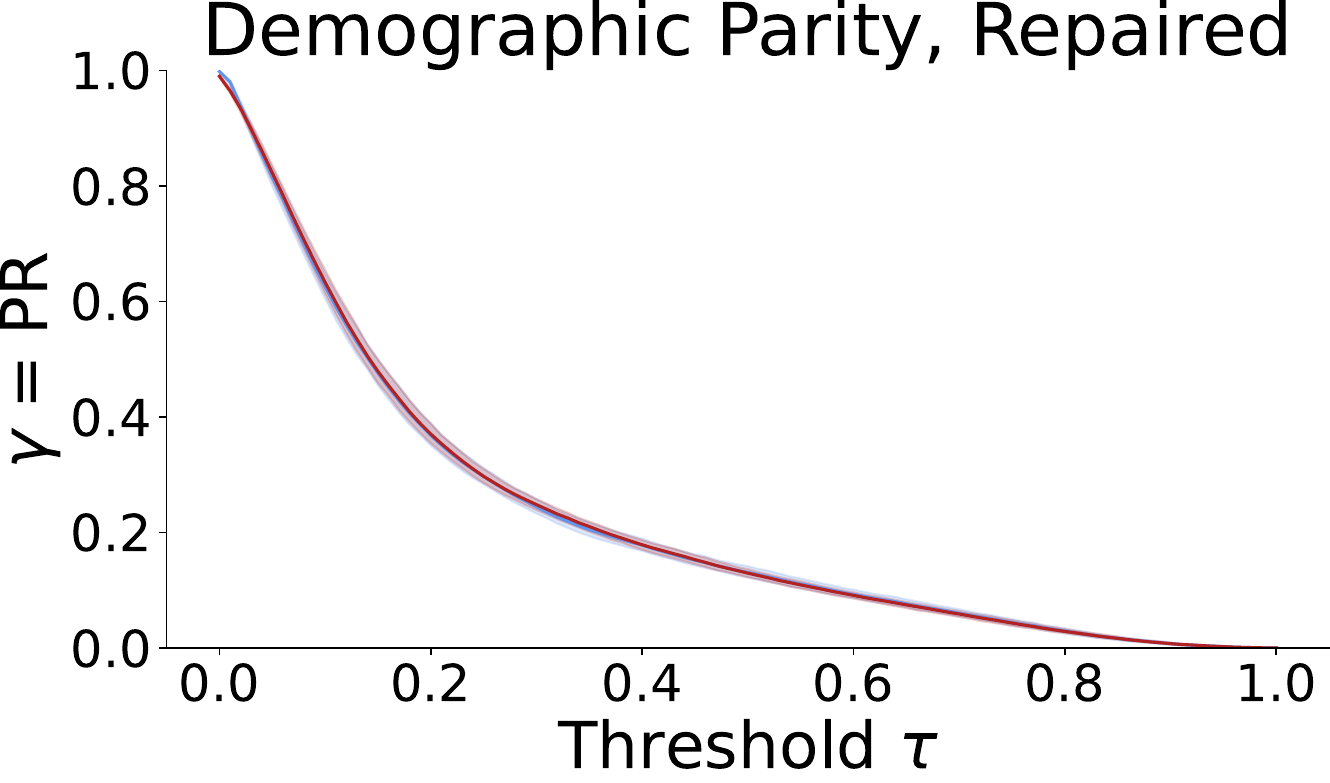}
        \subcaption{Algorithm~\ref{alg:repair} results for SDP}
        \label{fig:app:taiwan_mlp-sdp}
    \end{minipage}%
    \begin{minipage}{0.66\textwidth}
        \centering
        \includegraphics[width=0.45\linewidth]{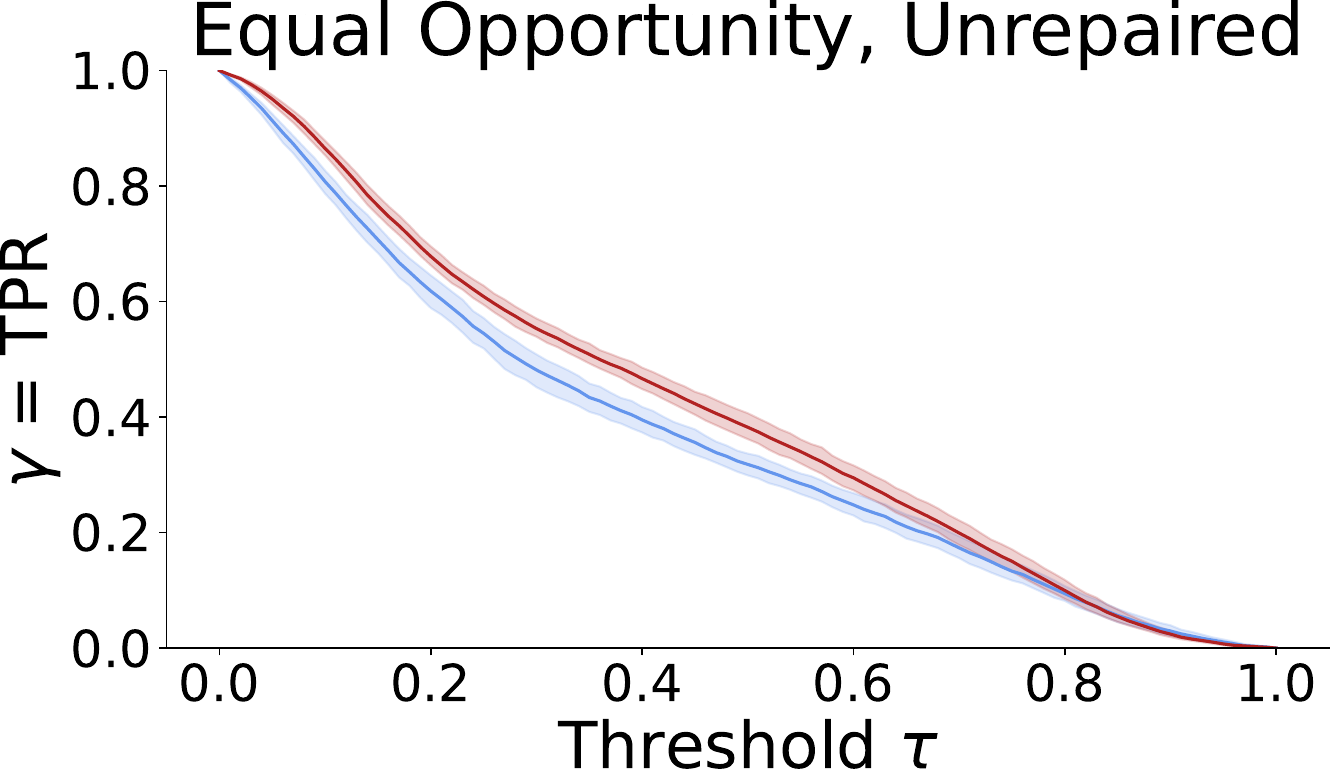}
        \includegraphics[width=0.45\linewidth]{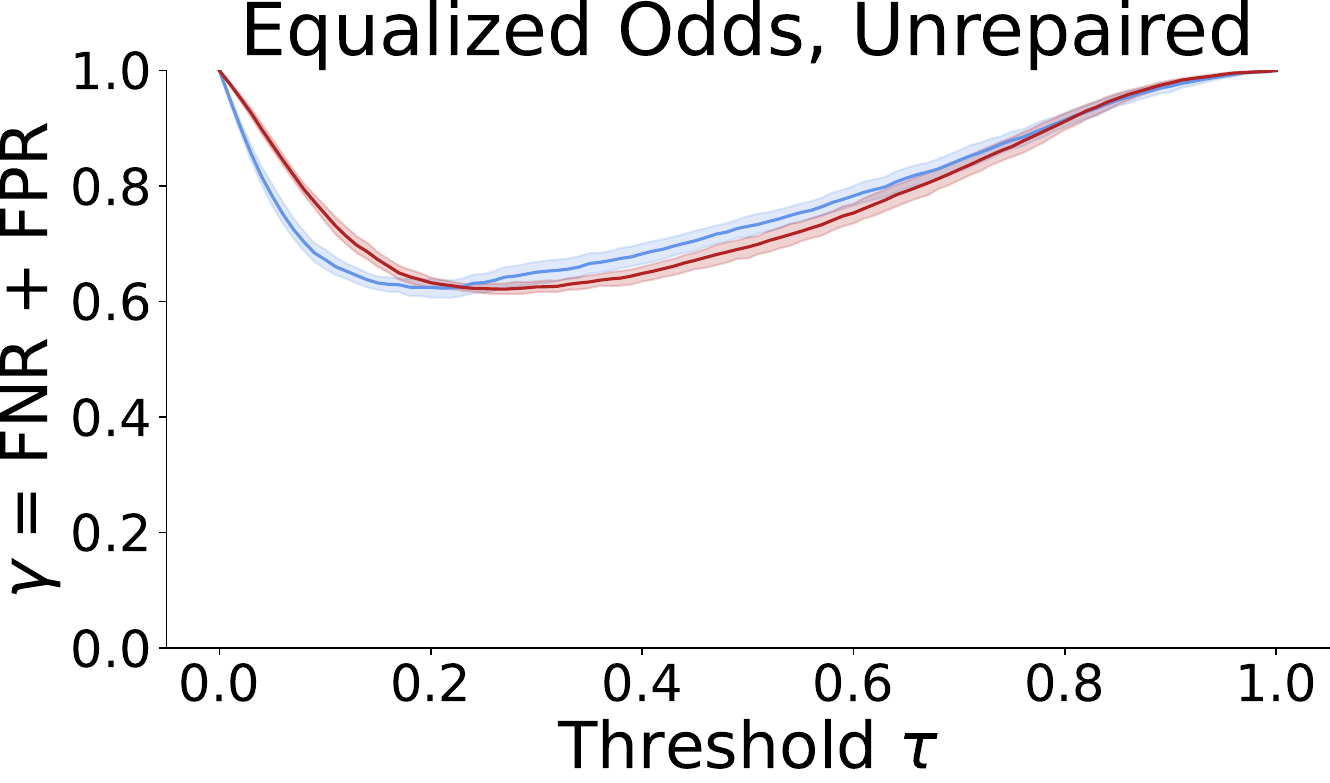}\\
        \includegraphics[width=0.45\linewidth]{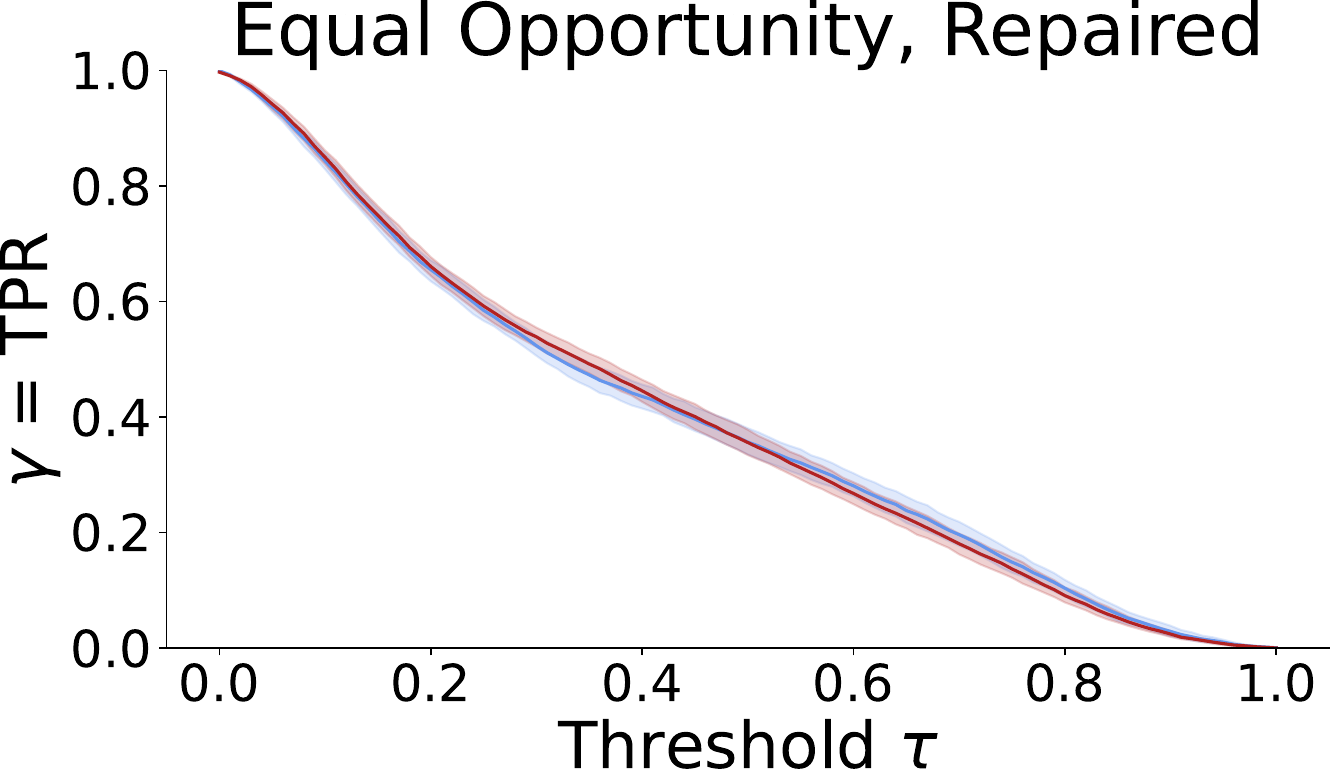}
        \includegraphics[width=0.45\linewidth]{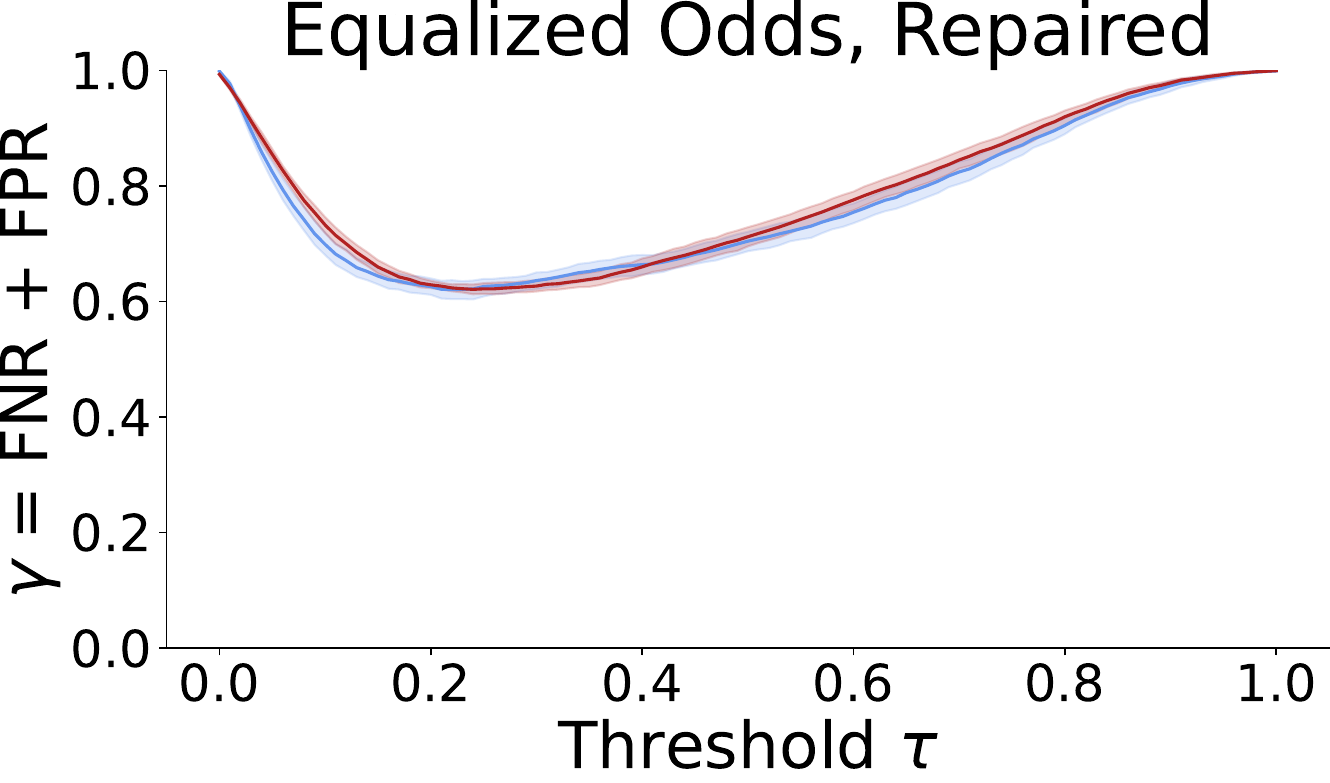}\\
        \subcaption{Algorithm~\ref{alg:repair} results for Eq. Odds and Eq. Opportunity}
        \label{fig:app:taiwan_mlp-ours}
    \end{minipage}
    \vspace{-.2cm}
    \caption{Comparing unrepaired and repaired MLPs on \texttt{Taiwan Credit} \citep{bay2000uci}.} 
    \label{fig:app:taiwan_mlp}
    \vspace{-.2cm}
\end{figure*}
